# Supplementary material for: The Power of Unbiased Recursive Partitioning: A Unifying View of CTree, MOB, and GUIDE
Source: arXiv:1906.10179 ancillary file (2019-06-24)
Supplement: Supplementary file 1 [file constparty.pdf]

# Constant Partying: Growing and Handling Trees with Constant Fits

Torsten Hothorn  
Universität Zürich

Achim Zeileis  
Universität Innsbruck

---

## Abstract

This vignette describes infrastructure for regression and classification trees with simple constant fits in each of the terminal nodes. Thus, all observations that are predicted to be in the same terminal node also receive the same prediction, e.g., a mean for numeric responses or proportions for categorical responses. This class of trees is very common and includes all traditional tree variants (AID, CHAID, CART, C4.5, FACT, QUEST) and also more recent approaches like CTree. Trees inferred by any of these algorithms could in principle be represented by objects of class “`constparty`” in **partykit** that then provides unified methods for printing, plotting, and predicting. Here, we describe how one can create “`constparty`” objects by (a) coercion from other R classes, (b) parsing of XML descriptions of trees learned in other software systems, (c) learning a tree using one’s own algorithm.

*Keywords:* recursive partitioning, regression trees, classification trees, decision trees.

---

## 1. Classes and methods

This vignette describes the handling of trees with constant fits in the terminal nodes. This class of regression models includes most classical tree algorithms like AID (Morgan and Sonquist 1963), CHAID (Kass 1980), CART (Breiman, Friedman, Olshen, and Stone 1984), FACT (Loh and Vanichsetakul 1988), QUEST (Loh and Shih 1997), C4.5 (Quinlan 1993), CTree (Hothorn, Hornik, and Zeileis 2006) etc. In this class of tree models, one can compute simple predictions for new observations, such as the conditional mean in a regression setup, from the responses of those learning sample observations in the same terminal node. Therefore, such predictions can easily be computed if the following pieces of information are available: the observed responses in the learning sample, the terminal node IDs assigned to the observations in the learning sample, and potentially associated weights (if any).

In **partykit** it is easy to create a “`party`” object that contains these pieces of information, yielding a “`constparty`” object. The technical details of the “`party`” class are discussed in detail in Section 3.4 of `vignette("partykit", package = "partykit")`. In addition to the elements required for any “`party`”, a “`constparty`” needs to have: `variables` (`fitted`) and `(response)` (and `(weights)` if applicable) in the `fitted` data frame along with the `terms` for the model. If such a “`party`” has been created, its properties can be checked and coerced to class “`constparty`” by the `as.constparty()` function.

Note that with such a “`constparty`” object it is possible to compute all kinds of predictions from the subsample in a given terminal node. For example, instead the mean response the

median (or any other quantile) could be employed. Similarly, for a categorical response the predicted probabilities (i.e., relative frequencies) can be computed or the corresponding mode or a ranking of the levels etc.

In case the full response from the learning sample is not available but only the constant fit from each terminal node, then a “`constparty`” cannot be set up. Specifically, this is the case for trees saved in the XML format PMML (Predictive Model Markup Language, [Data Mining Group 2014](#)) that does not provide the full learning sample. To also support such constant-fit trees based on simpler information `partykit` provides the “`simpleparty`” class. Inspired by the PMML format, this requires that the `info` of every node in the tree provides list elements `prediction`, `n`, `error`, and `distribution`. For classification trees these should contain the following node-specific information: the predicted single predicted factor, the learning sample size, the misclassification error (in %), and the absolute frequencies of all levels. For regression trees the contents should be: the predicted mean, the learning sample size, the error sum of squares, and `NULL`. The function `as.simpleparty()` can also coerce “`constparty`” trees to “`simpleparty`” trees by computing the above summary statistics from the full response associated with each node of the tree.

The remainder of this vignette consists of the following parts: In Section 2 we assume that the trees were fitted using some other software (either within or outside of R) and we describe how these models can be coerced to “`party`” objects using either the “`constparty`” or “`simpleparty`” class. Emphasize is given to displaying such trees in textual and graphical ways. Subsequently, in Section 3, we show a simple classification tree algorithm can be easily implemented using the `partykit` tools, yielding a “`constparty`” object. Section 4 shows how to compute predictions in both scenarios before Section 5 finally gives a brief conclusion.

## 2. Coercing tree objects

For the illustrations, we use the Titanic data set from package `datasets`, consisting of four variables on each of the 2201 Titanic passengers: gender (male, female), age (child, adult), and class (1st, 2nd, 3rd, or crew) set up as follows:

```
> data("Titanic", package = "datasets")
> ttnc <- as.data.frame(Titanic)
> ttnc <- ttnc[rep(1:nrow(ttnc), ttnc$Freq), 1:4]
> names(ttnc)[2] <- "Gender"
```

The response variable describes whether or not the passenger survived the sinking of the ship.

### 2.1. Coercing rpart objects

We first fit a classification tree by means of the the `rpart()` function from package `rpart` ([Therneau and Atkinson 1997](#)) to this data set (make sure to set `model = TRUE`; otherwise `model.frame.rpart` will return the `rpart` object and not the data):

```
> library("rpart")
> (rp <- rpart(Survived ~ ., data = ttnc, model = TRUE))
```

n= 2201

```
node), split, n, loss, yval, (yprob)
  * denotes terminal node
```

```
1) root 2201 711 No (0.6769650 0.3230350)
  2) Gender=Male 1731 367 No (0.7879838 0.2120162)
    4) Age=Adult 1667 338 No (0.7972406 0.2027594) *
    5) Age=Child 64 29 No (0.5468750 0.4531250)
      10) Class=3rd 48 13 No (0.7291667 0.2708333) *
      11) Class=1st,2nd 16 0 Yes (0.0000000 1.0000000) *
  3) Gender=Female 470 126 Yes (0.2680851 0.7319149)
    6) Class=3rd 196 90 No (0.5408163 0.4591837) *
    7) Class=1st,2nd,Crew 274 20 Yes (0.0729927 0.9270073) *
```

The “`rpart`” object `rp` can be coerced to a “`constparty`” by `as.party()`. Internally, this transforms the tree structure of the “`rpart`” tree to a “`partynode`” and combines it with the associated learning sample as described in Section 1. All of this is done automatically by

```
> (party_rp <- as.party(rp))
```

Model formula:

```
Survived ~ Class + Gender + Age
```

Fitted party:

```
[1] root
| [2] Gender in Male
| | [3] Age in Adult: No (n = 1667, err = 20.3%)
| | [4] Age in Child
| | | [5] Class in 3rd: No (n = 48, err = 27.1%)
| | | [6] Class in 1st, 2nd: Yes (n = 16, err = 0.0%)
| [7] Gender in Female
| | [8] Class in 3rd: No (n = 196, err = 45.9%)
| | [9] Class in 1st, 2nd, Crew: Yes (n = 274, err = 7.3%)
```

```
Number of inner nodes: 4
```

```
Number of terminal nodes: 5
```

Now, instead of the print method for “`rpart`” objects the print method for `constparty` objects creates a textual display of the tree structure. In a similar way, the corresponding `plot()` method produces a graphical representation of this tree, see Figure 1.

By default, the `predict()` method for “`rpart`” objects computes conditional class probabilities. The same numbers are returned by the `predict()` method for `constparty` objects with `type = "prob"` argument (see Section 4 for more details):

```
> all.equal(predict(rp), predict(party_rp, type = "prob"),
+ check.attributes = FALSE)
```

```
[1] TRUE
```

```
> plot(rp)
> text(rp)
```

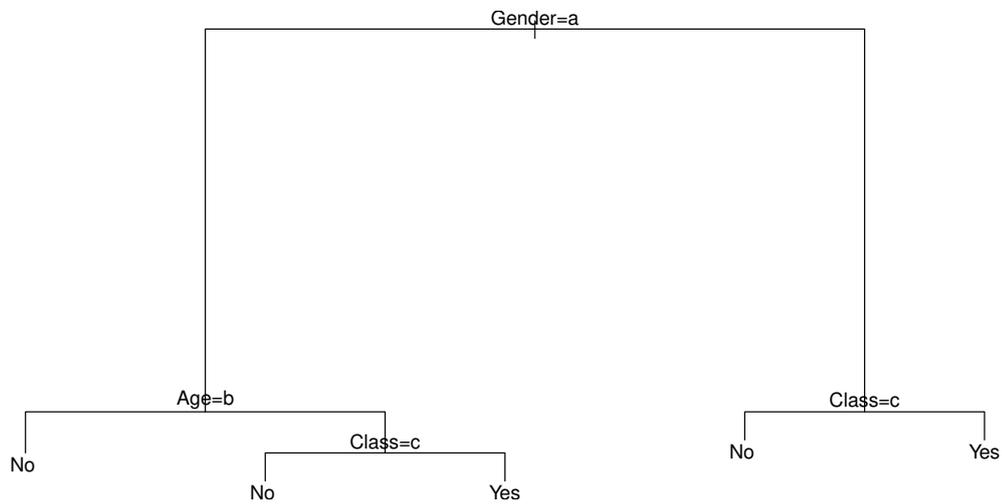

```
> plot(party_rp)
```

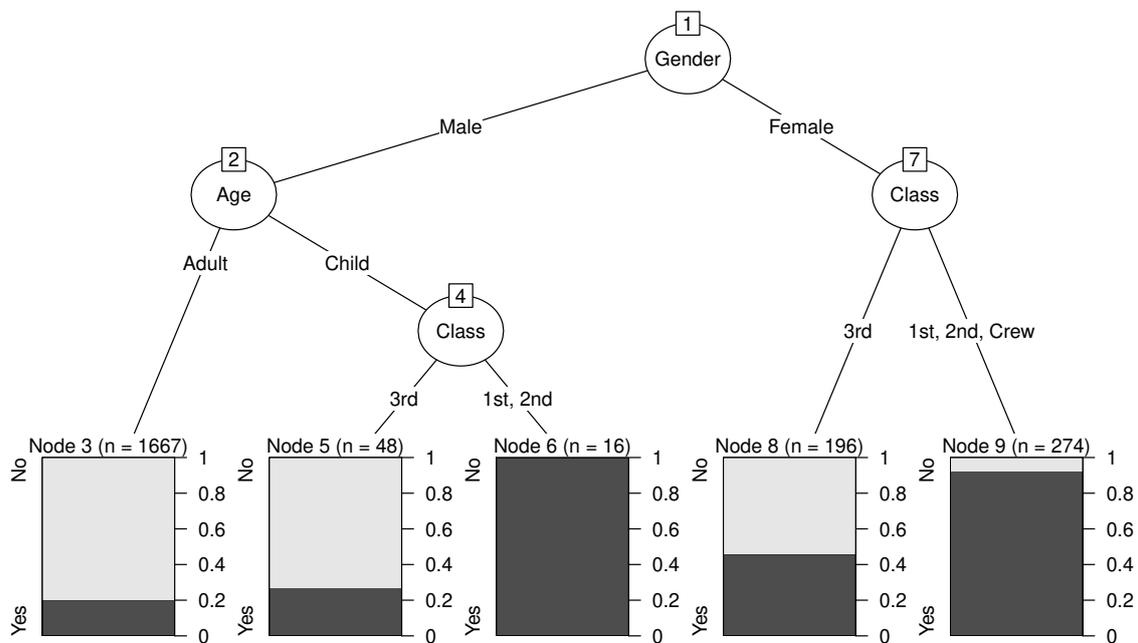

Figure 1: “**rpart**” tree of Titanic data plotted using **rpart** (top) and **partykit** (bottom) infrastructure.

Predictions are computed based on the `fitted` slot of a “`constparty`” object

```
> str(fitted(party_rp))
```

```
'data.frame':      2201 obs. of  2 variables:
 $ (fitted)  : int  5 5 5 5 5 5 5 5 5 5 ...
 $ (response): Factor w/ 2 levels "No","Yes": 1 1 1 1 1 1 1 1 1 1 ...
```

which contains the terminal node numbers and the response for each of the training samples. So, the conditional class probabilities for each terminal node can be computed via

```
> prop.table(do.call("table", fitted(party_rp)), 1)
```

```
      (response)
(fitted)      No      Yes
      3 0.7972406 0.2027594
      5 0.7291667 0.2708333
      6 0.0000000 1.0000000
      8 0.5408163 0.4591837
      9 0.0729927 0.9270073
```

Optionally, weights can be stored in the `fitted` slot as well.

## 2.2. Coercing J48 objects

The **RWeka** package (Hornik, Buchta, and Zeileis 2009) provides an interface to the **Weka** machine learning library and we can use the `J48()` function to fit a J4.8 tree to the Titanic data

```
> if (require("RWeka")) {
+   j48 <- J48(Survived ~ ., data = ttnc)
+ } else {
+   j48 <- rpart(Survived ~ ., data = ttnc)
+ }
> print(j48)
```

J48 pruned tree

-----

```
Gender = Male
|  Class = 1st
|  |  Age = Child: Yes (5.0)
|  |  Age = Adult: No (175.0/57.0)
|  Class = 2nd
|  |  Age = Child: Yes (11.0)
|  |  Age = Adult: No (168.0/14.0)
|  Class = 3rd: No (510.0/88.0)
```

```

|   Class = Crew: No (862.0/192.0)
Gender = Female
|   Class = 1st: Yes (145.0/4.0)
|   Class = 2nd: Yes (106.0/13.0)
|   Class = 3rd: No (196.0/90.0)
|   Class = Crew: Yes (23.0/3.0)

```

```
Number of Leaves :      10
```

```
Size of the tree :      15
```

This object can be coerced to a “party” object using

```
> (party_j48 <- as.party(j48))
```

Model formula:

```
Survived ~ Class + Gender + Age
```

Fitted party:

```

[1] root
|   [2] Gender in Male
|   |   [3] Class in 1st
|   |   |   [4] Age in Child: Yes (n = 5, err = 0.0%)
|   |   |   [5] Age in Adult: No (n = 175, err = 32.6%)
|   |   [6] Class in 2nd
|   |   |   [7] Age in Child: Yes (n = 11, err = 0.0%)
|   |   |   [8] Age in Adult: No (n = 168, err = 8.3%)
|   |   [9] Class in 3rd: No (n = 510, err = 17.3%)
|   |  [10] Class in Crew: No (n = 862, err = 22.3%)
|  [11] Gender in Female
|   |  [12] Class in 1st: Yes (n = 145, err = 2.8%)
|   |  [13] Class in 2nd: Yes (n = 106, err = 12.3%)
|   |  [14] Class in 3rd: No (n = 196, err = 45.9%)
|   |  [15] Class in Crew: Yes (n = 23, err = 13.0%)

```

```
Number of inner nodes:      5
```

```
Number of terminal nodes: 10
```

and, again, the print method from the **partykit** package creates a textual display. Note that, unlike the “**rpart**” trees, this tree includes multiway splits. The `plot()` method draws this tree, see Figure 2.

The conditional class probabilities computed by the `predict()` methods implemented in packages **RWeka** and **partykit** are equivalent:

```

> all.equal(predict(j48, type = "prob"), predict(party_j48, type = "prob"),
+   check.attributes = FALSE)

```

```
> plot(party_j48)
```

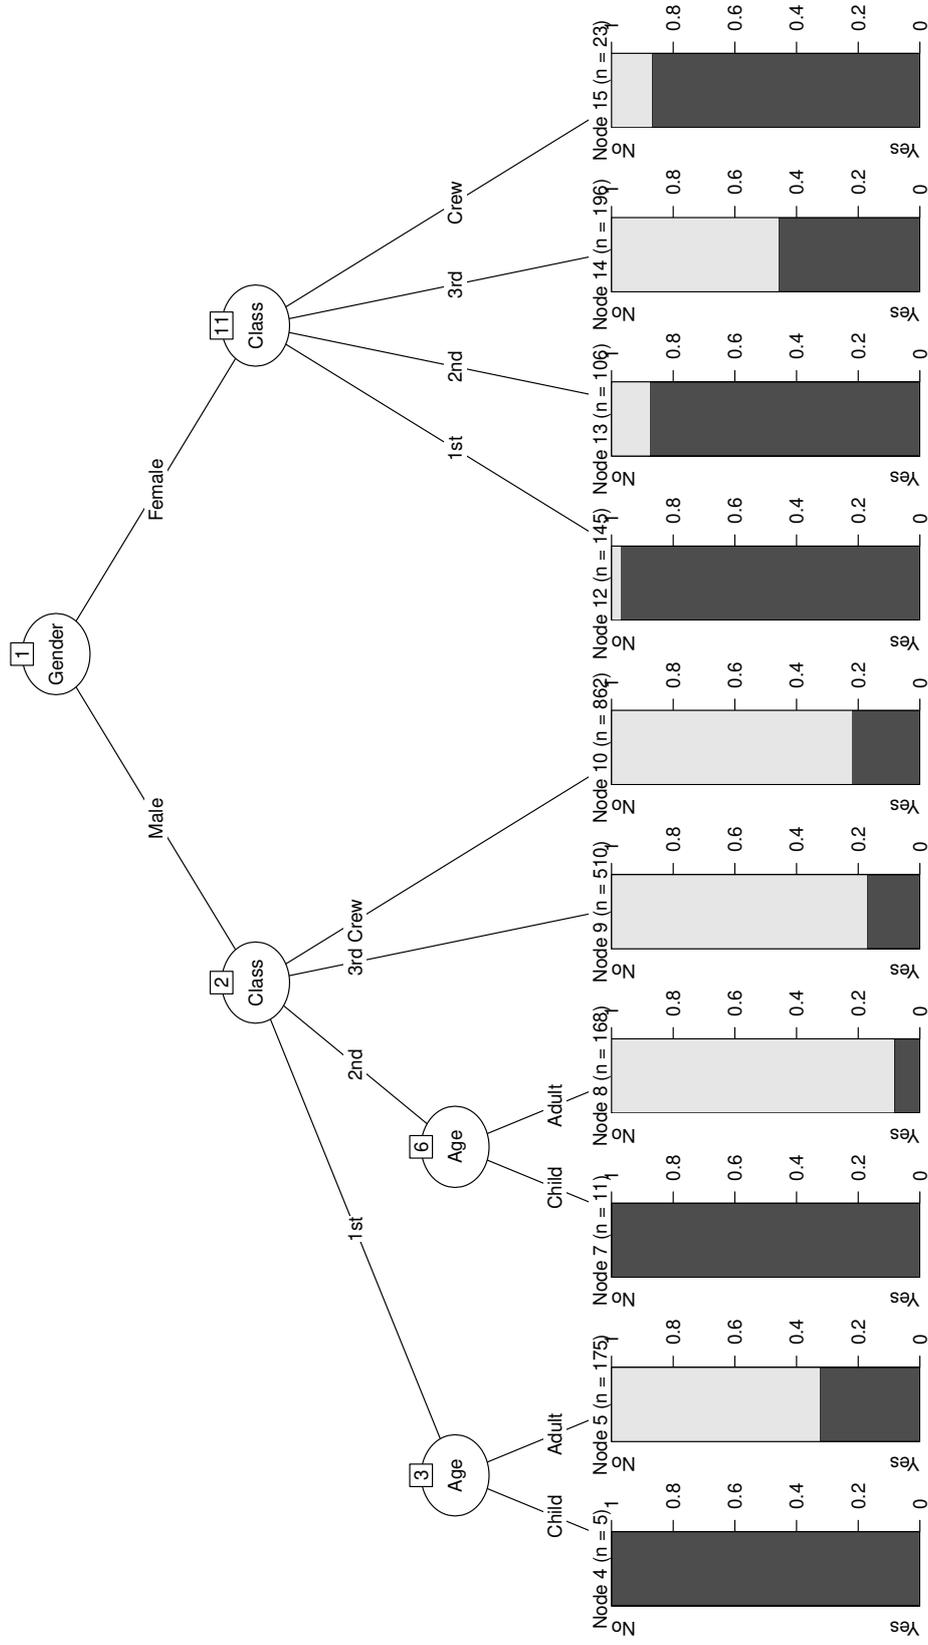

Figure 2: "J48" tree of Titanic data plotted using **partykit** infrastructure.

```
[1] TRUE
```

In addition to `J48()` **RWeka** provides several other tree learners, e.g., `M5P()` implementing M5' and `LMT()` implementing logistic model trees, respectively. These can also be coerced using `as.party()`. However, as these are not constant-fit trees this yields plain “**party**” trees with some character information stored in the `info` slot.

### 2.3. Importing trees from PMML files

The previous two examples showed how trees learned by other R packages can be handled in a unified way using **partykit**. Additionally, **partykit** can also be used to import trees from any other software package that supports the PMML (Predictive Model Markup Language) format.

As an example, we used SPSS to fit a QUEST tree to the Titanic data and exported this from SPSS in PMML format. This file is shipped along with the **partykit** package and we can read it as follows:

```
> ttnc_pmml <- file.path(system.file("pmml", package = "partykit"),
+ "ttnc.pmml")
> (ttnc_quest <- pmmlTreeModel(ttnc_pmml))
```

Model formula:

```
Survived ~ Gender + Class + Age
```

Fitted party:

```
[1] root
| [2] Gender in Female
| | [3] Class in 3rd, Crew: Yes (n = 219, err = 49.8%)
| | [4] Class in 1st, 2nd
| | | [5] Class in 2nd: Yes (n = 106, err = 12.3%)
| | | [6] Class in 1st: Yes (n = 145, err = 2.8%)
| [7] Gender in Male
| | [8] Class in 3rd, 2nd, Crew
| | | [9] Age in Child: No (n = 59, err = 40.7%)
| | | [10] Age in Adult
| | | | [11] Class in 3rd, Crew
| | | | | [12] Class in Crew: No (n = 862, err = 22.3%)
| | | | | [13] Class in 3rd: No (n = 462, err = 16.2%)
| | | | | [14] Class in 2nd: No (n = 168, err = 8.3%)
| | [15] Class in 1st: No (n = 180, err = 34.4%)
```

```
Number of inner nodes: 7
```

```
Number of terminal nodes: 8
```

The object `ttnc_quest` is of class “**simpleparty**” and the corresponding graphical display is shown in Figure 3. As explained in Section 1, the full learning data are not part of the PMML

```
> plot(ttnc_quest)
```

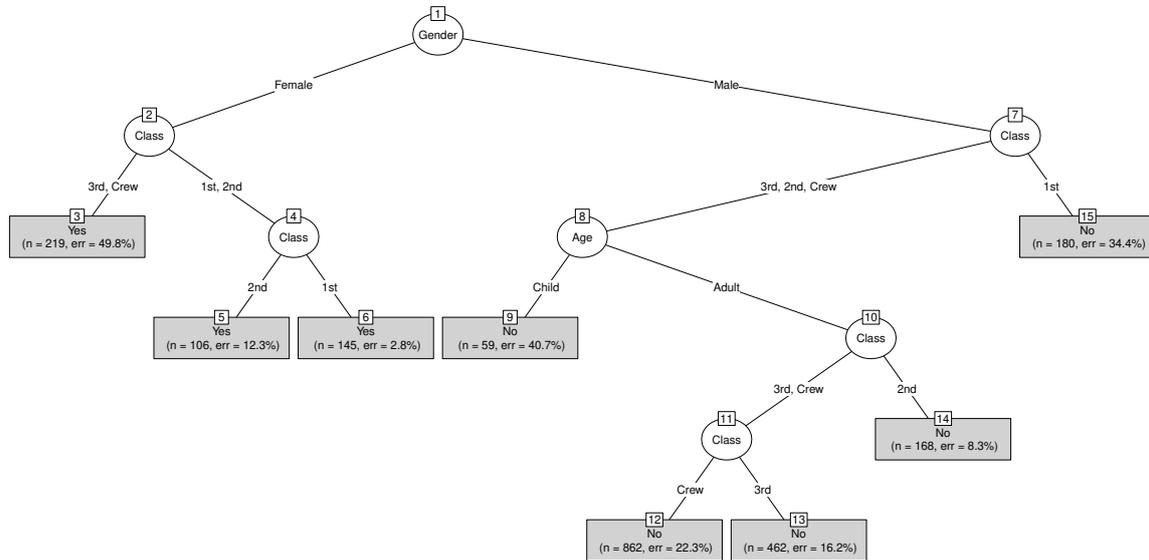

Figure 3: QUEST tree for Titanic data, fitted using SPSS and exported via PMML.

description and hence one can only obtain and display the summarized information provided by PMML.

In this particular case, however, we have the learning data available in R because we had exported the data from R to begin with. Hence, for this tree we can augment the “`simpleparty`” with the full learning sample to create a “`constparty`”. As SPSS had reordered some factor levels we need to carry out this reordering as well”

```
> ttnc2 <- ttnc[, names(ttnc_quest$data)]
> for(n in names(ttnc2)) {
+   if(is.factor(ttnc2[[n]])) ttnc2[[n]] <- factor(
+     ttnc2[[n]], levels = levels(ttnc_quest$data[[n]]))
+ }
```

Using this data all information for a “`constparty`” can be easily computed:

```
> ttnc_quest2 <- party(ttnc_quest$node,
+ data = ttnc2,
+ fitted = data.frame(
+   "(fitted)" = predict(ttnc_quest, ttnc2, type = "node"),
+   "(response)" = ttnc2$Survived,
+   check.names = FALSE),
+ terms = terms(Survived ~ ., data = ttnc2)
+ )
> ttnc_quest2 <- as.constparty(ttnc_quest2)
```

This object is plotted in Figure 4.

```
> plot(ttnc_quest2)
```

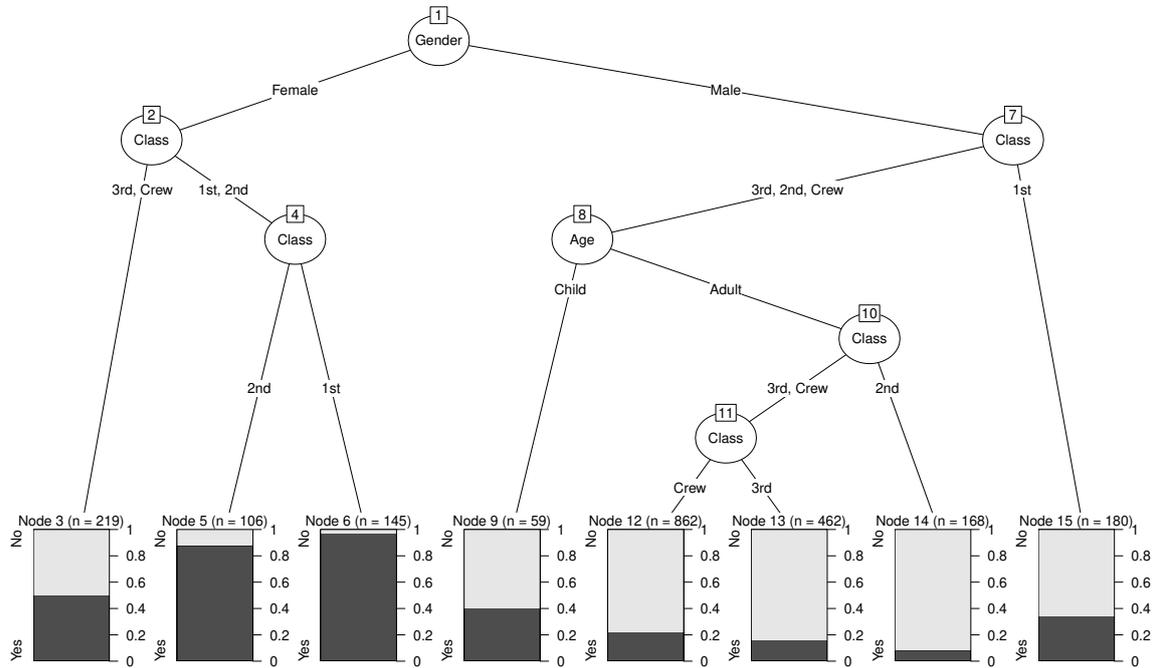

Figure 4: QUEST tree for Titanic data, fitted using SPSS, exported via PMML, and transformed into a “constparty” object.

Furthermore, we briefly point out that there is also the R package **pmml** (Williams, Jena, Hahsler, Zementis Inc., Ishwaran, Kogalur, and Guha 2014), part of the **rattle** project (Williams 2011), that allows to export PMML files for **rpart** trees from R. For example, for the “**rpart**” tree for the Titanic data:

```
> library("pmml")
> tfile <- tempfile()
> write(toString(pmml(rp)), file = tfile)
```

Then, we can simply read this file and inspect the resulting tree

```
> (party_pmml <- pmmlTreeModel(tfile))
```

Model formula:

```
Survived ~ Class + Gender + Age
```

Fitted party:

```
[1] root
| [2] Gender in Male
| | [3] Age in Adult: No (n = 1667, err = 20.3%)
| | [4] Age in Child
```

```
| | | [5] Class in 3rd: No (n = 48, err = 27.1%)
| | | [6] Class in 1st, 2nd: Yes (n = 16, err = 0.0%)
| [7] Gender in Female
| | [8] Class in 3rd: No (n = 196, err = 45.9%)
| | [9] Class in 1st, 2nd, Crew: Yes (n = 274, err = 7.3%)
```

```
Number of inner nodes: 4
Number of terminal nodes: 5
```

```
> all.equal(predict(party_rp, newdata = ttnc, type = "prob"),
+ predict(party_pmml, newdata = ttnc, type = "prob"),
+ check.attributes = FALSE)
```

```
[1] TRUE
```

Further example PMML files created with **rattle** are the Data Mining Group web page, e.g., [http://www.dmg.org/pmml\\_examples/rattle\\_pmml\\_examples/AuditTree.xml](http://www.dmg.org/pmml_examples/rattle_pmml_examples/AuditTree.xml) or [http://www.dmg.org/pmml\\_examples/rattle\\_pmml\\_examples/IrisTree.xml](http://www.dmg.org/pmml_examples/rattle_pmml_examples/IrisTree.xml).

### 3. Growing a simple classification tree

Although the **partykit** package offers an extensive toolbox for handling trees along with implementations of various tree algorithms, it does not offer unified infrastructure for *growing* trees. However, once you know how to estimate splits from data, it is fairly straightforward to implement trees. Consider a very simple CHAID-style algorithm (in fact so simple that we would advise *not to use it* for any real application). We assume that both response and explanatory variables are factors, as for the Titanic data set. First we determine the best explanatory variable by means of a global  $\chi^2$  test, i.e., splitting up the response into all levels of each explanatory variable. Then, for the selected explanatory variable we search for the binary best split by means of  $\chi^2$  tests, i.e., we cycle through all potential split points and assess the quality of the split by comparing the distributions of the response in the so-defined two groups. In both cases, we select the split variable/point with lowest  $p$ -value from the  $\chi^2$  test, however, only if the global test is significant at Bonferroni-corrected level  $\alpha = 0.01$ .

This strategy can be implemented based on the data (response and explanatory variables) and some case weights as follows (`response` is just the name of the response and `data` is a data frame with all variables):

```
> findsplit <- function(response, data, weights, alpha = 0.01) {
+
+   ## extract response values from data
+   y <- factor(rep(data[[response]], weights))
+
+   ## perform chi-squared test of y vs. x
+   mychisqtest <- function(x) {
+     x <- factor(x)
+     if(length(levels(x)) < 2) return(NA)
```

```

+   ct <- suppressWarnings(chisq.test(table(y, x), correct = FALSE))
+   pchisq(ct$statistic, ct$parameter, log = TRUE, lower.tail = FALSE)
+ }
+ xselect <- which(names(data) != response)
+ logp <- sapply(xselect, function(i) mychisqtest(rep(data[[i]], weights)))
+ names(logp) <- names(data)[xselect]
+
+ ## Bonferroni-adjusted p-value small enough?
+ if(all(is.na(logp))) return(NULL)
+ minp <- exp(min(logp, na.rm = TRUE))
+ minp <- 1 - (1 - minp)^sum(!is.na(logp))
+ if(minp > alpha) return(NULL)
+
+ ## for selected variable, search for split minimizing p-value
+ xselect <- xselect[which.min(logp)]
+ x <- rep(data[[xselect]], weights)
+
+ ## set up all possible splits in two kid nodes
+ lev <- levels(x[drop = TRUE])
+ if(length(lev) == 2) {
+   splitpoint <- lev[1]
+ } else {
+   comb <- do.call("c", lapply(1:(length(lev) - 2),
+     function(x) combn(lev, x, simplify = FALSE)))
+   xlogp <- sapply(comb, function(q) mychisqtest(x %in% q))
+   splitpoint <- comb[[which.min(xlogp)]]
+ }
+
+ ## split into two groups (setting groups that do not occur to NA)
+ splitindex <- !(levels(data[[xselect]]) %in% splitpoint)
+ splitindex[!(levels(data[[xselect]]) %in% lev)] <- NA_integer_
+ splitindex <- splitindex - min(splitindex, na.rm = TRUE) + 1L
+
+ ## return split as partysplit object
+ return(partysplit(varid = as.integer(xselect),
+   index = splitindex,
+   info = list(p.value = 1 - (1 - exp(logp))^sum(!is.na(logp))))))
+ }

```

In order to actually grow a tree on data, we have to set up the recursion for growing a recursive “partynode” structure:

```

> growtree <- function(id = 1L, response, data, weights, minbucket = 30) {
+
+   ## for less than 30 observations stop here
+   if (sum(weights) < minbucket) return(partynode(id = id))
+
+

```

```

+ ## find best split
+ sp <- findsplit(response, data, weights)
+ ## no split found, stop here
+ if (is.null(sp)) return(partynode(id = id))
+
+ ## actually split the data
+ kidids <- kidids_split(sp, data = data)
+
+ ## set up all daughter nodes
+ kids <- vector(mode = "list", length = max(kidids, na.rm = TRUE))
+ for (kidid in 1:length(kids)) {
+   ## select observations for current node
+   w <- weights
+   w[kidids != kidid] <- 0
+   ## get next node id
+   if (kidid > 1) {
+     myid <- max(nodeids(kids[[kidid - 1]]))
+   } else {
+     myid <- id
+   }
+   ## start recursion on this daughter node
+   kids[[kidid]] <- growtree(id = as.integer(myid + 1), response, data, w)
+ }
+
+ ## return nodes
+ return(partynode(id = as.integer(id), split = sp, kids = kids,
+   info = list(p.value = min(info_split(sp)$p.value, na.rm = TRUE)))
+ }

```

A very rough sketch of a formula-based user-interface sets-up the data and calls `growtree()`:

```

> mytree <- function(formula, data, weights = NULL) {
+
+   ## name of the response variable
+   response <- all.vars(formula)[1]
+   ## data without missing values, response comes last
+   data <- data[complete.cases(data), c(all.vars(formula)[-1], response)]
+   ## data is factors only
+   stopifnot(all(sapply(data, is.factor)))
+
+   if (is.null(weights)) weights <- rep(1L, nrow(data))
+   ## weights are case weights, i.e., integers
+   stopifnot(length(weights) == nrow(data) &
+     max(abs(weights - floor(weights))) < .Machine$double.eps)
+
+   ## grow tree
+   nodes <- growtree(id = 1L, response, data, weights)

```

```

+
+   ## compute terminal node number for each observation
+   fitted <- fitted_node(nodes, data = data)
+   ## return rich constparty object
+   ret <- party(nodes, data = data,
+     fitted = data.frame("(fitted)" = fitted,
+       "(response)" = data[[response]],
+       "(weights)" = weights,
+       check.names = FALSE),
+     terms = terms(formula))
+   as.constparty(ret)
+ }

```

The call to the constructor `party()` sets-up a “party” object with the tree structure contained in `nodes`, the training samples in `data` and the corresponding `terms` object. Class “constparty” inherits all slots from class “party” and has an additional `fitted` slot for storing the terminal node numbers for each sample in the training data, the response variable(s) and case weights. The `fitted` slot is a “data.frame” containing three variables: The fitted terminal node identifiers “(fitted)”, an integer vector of the same length as `data`; the response variables “(response)” as a vector (or `data.frame` for multivariate responses) with the same number of observations; and optionally a vector of weights “(weights)”. The additional `fitted` slot allows to compute arbitrary summary measures for each terminal node by simply subsetting the “(response)” and “(weights)” slots by “(fitted)” before computing (weighted) means, medians, empirical cumulative distribution functions, Kaplan-Meier estimates or whatever summary statistic might be appropriate for a certain response. The `print()`, `plot()`, and `predict()` methods for class “constparty” work this way with suitable defaults for the summary statistics depending on the class of the response(s).

We now can fit this tree to the Titanic data; the `print()` method provides us with a first overview on the resulting model

```
> (myttnc <- mytree(Survived ~ Class + Age + Gender, data = ttnc))
```

Model formula:

```
Survived ~ Class + Age + Gender
```

Fitted party:

```

[1] root
|   [2] Gender in Male
|   |   [3] Class in 1st
|   |   |   [4] Age in Child: Yes (n = 5, err = 0.0%)
|   |   |   [5] Age in Adult: No (n = 175, err = 32.6%)
|   |   [6] Class in 2nd, 3rd, Crew
|   |   |   [7] Age in Child
|   |   |   |   [8] Class in 2nd: Yes (n = 11, err = 0.0%)
|   |   |   |   [9] Class in 3rd: No (n = 48, err = 27.1%)
|   |   [10] Age in Adult
|   |   |   [11] Class in Crew: No (n = 862, err = 22.3%)

```

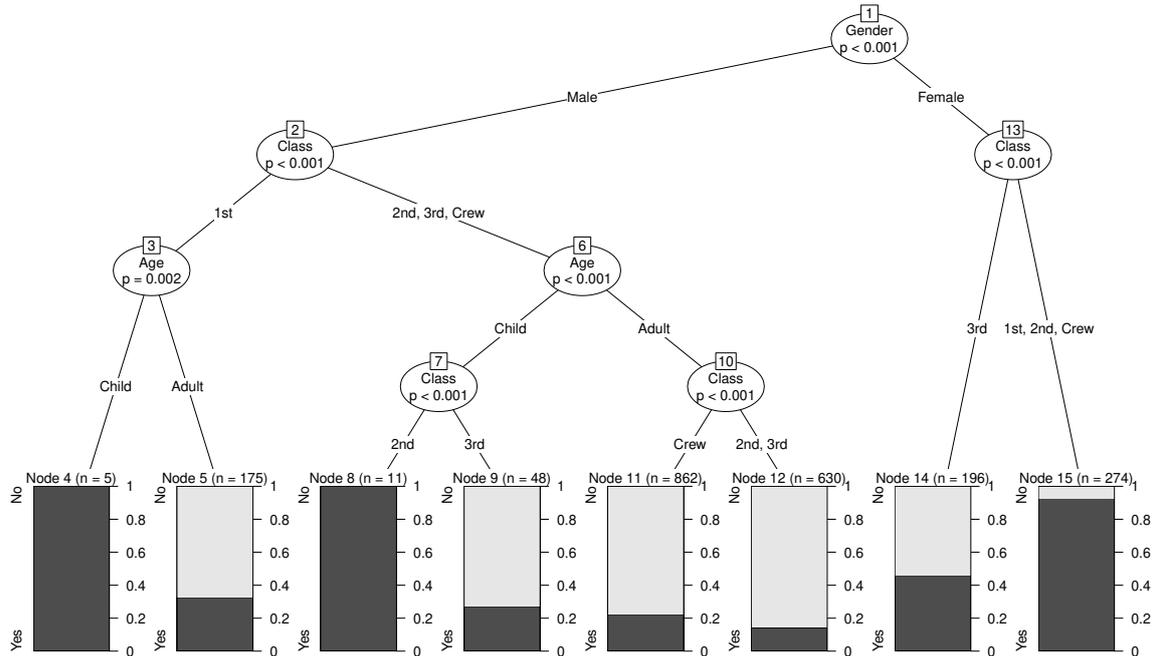Figure 5: Classification tree fitted by the `mytree()` function to the `ttnc` data.

```
| | | | [12] Class in 2nd, 3rd: No (n = 630, err = 14.1%)
| [13] Gender in Female
| | [14] Class in 3rd: No (n = 196, err = 45.9%)
| | [15] Class in 1st, 2nd, Crew: Yes (n = 274, err = 7.3%)
```

```
Number of inner nodes: 7
Number of terminal nodes: 8
```

Of course, we can immediately use `plot(myttnc)` to obtain a graphical representation of this tree, the result is given in Figure 5. The default behavior for trees with categorical responses is simply inherited from “`constparty`” and hence we readily obtain bar plots in all terminal nodes.

As the tree is fairly large, we might be interested in pruning the tree to a more reasonable size. For this purpose the `partykit` package provides the `nodeprune()` function that can prune back to nodes with selected IDs. As `nodeprune()` (by design) does not provide a specific pruning criterion, we need to determine ourselves which nodes to prune. Here, one idea could be to impose significance at a higher level than the default  $10^{-2}$  – say  $10^{-5}$  to obtain a strongly pruned tree. Hence we use `nodeapply()` to extract the minimal Bonferroni-corrected  $p$ -value from all inner nodes:

```
> nid <- nodeids(myttnc)
> iid <- nid[!(nid %in% nodeids(myttnc, terminal = TRUE))]
> (pval <- unlist(nodeapply(myttnc, ids = iid,
+ FUN = function(n) info_node(n)$p.value)))
```

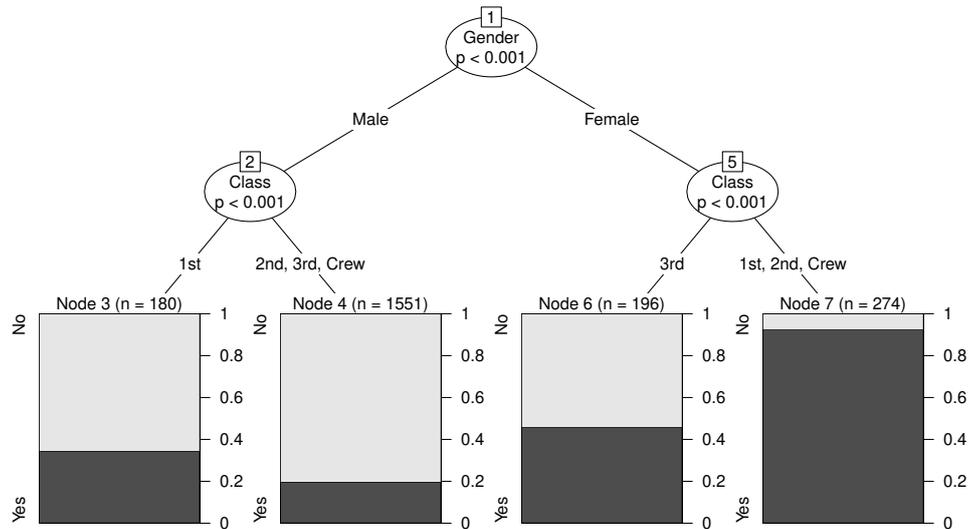

Figure 6: Pruned classification tree fitted by the `mytree()` function to the `ttnc` data.

```

          1          2          3          6          7
0.000000e+00 2.965383e-06 1.756527e-03 6.933623e-05 8.975754e-06
          10          13
2.992870e-05 0.000000e+00

```

Then, the pruning of the nodes with the larger  $p$ -values can be simply carried out by

```
> myttnc2 <- nodeprune(myttnc, ids = iid[pval > 1e-5])
```

The corresponding visualization is shown in Figure 6.

The accuracy of the tree built using the default options could be assessed by the bootstrap, for example. Here, we want to compare our tree for the Titanic survivor data with a simple logistic regression model. First, we fit this simple GLM and compute the (in-sample) log-likelihood:

```
> logLik(glm(Survived ~ Class + Age + Gender, data = ttnc,
+           family = binomial()))
```

```
'log Lik.' -1105.031 (df=6)
```

For our tree, we set-up 25 bootstrap samples

```
> bs <- rmultinom(25, nrow(ttnc), rep(1, nrow(ttnc)) / nrow(ttnc))
```

and implement the log-likelihood of a binomial model

```
> bloglik <- function(prob, weights)
+   sum(weights * dbinom(ttnc$Survived == "Yes", size = 1,
+   prob[, "Yes"], log = TRUE))
```

What remains to be done is to iterate over all bootstrap samples, to refit the tree on the bootstrap sample and to evaluate the log-likelihood on the out-of-bootstrap samples based on the trees' predictions (details on how to compute predictions are given in the next section):

```
> f <- function(w) {
+   tr <- mytree(Survived ~ Class + Age + Gender, data = ttnc, weights = w)
+   bloglik(predict(tr, newdata = ttnc, type = "prob"), as.numeric(w == 0))
+ }
> apply(bs, 2, f)

[1] -390.2268 -410.8696 -377.7492 -416.7790 -396.5327 -383.9575
[7] -389.4972 -405.8401 -379.9248 -384.7071 -381.1303 -394.8712
[13] -409.8711 -385.3753 -396.2723 -385.6372 -408.9187 -412.4585
[19] -401.3972 -403.0548 -406.7881 -389.8507 -408.0418 -392.1441
[25] -389.4687
```

We see that the in-sample log-likelihood of the linear logistic regression model is much smaller than the out-of-sample log-likelihood found for our tree and thus we can conclude that our tree-based approach fits data the better than the linear model.

## 4. Predictions

As argued in Section 1 arbitrary types of predictions can be computed from “`constparty`” objects because the full empirical distribution of the response in the learning sample nodes is available. All of these can be easily computed in the `predict()` method for “`constparty`” objects by supplying a suitable aggregation function. However, as certain types of predictions are much more commonly used, these are available even more easily by setting a `type` argument.

The prediction `type` can either be “`node`”, “`response`”, or “`prob`” (see Table 1). The idea is that “`response`” always returns a prediction of the same class as the original response and “`prob`” returns some object that characterizes the entire empirical distribution. Hence, for different response classes, different types of predictions are produced, see Table 1 for an overview. Additionally, for “`numeric`” responses `type = "quantile"` and `type = "density"` is available. By default, these return functions for computing predicted quantiles and probability densities, respectively, but optionally these functions can be directly evaluated at given values and then return a vector/matrix.

Here, we illustrate all different predictions for all possible combinations of the explanatory factor levels.

| Response class           | <code>type = "node"</code> | <code>type = "response"</code> | <code>type = "prob"</code> |
|--------------------------|----------------------------|--------------------------------|----------------------------|
| “ <code>factor</code> ”  | terminal node number       | majority class                 | class probabilities        |
| “ <code>numeric</code> ” | terminal node number       | mean                           | ECDF                       |
| “ <code>Surv</code> ”    | terminal node number       | median survival time           | Kaplan-Meier               |

Table 1: Overview on type of predictions computed by the `predict()` method for “`constparty`” objects. For multivariate responses, combinations thereof are returned.

```
> nttnc <- expand.grid(Class = levels(ttnc$Class),
+   Gender = levels(ttnc$Gender), Age = levels(ttnc$Age))
> nttnc
```

|    | Class | Gender | Age   |
|----|-------|--------|-------|
| 1  | 1st   | Male   | Child |
| 2  | 2nd   | Male   | Child |
| 3  | 3rd   | Male   | Child |
| 4  | Crew  | Male   | Child |
| 5  | 1st   | Female | Child |
| 6  | 2nd   | Female | Child |
| 7  | 3rd   | Female | Child |
| 8  | Crew  | Female | Child |
| 9  | 1st   | Male   | Adult |
| 10 | 2nd   | Male   | Adult |
| 11 | 3rd   | Male   | Adult |
| 12 | Crew  | Male   | Adult |
| 13 | 1st   | Female | Adult |
| 14 | 2nd   | Female | Adult |
| 15 | 3rd   | Female | Adult |
| 16 | Crew  | Female | Adult |

The corresponding predicted nodes, modes, and probability distributions are:

```
> predict(myttnc, newdata = nttnc, type = "node")
```

|   |   |   |   |    |    |    |    |   |    |    |    |    |    |    |    |
|---|---|---|---|----|----|----|----|---|----|----|----|----|----|----|----|
| 1 | 2 | 3 | 4 | 5  | 6  | 7  | 8  | 9 | 10 | 11 | 12 | 13 | 14 | 15 | 16 |
| 4 | 8 | 9 | 9 | 15 | 15 | 14 | 15 | 5 | 12 | 12 | 11 | 15 | 15 | 14 | 15 |

```
> predict(myttnc, newdata = nttnc, type = "response")
```

|                |     |    |     |     |     |    |     |    |    |    |    |     |     |    |     |
|----------------|-----|----|-----|-----|-----|----|-----|----|----|----|----|-----|-----|----|-----|
| 1              | 2   | 3  | 4   | 5   | 6   | 7  | 8   | 9  | 10 | 11 | 12 | 13  | 14  | 15 | 16  |
| Yes            | Yes | No | Yes | Yes | Yes | No | Yes | No | No | No | No | Yes | Yes | No | Yes |
| Levels: No Yes |     |    |     |     |     |    |     |    |    |    |    |     |     |    |     |

```
> predict(myttnc, newdata = nttnc, type = "prob")
```

|   | No        | Yes       |
|---|-----------|-----------|
| 1 | 0.0000000 | 1.0000000 |
| 2 | 0.0000000 | 1.0000000 |
| 3 | 0.7291667 | 0.2708333 |
| 4 | 0.0000000 | 1.0000000 |
| 5 | 0.0729927 | 0.9270073 |
| 6 | 0.0729927 | 0.9270073 |
| 7 | 0.5408163 | 0.4591837 |
| 8 | 0.0729927 | 0.9270073 |

```

9 0.6742857 0.3257143
10 0.8587302 0.1412698
11 0.8587302 0.1412698
12 0.7772622 0.2227378
13 0.0729927 0.9270073
14 0.0729927 0.9270073
15 0.5408163 0.4591837
16 0.0729927 0.9270073

```

Furthermore, the `predict()` method features a `FUN` argument that can be used to compute customized predictions. If we are, say, interested in the rank of the probabilities for the two classes, we can simply specify a function that implements this feature:

```

> predict(myttnc, newdata = nttnc, FUN = function(y, w)
+   rank(table(rep(y, w))))

```

|    | No | Yes |
|----|----|-----|
| 1  | 1  | 2   |
| 2  | 1  | 2   |
| 3  | 2  | 1   |
| 4  | 1  | 2   |
| 5  | 1  | 2   |
| 6  | 1  | 2   |
| 7  | 2  | 1   |
| 8  | 1  | 2   |
| 9  | 2  | 1   |
| 10 | 2  | 1   |
| 11 | 2  | 1   |
| 12 | 2  | 1   |
| 13 | 1  | 2   |
| 14 | 1  | 2   |
| 15 | 2  | 1   |
| 16 | 1  | 2   |

The user-supplied function `FUN` takes two arguments, `y` is the response and `w` is a vector of weights (case weights in this situation). Of course, it would have been easier to do these computations directly on the conditional class probabilities (`type = "prob"`), but the approach taken here for illustration generalizes to situations where this is not possible, especially for numeric responses.

## 5. Conclusion

The classes “`constparty`” and “`simpleparty`” introduced here can be used to represent trees with constant fits in the terminal nodes, including most of the traditional tree variants. For a number of implementations it is possible to convert the resulting trees to one of these classes, thus offering unified methods for handling constant-fit trees. User-extensible methods for

printing and plotting these trees are available. Also, computing non-standard predictions, such as the median or empirical cumulative distribution functions, is easily possible within this framework. With the infrastructure provided in **partykit** it is rather straightforward to implement a new (or old) tree algorithm and therefore a prototype implementation of fancy ideas for improving trees is only a couple lines of R code away.

## References

- Breiman L, Friedman JH, Olshen RA, Stone CJ (1984). *Classification and Regression Trees*. Wadsworth, California.
- Data Mining Group (2014). “Predictive Model Markup Language.” Version 4.2, URL <http://www.dmg.org/>.
- Hornik K, Buchta C, Zeileis A (2009). “Open-Source Machine Learning: R Meets **Weka**.” *Computational Statistics*, **24**(2), 225–232.
- Hothorn T, Hornik K, Zeileis A (2006). “Unbiased Recursive Partitioning: A Conditional Inference Framework.” *Journal of Computational and Graphical Statistics*, **15**(3), 651–674. doi:10.1198/106186006X133933.
- Kass GV (1980). “An Exploratory Technique for Investigating Large Quantities of Categorical Data.” *Applied Statistics*, **29**(2), 119–127.
- Loh WY, Shih YS (1997). “Split Selection Methods for Classification Trees.” *Statistica Sinica*, **7**, 815–840.
- Loh WY, Vanichsetakul N (1988). “Tree-Structured Classification via Generalized Discriminant Analysis.” *Journal of the American Statistical Association*, **83**, 715–725.
- Morgan JN, Sonquist JA (1963). “Problems in the Analysis of Survey Data, and a Proposal.” *Journal of the American Statistical Association*, **58**, 415–434.
- Quinlan JR (1993). *C4.5: Programs for Machine Learning*. Morgan Kaufmann Publishers, San Mateo.
- Therneau TM, Atkinson EJ (1997). “An Introduction to Recursive Partitioning Using the **rpart** Routine.” *Technical Report 61*, Section of Biostatistics, Mayo Clinic, Rochester. URL <http://www.mayo.edu/hsr/techrpt/61.pdf>.
- Williams G (2011). *Data Mining with **rattle** and R: The Art of Excavating Data for Knowledge Discovery*. Springer-Verlag, New York. URL <http://CRAN.R-project.org/package=rattle>.
- Williams G, Jena T, Hahsler M, Zementis Inc, Ishwaran H, Kogalur UB, Guha R (2014). *pmml: Generate PMML for Various Models*. R package version 1.4.2, URL <http://CRAN.R-project.org/package=pmml>.

**Affiliation:**

Torsten Hothorn  
Institut für Epidemiologie, Biostatistik und Prävention  
Universität Zürich  
Hirschengraben 84  
CH-8001 Zürich, Switzerland  
E-mail: [Torsten.Hothorn@R-project.org](mailto:Torsten.Hothorn@R-project.org)  
URL: <http://user.math.uzh.ch/hothorn/>

Achim Zeileis  
Department of Statistics  
Faculty of Economics and Statistics  
Universität Innsbruck  
Universitätsstr. 15  
6020 Innsbruck, Austria  
E-mail: [Achim.Zeileis@R-project.org](mailto:Achim.Zeileis@R-project.org)  
URL: <http://eeecon.uibk.ac.at/~zeileis/>
