# Supplementary material for: The Power of Unbiased Recursive Partitioning: A Unifying View of CTree, MOB, and GUIDE
Source: arXiv:1906.10179 ancillary file (2019-06-24)
Supplement: Supplementary file 2 [file ctree.pdf]

# ctree: Conditional Inference Trees

**Torsten Hothorn**  
Universität Zürich

**Kurt Hornik**  
Wirtschaftsuniversität Wien

**Achim Zeileis**  
Universität Innsbruck

---

## Abstract

This vignette describes the new reimplementation of conditional inference trees (CTree) in the R package **partykit**. CTree is a non-parametric class of regression trees embedding tree-structured regression models into a well defined theory of conditional inference procedures. It is applicable to all kinds of regression problems, including nominal, ordinal, numeric, censored as well as multivariate response variables and arbitrary measurement scales of the covariates. The vignette comprises a practical guide to exploiting the flexible and extensible computational tools in **partykit** for fitting and visualizing conditional inference trees.

*Keywords:* conditional inference, non-parametric models, recursive partitioning.

---

## 1. Overview

This vignette describes conditional inference trees (Hothorn, Hornik, and Zeileis 2006) along with its new and improved reimplementation in package **partykit**. Originally, the method was implemented in the package **party** almost entirely in C while the new implementation is now almost entirely in R. In particular, this has the advantage that all the generic infrastructure from **partykit** can be reused, making many computations more modular and easily extensible. Hence, `partykit::ctree` is the new reference implementation that will be improved and developed further in the future.

In almost all cases, the two implementations will produce identical trees. In exceptional cases, additional parameters have to be specified in order to ensure backward compatibility. These and novel features in `ctree:partykit` are introduced in Section 7.

## 2. Introduction

The majority of recursive partitioning algorithms are special cases of a simple two-stage algorithm: First partition the observations by univariate splits in a recursive way and second fit a constant model in each cell of the resulting partition. The most popular implementations of such algorithms are ‘CART’ (Breiman, Friedman, Olshen, and Stone 1984) and ‘C4.5’ (Quinlan 1993). Not unlike AID, both perform an exhaustive search over all possible splits maximizing an information measure of node impurity selecting the covariate showing the best split. This approach has two fundamental problems: overfitting and a selection bias towards covariates with many possible splits. With respect to the overfitting problem Mingers (1987) notes that the algorithm

[...] has no concept of statistical significance, and so cannot distinguish between a significant and an insignificant improvement in the information measure.

With conditional inference trees (see [Hothorn et al. 2006](#), for a full description of its methodological foundations) we enter at the point where [White and Liu \(1994\)](#) demand for

[...] a *statistical* approach [to recursive partitioning] which takes into account the *distributional* properties of the measures.

We present a unified framework embedding recursive binary partitioning into the well defined theory of permutation tests developed by [Strasser and Weber \(1999\)](#). The conditional distribution of statistics measuring the association between responses and covariates is the basis for an unbiased selection among covariates measured at different scales. Moreover, multiple test procedures are applied to determine whether no significant association between any of the covariates and the response can be stated and the recursion needs to stop.

### 3. Recursive binary partitioning

We focus on regression models describing the conditional distribution of a response variable  $\mathbf{Y}$  given the status of  $m$  covariates by means of tree-structured recursive partitioning. The response  $\mathbf{Y}$  from some sample space  $\mathcal{Y}$  may be multivariate as well. The  $m$ -dimensional covariate vector  $\mathbf{X} = (X_1, \dots, X_m)$  is taken from a sample space  $\mathcal{X} = \mathcal{X}_1 \times \dots \times \mathcal{X}_m$ . Both response variable and covariates may be measured at arbitrary scales. We assume that the conditional distribution  $D(\mathbf{Y}|\mathbf{X})$  of the response  $\mathbf{Y}$  given the covariates  $\mathbf{X}$  depends on a function  $f$  of the covariates

$$D(\mathbf{Y}|\mathbf{X}) = D(\mathbf{Y}|X_1, \dots, X_m) = D(\mathbf{Y}|f(X_1, \dots, X_m)),$$

where we restrict ourselves to partition based regression relationships, i.e.,  $r$  disjoint cells  $B_1, \dots, B_r$  partitioning the covariate space  $\mathcal{X} = \bigcup_{k=1}^r B_k$ . A model of the regression relationship is to be fitted based on a learning sample  $\mathcal{L}_n$ , i.e., a random sample of  $n$  independent and identically distributed observations, possibly with some covariates  $X_{ji}$  missing,

$$\mathcal{L}_n = \{(\mathbf{Y}_i, X_{1i}, \dots, X_{mi}); i = 1, \dots, n\}.$$

A generic algorithm for recursive binary partitioning for a given learning sample  $\mathcal{L}_n$  can be formulated using non-negative integer valued case weights  $\mathbf{w} = (w_1, \dots, w_n)$ . Each node of a tree is represented by a vector of case weights having non-zero elements when the corresponding observations are elements of the node and are zero otherwise. The following algorithm implements recursive binary partitioning:

1. For case weights  $\mathbf{w}$  test the global null hypothesis of independence between any of the  $m$  covariates and the response. Stop if this hypothesis cannot be rejected. Otherwise select the covariate  $X_{j^*}$  with strongest association to  $\mathbf{Y}$ .
2. Choose a set  $A^* \subset \mathcal{X}_{j^*}$  in order to split  $\mathcal{X}_{j^*}$  into two disjoint sets  $A^*$  and  $\mathcal{X}_{j^*} \setminus A^*$ . The case weights  $\mathbf{w}_{\text{left}}$  and  $\mathbf{w}_{\text{right}}$  determine the two subgroups with  $w_{\text{left},i} = w_i I(X_{j^*i} \in A^*)$  and  $w_{\text{right},i} = w_i I(X_{j^*i} \notin A^*)$  for all  $i = 1, \dots, n$  ( $I(\cdot)$  denotes the indicator function).

3. Recursively repeat steps 1 and 2 with modified case weights  $\mathbf{w}_{\text{left}}$  and  $\mathbf{w}_{\text{right}}$ , respectively.

The separation of variable selection and splitting procedure into steps 1 and 2 of the algorithm is the key for the construction of interpretable tree structures not suffering a systematic tendency towards covariates with many possible splits or many missing values. In addition, a statistically motivated and intuitive stopping criterion can be implemented: We stop when the global null hypothesis of independence between the response and any of the  $m$  covariates cannot be rejected at a pre-specified nominal level  $\alpha$ . The algorithm induces a partition  $\{B_1, \dots, B_r\}$  of the covariate space  $\mathcal{X}$ , where each cell  $B \in \{B_1, \dots, B_r\}$  is associated with a vector of case weights.

## 4. Recursive partitioning by conditional inference

In the main part of this section we focus on step 1 of the generic algorithm. Unified tests for independence are constructed by means of the conditional distribution of linear statistics in the permutation test framework developed by [Strasser and Weber \(1999\)](#). The determination of the best binary split in one selected covariate and the handling of missing values is performed based on standardized linear statistics within the same framework as well.

### 4.1. Variable selection and stopping criteria

At step 1 of the generic algorithm given in Section 3 we face an independence problem. We need to decide whether there is any information about the response variable covered by any of the  $m$  covariates. In each node identified by case weights  $\mathbf{w}$ , the global hypothesis of independence is formulated in terms of the  $m$  partial hypotheses  $H_0^j : D(\mathbf{Y}|X_j) = D(\mathbf{Y})$  with global null hypothesis  $H_0 = \bigcap_{j=1}^m H_0^j$ . When we are not able to reject  $H_0$  at a pre-specified level  $\alpha$ , we stop the recursion. If the global hypothesis can be rejected, we measure the association between  $\mathbf{Y}$  and each of the covariates  $X_j, j = 1, \dots, m$ , by test statistics or  $P$ -values indicating the deviation from the partial hypotheses  $H_0^j$ .

For notational convenience and without loss of generality we assume that the case weights  $w_i$  are either zero or one. The symmetric group of all permutations of the elements of  $(1, \dots, n)$  with corresponding case weights  $w_i = 1$  is denoted by  $S(\mathcal{L}_n, \mathbf{w})$ . A more general notation is given in the Appendix. We measure the association between  $\mathbf{Y}$  and  $X_j, j = 1, \dots, m$ , by linear statistics of the form

$$\mathbf{T}_j(\mathcal{L}_n, \mathbf{w}) = \text{vec} \left( \sum_{i=1}^n w_i g_j(X_{ji}) h(\mathbf{Y}_i, (\mathbf{Y}_1, \dots, \mathbf{Y}_n))^\top \right) \in \mathbb{R}^{p_j q} \quad (1)$$

where  $g_j : \mathcal{X}_j \rightarrow \mathbb{R}^{p_j}$  is a non-random transformation of the covariate  $X_j$ . The transformation may be specified using the `xtrafo` argument (Note: this argument is currently not implemented in `partykit::ctree` but is available from `party::ctree`). The *influence function*  $h : \mathcal{Y} \times \mathcal{Y}^n \rightarrow \mathbb{R}^q$  depends on the responses  $(\mathbf{Y}_1, \dots, \mathbf{Y}_n)$  in a permutation symmetric way. Section 5 explains how to choose  $g_j$  and  $h$  in different practical settings. A  $p_j \times q$  matrix is converted into a  $p_j q$  column vector by column-wise combination using the ‘vec’ operator. The influence function can be specified using the `ytrafo` argument.

The distribution of  $\mathbf{T}_j(\mathcal{L}_n, \mathbf{w})$  under  $H_0^j$  depends on the joint distribution of  $\mathbf{Y}$  and  $X_j$ , which is unknown under almost all practical circumstances. At least under the null hypothesis

one can dispose of this dependency by fixing the covariates and conditioning on all possible permutations of the responses. This principle leads to test procedures known as *permutation tests*. The conditional expectation  $\mu_j \in \mathbb{R}^{p_j q}$  and covariance  $\Sigma_j \in \mathbb{R}^{p_j q \times p_j q}$  of  $\mathbf{T}_j(\mathcal{L}_n, \mathbf{w})$  under  $H_0$  given all permutations  $\sigma \in S(\mathcal{L}_n, \mathbf{w})$  of the responses are derived by [Strasser and Weber \(1999\)](#):

$$\begin{aligned} \mu_j &= \mathbb{E}(\mathbf{T}_j(\mathcal{L}_n, \mathbf{w}) | S(\mathcal{L}_n, \mathbf{w})) = \text{vec} \left( \left( \sum_{i=1}^n w_i g_j(X_{ji}) \right) \mathbb{E}(h | S(\mathcal{L}_n, \mathbf{w}))^\top \right), \\ \Sigma_j &= \mathbb{V}(\mathbf{T}_j(\mathcal{L}_n, \mathbf{w}) | S(\mathcal{L}_n, \mathbf{w})) \\ &= \frac{\mathbf{w} \cdot}{\mathbf{w} \cdot - 1} \mathbb{V}(h | S(\mathcal{L}_n, \mathbf{w})) \otimes \left( \sum_i w_i g_j(X_{ji}) \otimes w_i g_j(X_{ji})^\top \right) \\ &\quad - \frac{1}{\mathbf{w} \cdot - 1} \mathbb{V}(h | S(\mathcal{L}_n, \mathbf{w})) \otimes \left( \sum_i w_i g_j(X_{ji}) \right) \otimes \left( \sum_i w_i g_j(X_{ji}) \right)^\top \end{aligned} \quad (2)$$

where  $\mathbf{w} \cdot = \sum_{i=1}^n w_i$  denotes the sum of the case weights,  $\otimes$  is the Kronecker product and the conditional expectation of the influence function is

$$\mathbb{E}(h | S(\mathcal{L}_n, \mathbf{w})) = \mathbf{w} \cdot^{-1} \sum_i w_i h(\mathbf{Y}_i, (\mathbf{Y}_1, \dots, \mathbf{Y}_n)) \in \mathbb{R}^q$$

with corresponding  $q \times q$  covariance matrix

$$\begin{aligned} \mathbb{V}(h | S(\mathcal{L}_n, \mathbf{w})) &= \mathbf{w} \cdot^{-1} \sum_i w_i (h(\mathbf{Y}_i, (\mathbf{Y}_1, \dots, \mathbf{Y}_n)) - \mathbb{E}(h | S(\mathcal{L}_n, \mathbf{w}))) \\ &\quad (h(\mathbf{Y}_i, (\mathbf{Y}_1, \dots, \mathbf{Y}_n)) - \mathbb{E}(h | S(\mathcal{L}_n, \mathbf{w})))^\top. \end{aligned}$$

Having the conditional expectation and covariance at hand we are able to standardize a linear statistic  $\mathbf{T} \in \mathbb{R}^{pq}$  of the form (1) for some  $p \in \{p_1, \dots, p_m\}$ . Univariate test statistics  $c$  mapping an observed multivariate linear statistic  $\mathbf{t} \in \mathbb{R}^{pq}$  into the real line can be of arbitrary form. An obvious choice is the maximum of the absolute values of the standardized linear statistic

$$c_{\max}(\mathbf{t}, \mu, \Sigma) = \max_{k=1, \dots, pq} \left| \frac{(\mathbf{t} - \mu)_k}{\sqrt{(\Sigma)_{kk}}} \right|$$

utilizing the conditional expectation  $\mu$  and covariance matrix  $\Sigma$ . The application of a quadratic form  $c_{\text{quad}}(\mathbf{t}, \mu, \Sigma) = (\mathbf{t} - \mu) \Sigma^+ (\mathbf{t} - \mu)^\top$  is one alternative, although computationally more expensive because the Moore-Penrose inverse  $\Sigma^+$  of  $\Sigma$  is involved.

The type of test statistic to be used can be specified by means of the `ctree_control` function, for example

```
> ctree_control(teststat = "max")
```

uses  $c_{\max}$  and

```
> ctree_control(teststat = "quad")
```

takes  $c_{\text{quad}}$  (the default).

It is important to note that the test statistics  $c(\mathbf{t}_j, \mu_j, \Sigma_j), j = 1, \dots, m$ , cannot be directly compared in an unbiased way unless all of the covariates are measured at the same scale, i.e.,  $p_1 = p_j, j = 2, \dots, m$ . In order to allow for an unbiased variable selection we need to switch to the  $P$ -value scale because  $P$ -values for the conditional distribution of test statistics  $c(\mathbf{T}_j(\mathcal{L}_n, \mathbf{w}), \mu_j, \Sigma_j)$  can be directly compared among covariates measured at different scales. In step 1 of the generic algorithm we select the covariate with minimum  $P$ -value, i.e., the covariate  $X_{j^*}$  with  $j^* = \text{argmin}_{j=1, \dots, m} P_j$ , where

$$P_j = \mathbb{P}_{H_0^j}(c(\mathbf{T}_j(\mathcal{L}_n, \mathbf{w}), \mu_j, \Sigma_j) \geq c(\mathbf{t}_j, \mu_j, \Sigma_j) | S(\mathcal{L}_n, \mathbf{w}))$$

denotes the  $P$ -value of the conditional test for  $H_0^j$ . So far, we have only addressed testing each partial hypothesis  $H_0^j$ , which is sufficient for an unbiased variable selection. A global test for  $H_0$  required in step 1 can be constructed via an aggregation of the transformations  $g_j, j = 1, \dots, m$ , i.e., using a linear statistic of the form

$$\mathbf{T}(\mathcal{L}_n, \mathbf{w}) = \text{vec} \left( \sum_{i=1}^n w_i \left( g_1(X_{1i})^\top, \dots, g_m(X_{mi})^\top \right)^\top h(\mathbf{Y}_i, (\mathbf{Y}_1, \dots, \mathbf{Y}_n))^\top \right).$$

However, this approach is less attractive for learning samples with missing values. Universally applicable approaches are multiple test procedures based on  $P_1, \dots, P_m$ . Simple Bonferroni-adjusted  $P$ -values (the adjustment  $1 - (1 - P_j)^m$  is used), available via

```
> ctree_control(testtype = "Bonferroni")
```

or a min- $P$ -value resampling approach (Note: resampling is currently not implemented in `partykit::ctree`) are just examples and we refer to the multiple testing literature (e.g., [Westfall and Young 1993](#)) for more advanced methods. We reject  $H_0$  when the minimum of the adjusted  $P$ -values is less than a pre-specified nominal level  $\alpha$  and otherwise stop the algorithm. In this sense,  $\alpha$  may be seen as a unique parameter determining the size of the resulting trees.

## 4.2. Splitting criteria

Once we have selected a covariate in step 1 of the algorithm, the split itself can be established by any split criterion, including those established by [Breiman \*et al.\* \(1984\)](#) or [Shih \(1999\)](#). Instead of simple binary splits, multiway splits can be implemented as well, for example utilizing the work of [O'Brien \(2004\)](#). However, most splitting criteria are not applicable to response variables measured at arbitrary scales and we therefore utilize the permutation test framework described above to find the optimal binary split in one selected covariate  $X_{j^*}$  in step 2 of the generic algorithm. The goodness of a split is evaluated by two-sample linear statistics which are special cases of the linear statistic (1). For all possible subsets  $A$  of the sample space  $\mathcal{X}_{j^*}$  the linear statistic

$$\mathbf{T}_{j^*}^A(\mathcal{L}_n, \mathbf{w}) = \text{vec} \left( \sum_{i=1}^n w_i I(X_{j^*i} \in A) h(\mathbf{Y}_i, (\mathbf{Y}_1, \dots, \mathbf{Y}_n))^\top \right) \in \mathbb{R}^q$$

induces a two-sample statistic measuring the discrepancy between the samples  $\{\mathbf{Y}_i | w_i > 0 \text{ and } X_{ji} \in A; i = 1, \dots, n\}$  and  $\{\mathbf{Y}_i | w_i > 0 \text{ and } X_{ji} \notin A; i = 1, \dots, n\}$ . The conditional expectation  $\mu_{j^*}^A$  and covariance  $\Sigma_{j^*}^A$  can be computed by (2). The split  $A^*$  with a test statistic maximized over all possible subsets  $A$  is established:

$$A^* = \operatorname{argmax}_A c(\mathbf{t}_{j^*}^A, \mu_{j^*}^A, \Sigma_{j^*}^A). \quad (3)$$

The statistics  $c(\mathbf{t}_{j^*}^A, \mu_{j^*}^A, \Sigma_{j^*}^A)$  are available for each node with and can be used to depict a scatter plot of the covariate  $\mathcal{X}_{j^*}$  against the statistics (Note: this feature is currently not implemented in **partykit**).

Note that we do not need to compute the distribution of  $c(\mathbf{t}_{j^*}^A, \mu_{j^*}^A, \Sigma_{j^*}^A)$  in step 2. In order to anticipate pathological splits one can restrict the number of possible subsets that are evaluated, for example by introducing restrictions on the sample size or the sum of the case weights in each of the two groups of observations induced by a possible split. For example,

```
> ctree_control(minsplit = 20)
```

requires the sum of the weights in both the left and right daughter node to exceed the value of 20.

### 4.3. Missing values and surrogate splits

If an observation  $X_{ji}$  in covariate  $X_j$  is missing, we set the corresponding case weight  $w_i$  to zero for the computation of  $\mathbf{T}_j(\mathcal{L}_n, \mathbf{w})$  and, if we would like to split in  $X_j$ , in  $\mathbf{T}_j^A(\mathcal{L}_n, \mathbf{w})$  as well. Once a split  $A^*$  in  $X_j$  has been implemented, surrogate splits can be established by searching for a split leading to roughly the same division of the observations as the original split. One simply replaces the original response variable by a binary variable  $I(X_{ji} \in A^*)$  coding the split and proceeds as described in the previous part. The number of surrogate splits can be controlled using

```
> ctree_control(maxsurrogate = 3)
```

### 4.4. Fitting and inspecting a tree

For the sake of simplicity, we use a learning sample

```
> ls <- data.frame(y = gl(3, 50, labels = c("A", "B", "C")),
+                 x1 = rnorm(150) + rep(c(1, 0, 0), c(50, 50, 50)),
+                 x2 = runif(150))
```

in the following illustrations. In `partykit::ctree`, the dependency structure and the variables may be specified in a traditional formula based way

```
> library("partykit")
> ctree(y ~ x1 + x2, data = ls)
```

Case counts  $\mathbf{w}$  may be specified using the `weights` argument. Once we have fitted a conditional tree via

```
> plot(ct)
```

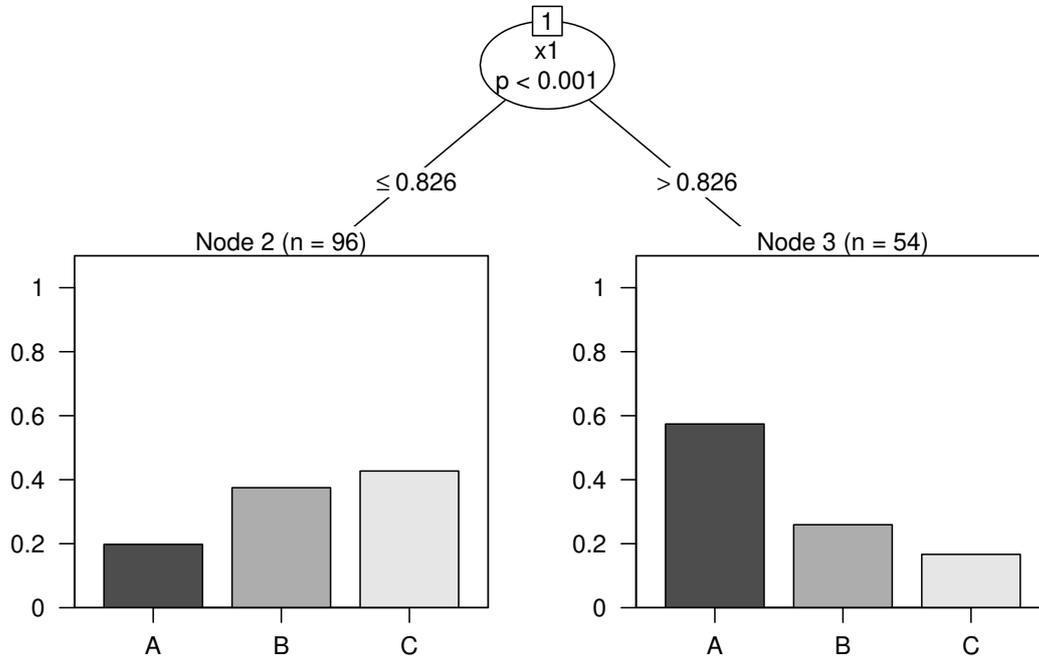

Figure 1: A graphical representation of a classification tree.

```
> ct <- ctree(y ~ x1 + x2, data = ls)
```

we can inspect the results via a `print` method

```
> ct
```

Model formula:

```
y ~ x1 + x2
```

Fitted party:

```
[1] root
| [2] x1 <= 0.82552: C (n = 96, err = 57.3%)
| [3] x1 > 0.82552: A (n = 54, err = 42.6%)
```

Number of inner nodes: 1

Number of terminal nodes: 2

or by looking at a graphical representation as in Figure 1.

Each node can be extracted by its node number, i.e., the root node is

```
> ct[1]
```

Model formula:

```
y ~ x1 + x2
```

Fitted party:

```
[1] root
| [2] x1 <= 0.82552: C (n = 96, err = 57.3%)
| [3] x1 > 0.82552: A (n = 54, err = 42.6%)
```

Number of inner nodes: 1

Number of terminal nodes: 2

This object is an object of class

```
> class(ct[1])
```

```
[1] "constparty" "party"
```

and we refer to the manual pages for a description of those elements. The `predict` function computes predictions in the space of the response variable, in our case a factor

```
> predict(ct, newdata = ls)
```

```
 1  2  3  4  5  6  7  8  9 10 11 12 13 14 15 16 17
A  A  A  A  C  A  C  A  C  C  A  A  C  A  A  A  A
18 19 20 21 22 23 24 25 26 27 28 29 30 31 32 33 34
C  A  C  A  A  A  C  A  A  A  C  C  A  A  C  A  A
35 36 37 38 39 40 41 42 43 44 45 46 47 48 49 50 51
C  A  A  C  C  C  A  A  C  C  C  C  A  A  A  A  A
52 53 54 55 56 57 58 59 60 61 62 63 64 65 66 67 68
A  C  C  C  C  A  C  C  A  C  C  C  C  C  C  A  A
69 70 71 72 73 74 75 76 77 78 79 80 81 82 83 84 85
A  A  A  C  C  A  C  A  C  C  C  C  C  C  C  C  C
86 87 88 89 90 91 92 93 94 95 96 97 98 99 100 101 102
C  C  C  A  C  A  C  A  C  C  C  C  C  C  C  C  A
103 104 105 106 107 108 109 110 111 112 113 114 115 116 117 118 119
C  C  C  A  C  C  A  C  C  C  C  C  C  C  A  C  C
120 121 122 123 124 125 126 127 128 129 130 131 132 133 134 135 136
C  C  C  C  C  C  C  C  C  C  C  C  C  C  C  C  C
137 138 139 140 141 142 143 144 145 146 147 148 149 150
C  A  C  C  C  C  A  C  C  A  C  A  C  A
Levels: A B C
```

When we are interested in properties of the conditional distribution of the response given the covariates, we use

```
> predict(ct, newdata = ls[c(1, 51, 101),], type = "prob")
```

|     | A         | B         | C         |
|-----|-----------|-----------|-----------|
| 1   | 0.5740741 | 0.2592593 | 0.1666667 |
| 51  | 0.5740741 | 0.2592593 | 0.1666667 |
| 101 | 0.1979167 | 0.3750000 | 0.4270833 |

which, in our case, is a data frame with conditional class probabilities. We can determine the node numbers of nodes some new observations are falling into by

```
> predict(ct, newdata = ls[c(1,51,101),], type = "node")
```

```
1 51 101
3 3 2
```

Finally, the `sctest` method can be used to extract the test statistics and  $p$ -values computed in each node. The function `sctest` is used because for the `mob` algorithm such a method (for structural change tests) is also provided. To make the generic available, the `strucchange` package needs to be loaded (otherwise `sctest.constparty` would have to be called directly).

```
> library("strucchange")
> sctest(ct)
```

```
$`1`
           x1           x2
statistic 2.299131e+01 4.0971294
p.value    2.034833e-05 0.2412193
```

```
$`2`
           x1           x2
statistic 2.6647107 4.3628130
p.value    0.4580906 0.2130228
```

```
$`3`
           x1           x2
statistic 2.1170497 2.8275567
p.value    0.5735483 0.4272879
```

Here, we see that `x1` leads to a significant test result in the root node and is hence used for splitting. In the kid nodes, no more significant results are found and hence splitting stops. For other data sets, other stopping criteria might also be relevant (e.g., the sample size restrictions `minsplit`, `minbucket`, etc.). In case, splitting stops due to these, the test results may also be `NULL`.

## 5. Examples

### 5.1. Univariate continuous or discrete regression

For a univariate numeric response  $\mathbf{Y} \in \mathbb{R}$ , the most natural influence function is the identity  $h(\mathbf{Y}_i, (\mathbf{Y}_1, \dots, \mathbf{Y}_n)) = \mathbf{Y}_i$ . In case some observations with extremely large or small values

have been observed, a ranking of the observations may be appropriate:  $h(\mathbf{Y}_i, (\mathbf{Y}_1, \dots, \mathbf{Y}_n)) = \sum_{k=1}^n w_k I(\mathbf{Y}_k \leq \mathbf{Y}_i)$  for  $i = 1, \dots, n$ . Numeric covariates can be handled by the identity transformation  $g_{ji}(x) = x$  (ranks are possible, too). Nominal covariates at levels  $1, \dots, K$  are represented by  $g_{ji}(k) = e_K(k)$ , the unit vector of length  $K$  with  $k$ th element being equal to one. Due to this flexibility, special test procedures like the Spearman test, the Wilcoxon-Mann-Whitney test or the Kruskal-Wallis test and permutation tests based on ANOVA statistics or correlation coefficients are covered by this framework. Splits obtained from (3) maximize the absolute value of the standardized difference between two means of the values of the influence functions. For prediction, one is usually interested in an estimate of the expectation of the response  $\mathbb{E}(\mathbf{Y}|\mathbf{X} = \mathbf{x})$  in each cell, an estimate can be obtained by

$$\hat{\mathbb{E}}(\mathbf{Y}|\mathbf{X} = \mathbf{x}) = \left( \sum_{i=1}^n w_i(\mathbf{x}) \right)^{-1} \sum_{i=1}^n w_i(\mathbf{x}) \mathbf{Y}_i.$$

## 5.2. Censored regression

The influence function  $h$  may be chosen as Logrank or Savage scores taking censoring into account and one can proceed as for univariate continuous regression. This is essentially the approach first published by Segal (1988). An alternative is the weighting scheme suggested by Molinaro, Dudoit, and van der Laan (2004). A weighted Kaplan-Meier curve for the case weights  $\mathbf{w}(\mathbf{x})$  can serve as prediction.

## 5.3. $J$ -class classification

The nominal response variable at levels  $1, \dots, J$  is handled by influence functions  $h(\mathbf{Y}_i, (\mathbf{Y}_1, \dots, \mathbf{Y}_n)) = e_J(\mathbf{Y}_i)$ . Note that for a nominal covariate  $X_j$  at levels  $1, \dots, K$  with  $g_{ji}(k) = e_K(k)$  the corresponding linear statistic  $\mathbf{T}_j$  is a vectorized contingency table. The conditional class probabilities can be estimated via

$$\hat{\mathbb{P}}(\mathbf{Y} = y|\mathbf{X} = \mathbf{x}) = \left( \sum_{i=1}^n w_i(\mathbf{x}) \right)^{-1} \sum_{i=1}^n w_i(\mathbf{x}) I(\mathbf{Y}_i = y), \quad y = 1, \dots, J.$$

## 5.4. Ordinal regression

Ordinal response variables measured at  $J$  levels, and ordinal covariates measured at  $K$  levels, are associated with score vectors  $\xi \in \mathbb{R}^J$  and  $\gamma \in \mathbb{R}^K$ , respectively. Those scores reflect the ‘distances’ between the levels: If the variable is derived from an underlying continuous variable, the scores can be chosen as the midpoints of the intervals defining the levels. The linear statistic is now a linear combination of the linear statistic  $\mathbf{T}_j$  of the form

$$\mathbf{M}\mathbf{T}_j(\mathcal{L}_n, \mathbf{w}) = \text{vec} \left( \sum_{i=1}^n w_i \gamma^\top g_j(X_{ji}) \left( \xi^\top h(\mathbf{Y}_i, (\mathbf{Y}_1, \dots, \mathbf{Y}_n)) \right)^\top \right)$$

with  $g_j(x) = e_K(x)$  and  $h(\mathbf{Y}_i, (\mathbf{Y}_1, \dots, \mathbf{Y}_n)) = e_J(\mathbf{Y}_i)$ . If both response and covariate are ordinal, the matrix of coefficients is given by the Kronecker product of both score vectors

$\mathbf{M} = \xi \otimes \gamma \in \mathbb{R}^{1,KJ}$ . In case the response is ordinal only, the matrix of coefficients  $\mathbf{M}$  is a block matrix

$$\mathbf{M} = \left( \begin{array}{ccc|ccc} \xi_1 & & 0 & & \xi_q & 0 \\ & \ddots & & \dots & & \\ 0 & & \xi_1 & & 0 & \xi_q \end{array} \right) \text{ or } \mathbf{M} = \text{diag}(\gamma)$$

when one covariate is ordered but the response is not. For both  $\mathbf{Y}$  and  $X_j$  being ordinal, the corresponding test is known as linear-by-linear association test (Agresti 2002). Scores can be supplied to `ctree` using the `scores` argument, see Section 6 for an example.

### 5.5. Multivariate regression

For multivariate responses, the influence function is a combination of influence functions appropriate for any of the univariate response variables discussed in the previous paragraphs, e.g., indicators for multiple binary responses (Zhang 1998; Noh, Song, and Park 2004), Log-rank or Savage scores for multiple failure times and the original observations or a rank transformation for multivariate regression (De'ath 2002).

## 6. Illustrations and applications

In this section, we present regression problems which illustrate the potential fields of application of the methodology. Conditional inference trees based on  $c_{\text{quad}}$ -type test statistics using the identity influence function for numeric responses and asymptotic  $\chi^2$  distribution are applied. For the stopping criterion a simple Bonferroni correction is used and we follow the usual convention by choosing the nominal level of the conditional independence tests as  $\alpha = 0.05$ .

### 6.1. Tree pipit abundance

```
> data("treepipit", package = "coin")
> tptree <- ctree(counts ~ ., data = treepipit)
```

The impact of certain environmental factors on the population density of the tree pipit *Anthus trivialis* is investigated by Müller and Hothorn (2004). The occurrence of tree pipits was recorded several times at  $n = 86$  stands which were established on a long environmental gradient. Among nine environmental factors, the covariate showing the largest association to the number of tree pipits is the canopy overstorey ( $P = 0.002$ ). Two groups of stands can be distinguished: Sunny stands with less than 40% canopy overstorey ( $n = 24$ ) show a significantly higher density of tree pipits compared to darker stands with more than 40% canopy overstorey ( $n = 62$ ). This result is important for management decisions in forestry enterprises: Cutting the overstorey with release of old oaks creates a perfect habitat for this indicator species of near natural forest environments.

### 6.2. Glaucoma and laser scanning images

```
> plot(tptree, terminal_panel = node_barplot)
```

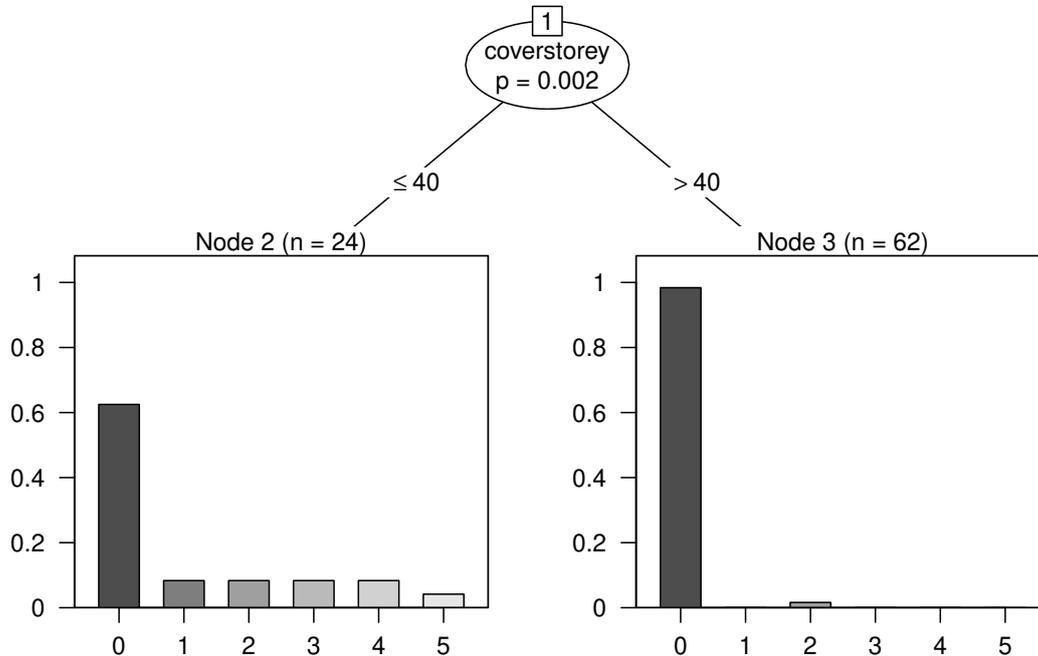

Figure 2: Conditional regression tree for the tree pipit data.

```
> data("GlaucomaM", package = "TH.data")
> gtree <- ctree(Class ~ ., data = GlaucomaM)
```

Laser scanning images taken from the eye background are expected to serve as the basis of an automated system for glaucoma diagnosis. Although prediction is more important in this application (Mardin, Hothorn, Peters, Jünemann, Nguyen, and Lausen 2003), a simple visualization of the regression relationship is useful for comparing the structures inherent in the learning sample with subject matter knowledge. For 98 patients and 98 controls, matched by age and gender, 62 covariates describing the eye morphology are available. The data is part of the **TH.data** package, <http://CRAN.R-project.org>). The first split in Figure 3 separates eyes with a volume above reference less than  $\text{mm}^3$  in the inferior part of the optic nerve head (**vari**). Observations with larger volume are mostly controls, a finding which corresponds to subject matter knowledge: The volume above reference measures the thickness of the nerve layer, expected to decrease with a glaucomatous damage of the optic nerve. Further separation is achieved by the volume above surface global (**vasg**) and the volume above reference in the temporal part of the optic nerve head (**vart**).

The plot in Figure 3 is generated by

```
> plot(gtree)
```

and shows the distribution of the classes in the terminal nodes. This distribution can be shown for the inner nodes as well, namely by specifying the appropriate panel generating

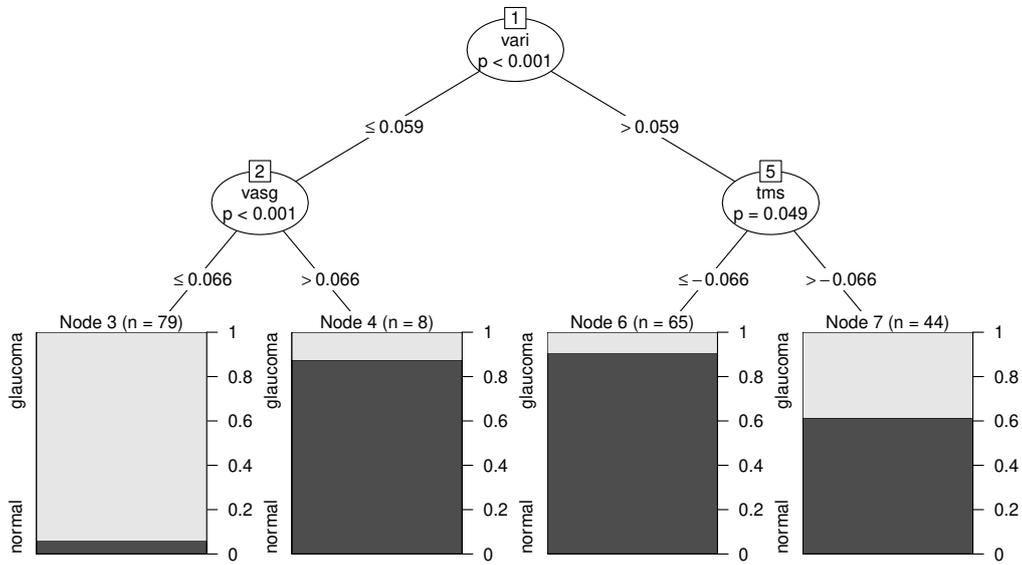

Figure 3: Conditional inference tree for the glaucoma data. For each inner node, the Bonferroni-adjusted  $P$ -values are given, the fraction of glaucomatous eyes is displayed for each terminal node.

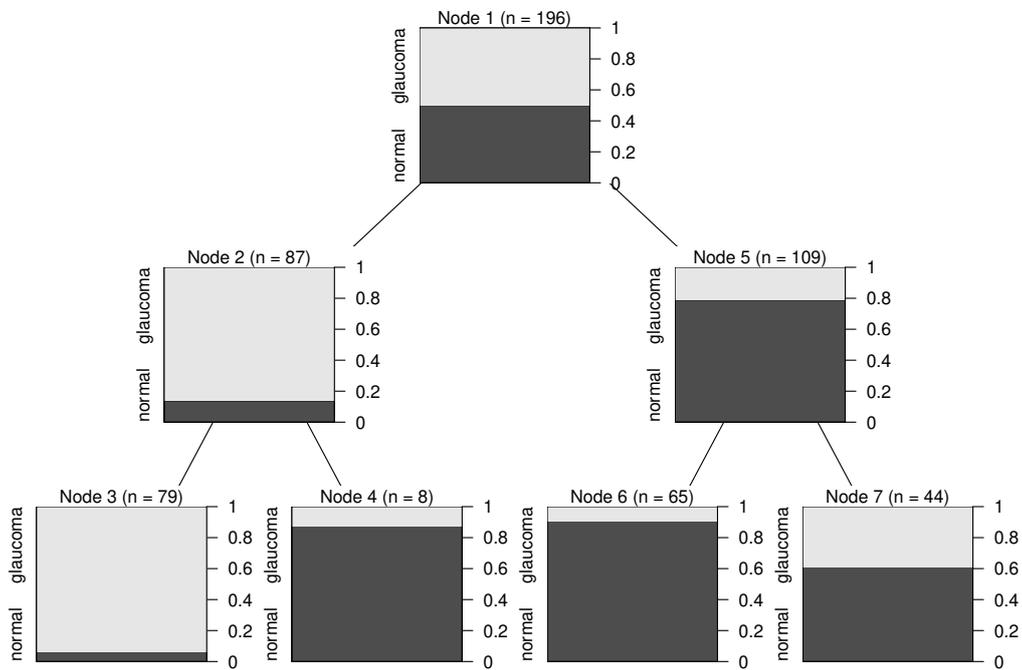

Figure 4: Conditional inference tree for the glaucoma data with the fraction of glaucomatous eyes displayed for both inner and terminal nodes.

```

> prob <- predict(gtree, type = "prob")[,1] +
+           runif(nrow(GlaucomaM), min = -0.01, max = 0.01)
> splitvar <- character_split(split_node(node_party(gtree)),
+                             data = data_party(gtree)$name)
> plot(GlaucomaM[[splitvar]], prob,
+       pch = as.numeric(GlaucomaM$Class), ylab = "Conditional Class Prob.",
+       xlab = splitvar)
> abline(v = split_node(node_party(gtree))$breaks, lty = 2)
> legend(0.15, 0.7, pch = 1:2, legend = levels(GlaucomaM$Class), bty = "n")

```

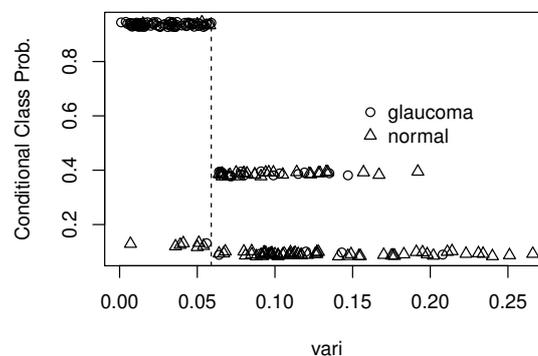

Figure 5: Estimated conditional class probabilities (slightly jittered) for the Glaucoma data depending on the first split variable. The vertical line denotes the first split point.

function (`node_barplot` in our case), see Figure 4.

```

> plot(gtree, inner_panel = node_barplot,
+       edge_panel = function(...) invisible(), tnex = 1)

```

The class predictions of the tree for the learning sample (and for new observations as well) can be computed using the `predict` function. A comparison with the true class memberships is done by

```

> table(predict(gtree), GlaucomaM$Class)

```

|          | glaucoma | normal |
|----------|----------|--------|
| glaucoma | 74       | 5      |
| normal   | 24       | 93     |

When we are interested in conditional class probabilities, the `predict(, type = "prob")` method must be used. A graphical representation is shown in Figure 5.

### 6.3. Node positive breast cancer

Recursive partitioning for censored responses has attracted a lot of interest (e.g., [Segal 1988](#); [LeBlanc and Crowley 1992](#)). Survival trees using  $P$ -value adjusted Logrank statistics are used

by Schumacher, Holländer, Schwarzer, and Sauerbrei (2001) for the evaluation of prognostic factors for the German Breast Cancer Study Group (GBSG2) data, a prospective controlled clinical trial on the treatment of node positive breast cancer patients. Here, we use Logrank scores as well. Complete data of seven prognostic factors of 686 women are used for prognostic modeling, the dataset is available within the **TH.data** package. The number of positive lymph nodes (`pnodes`) and the progesterone receptor (`progrec`) have been identified as prognostic factors in the survival tree analysis by Schumacher *et al.* (2001). Here, the binary variable coding whether a hormonal therapy was applied or not (`horTh`) additionally is part of the model depicted in Figure 6, which was fitted using the following code:

```
> data("GBSG2", package = "TH.data")
> library("survival")
> (stree <- ctree(Surv(time, cens) ~ ., data = GBSG2))
```

Model formula:

```
Surv(time, cens) ~ horTh + age + menostat + tsize + tgrade +
  pnodes + progrec + estrec
```

Fitted party:

```
[1] root
|   [2] pnodes <= 3
|   |   [3] horTh in no: 2093.000 (n = 248)
|   |   [4] horTh in yes: Inf (n = 128)
|   [5] pnodes > 3
|   |   [6] progrec <= 20: 624.000 (n = 144)
|   |   [7] progrec > 20: 1701.000 (n = 166)
```

Number of inner nodes: 3

Number of terminal nodes: 4

The estimated median survival time for new patients is less informative compared to the whole Kaplan-Meier curve estimated from the patients in the learning sample for each terminal node. We can compute those ‘predictions’ by means of the `treeresponse` method

```
> pn <- predict(stree, newdata = GBSG2[1:2,], type = "node")
> n <- predict(stree, type = "node")
> survfit(Surv(time, cens) ~ 1, data = GBSG2, subset = (n == pn[1]))
```

```
Call: survfit(formula = Surv(time, cens) ~ 1, data = GBSG2, subset = (n ==
  pn[1]))
```

| n   | events | median | 0.95LCL | 0.95UCL |
|-----|--------|--------|---------|---------|
| 248 | 88     | 2093   | 1814    | NA      |

```
> survfit(Surv(time, cens) ~ 1, data = GBSG2, subset = (n == pn[2]))
```

```
Call: survfit(formula = Surv(time, cens) ~ 1, data = GBSG2, subset = (n ==
  pn[2]))
```

```
> plot(stree)
```

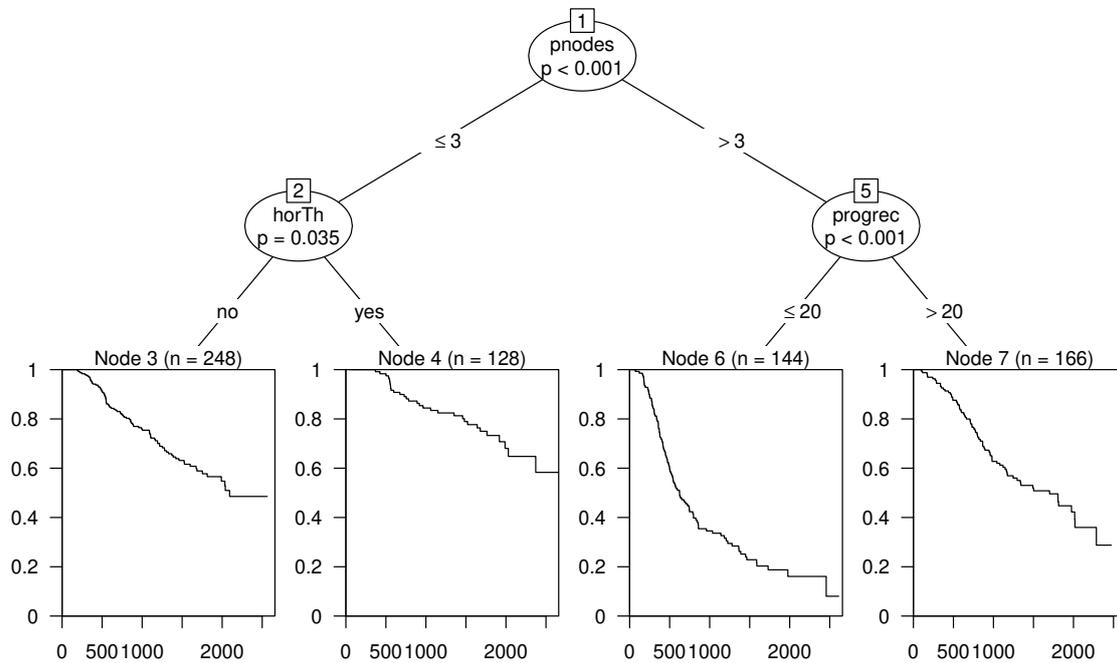

Figure 6: Tree-structured survival model for the GBSG2 data and the distribution of survival times in the terminal nodes. The median survival time is displayed in each terminal node of the tree.

| n   | events | median | 0.95LCL | 0.95UCL |
|-----|--------|--------|---------|---------|
| 166 | 77     | 1701   | 1174    | 2018    |

#### 6.4. Mammography experience

```
> data("mammoexp", package = "TH.data")
> mtree <- ctree(ME ~ ., data = mammoexp)
```

Ordinal response variables are common in investigations where the response is a subjective human interpretation. We use an example given by [Hosmer and Lemeshow \(2000\)](#), p. 264, studying the relationship between the mammography experience (never, within a year, over one year) and opinions about mammography expressed in questionnaires answered by  $n = 412$  women. The resulting partition based on scores  $\xi = (1, 2, 3)$  is given in Figure 7. Women who (strongly) agree with the question ‘You do not need a mammogram unless you develop symptoms’ seldomly have experienced a mammography. The variable `benefit` is a score with low values indicating a strong agreement with the benefits of the examination. For those women in (strong) disagreement with the first question above, low values of `benefit` identify persons being more likely to have experienced such an examination at all.

```
> plot(mtree)
```

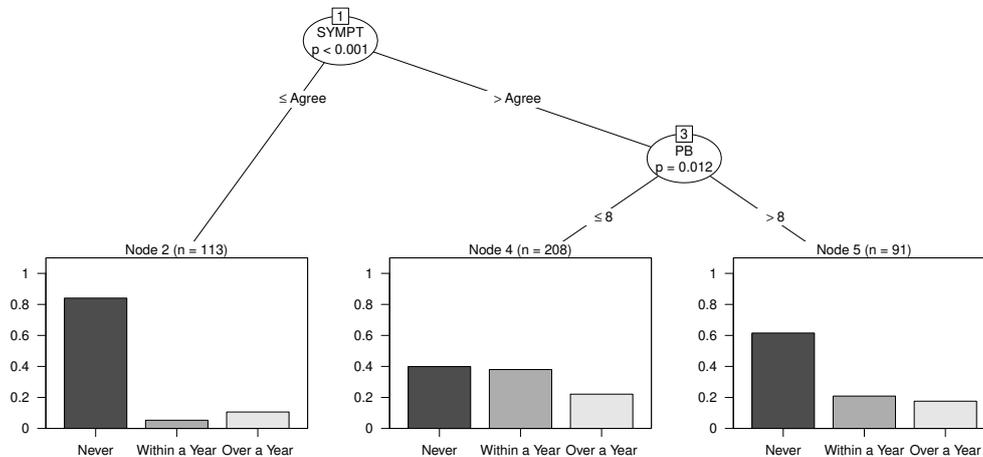

Figure 7: Ordinal regression for the mammography experience data with the fractions of (never, within a year, over one year) given in the nodes. No admissible split was found for node 5 because only 5 of 91 women reported a family history of breast cancer and the sample size restrictions would require more than 5 observations in each daughter node.

## 6.5. Hunting spiders

Finally, we take a closer look at a challenging dataset on animal abundance first reported by Van der Aart and Smeenk-Enserink (1975) and re-analyzed by De'ath (2002) using regression trees dealing with multivariate responses. The abundance of 12 hunting spider species is regressed on six environmental variables (`water`, `sand`, `moss`, `reft`, `twigs` and `herbs`) for  $n = 28$  observations. Because of the small sample size we allow for a split if at least 5 observations are element of a node. The prognostic factor `water` found by De'ath (2002) is confirmed by the model shown in Figures 8 and 9 which additionally identifies `reft`. The data are available in package `mvpart` (De'ath 2014).

```
> data("HuntingSpiders", package = "partykit")
> sptree <- ctree(arct.lute + pard.lugu + zora.spin + pard.nigr +
+   pard.pull + aulo.albi + troc.terr + alop.cune + pard.mont + alop.acce +
+   alop.fabr + arct.peri ~ herbs + reft + moss + sand + twigs + water,
+   data = HuntingSpiders, teststat = "max", minsplit = 5,
+   pargs = GenzBretz(abseps = .1, releps = .1))
```

## 7. Backward compatibility and novel functionality

`partykit::ctree` is a complete reimplementaion of `party::ctree`. The latter reference implementation is based on a monolithic C core and an S4-based R interface. The novel implementation of conditional inference trees in `partykit` is much more modular and was almost entirely written in R (package `partykit` does not contain any foreign language code as of version 1.2-0). Permutation tests are computed in the dedicated R add-on package `libcoin`.

```
> plot(sptree, terminal_panel = node_barplot)
```

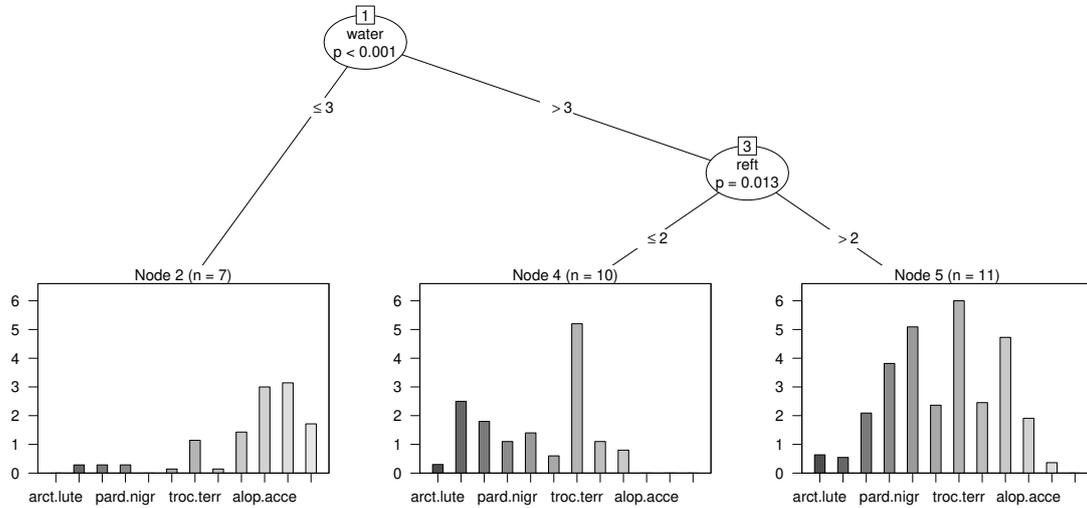

Figure 8: Regression tree for hunting spider abundance with bars for the mean of each response.

Nevertheless, both implementations will almost every time produce the same tree. There are, naturally, exceptions where ensuring backward-compatibility requires specific choices of hyper parameters in `partykit::ctree_control`. We will demonstrate how one can compute the same trees in `partykit` and `party` in this section. In addition, some novel features introduced in `partykit` 1.2-0 are described.

## 7.1. Regression

We use the `airquality` data from package `party` and fit a regression tree after removal of missing response values. There are missing values in one of the explanatory variables, so we ask for three surrogate splits to be set-up:

```
> data("airquality", package = "datasets")
> airq <- subset(airquality, !is.na(Ozone))
> (airct_party <- party::ctree(Ozone ~ ., data = airq,
+   controls = party::ctree_control(maxsurrogate = 3)))
```

Conditional inference tree with 5 terminal nodes

```
Response: Ozone
Inputs: Solar.R, Wind, Temp, Month, Day
Number of observations: 116
```

- 1) Temp <= 82; criterion = 1, statistic = 56.086
- 2) Wind <= 6.9; criterion = 0.998, statistic = 12.969
- 3)\* weights = 10

> plot(sptree)

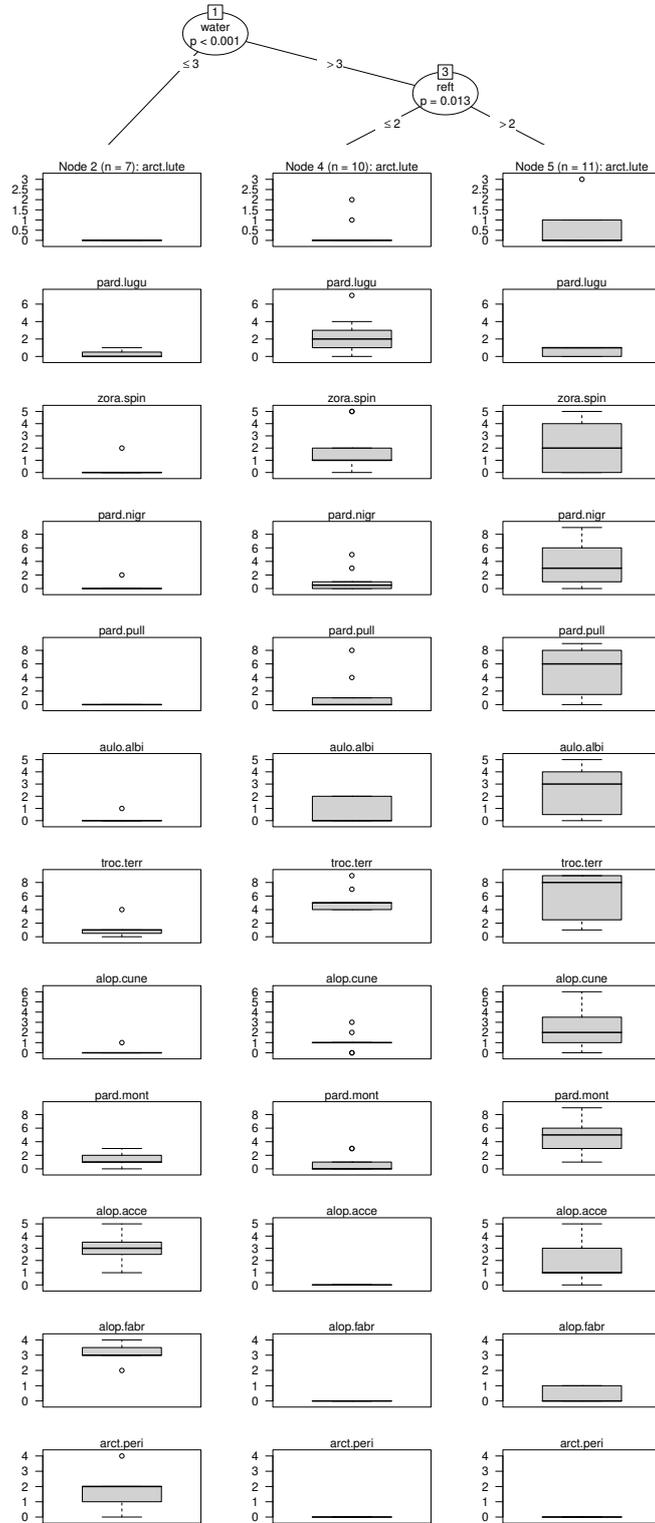

Figure 9: Regression tree for hunting spider abundance with boxplots for each response.

```

2) Wind > 6.9
  4) Temp <= 77; criterion = 0.997, statistic = 11.599
    5)* weights = 48
  4) Temp > 77
    6)* weights = 21
1) Temp > 82
  7) Wind <= 10.3; criterion = 0.997, statistic = 11.712
    8)* weights = 30
  7) Wind > 10.3
    9)* weights = 7

```

```
> mean((airq$Ozone - predict(airct_party))^2)
```

```
[1] 403.6668
```

For this specific example, the same call produces the same tree under both **party** and **partykit**. To ensure this also for other patterns of missingness, the `numsurrogate` flag needs to be set in order to restrict the evaluation of surrogate splits to numeric variables only (this is a restriction hard-coded in **party**):

```
> (airct_partykit <- partykit::ctree(Ozone ~ ., data = airq,
+   control = partykit::ctree_control(maxsurrogate = 3,
+   numsurrogate = TRUE)))
```

Model formula:

```
Ozone ~ Solar.R + Wind + Temp + Month + Day
```

Fitted party:

```
[1] root
| [2] Temp <= 82
| | [3] Wind <= 6.9: 55.600 (n = 10, err = 21946.4)
| | [4] Wind > 6.9
| | | [5] Temp <= 77: 18.479 (n = 48, err = 3956.0)
| | | [6] Temp > 77: 31.143 (n = 21, err = 4620.6)
| [7] Temp > 82
| | [8] Wind <= 10.3: 81.633 (n = 30, err = 15119.0)
| | [9] Wind > 10.3: 48.714 (n = 7, err = 1183.4)
```

Number of inner nodes: 4

Number of terminal nodes: 5

```
> mean((airq$Ozone - predict(airct_partykit))^2)
```

```
[1] 403.6668
```

```
> table(predict(airct_party, type = "node"),
+   predict(airct_partykit, type = "node"))
```

```

      3  5  6  8  9
3 10  0  0  0  0
5  0 48  0  0  0
6  0  0 21  0  0
8  0  0  0 30  0
9  0  0  0  0  7

> max(abs(predict(airct_party) - predict(airct_partykit)))

[1] 0

The results are identical as are the underlying test statistics:

> airct_party@tree$criterion

$statistic
      Solar.R      Wind      Temp      Month      Day
13.34761286 41.61369618 56.08632426  3.11265955  0.02011554

$criterion
      Solar.R      Wind      Temp      Month      Day
9.987069e-01 1.000000e+00 1.000000e+00 6.674119e-01 1.824984e-05

$maxcriterion
[1] 1

> info_node(node_party(airct_partykit))

$criterion
      Solar.R      Wind      Temp      Month
statistic 13.347612859 4.161370e+01 5.608632e+01 3.1126596
p.value   0.001293090 5.560572e-10 3.467894e-13 0.3325881
criterion -0.001293926 -5.560572e-10 -3.467894e-13 -0.4043478
      Day
statistic 0.02011554
p.value   0.99998175
criterion -10.91135399

$p.value
      Temp
3.467894e-13

$unweighted
[1] TRUE

$nobs
[1] 116

```

`partykit` has a nicer way of presenting the variable selection test statistics on the scale of the statistics and the  $p$ -values. In addition, the criterion to be maximised (here:  $\log(1-p\text{-value})$ ) is given.

## 7.2. Classification

For classification tasks with more than two classes, the default in `party` is a maximum-type test statistic on the multidimensional test statistic when computing splits. `partykit` employs a quadratic test statistic by default, because it was found to produce better splits empirically. One can switch-back to the old behaviour using the `splitstat` argument:

```
> (irisct_party <- party::ctree(Species ~ ., data = iris))

      Conditional inference tree with 4 terminal nodes

Response: Species
Inputs:  Sepal.Length, Sepal.Width, Petal.Length, Petal.Width
Number of observations: 150

1) Petal.Length <= 1.9; criterion = 1, statistic = 140.264
   2)* weights = 50
1) Petal.Length > 1.9
   3) Petal.Width <= 1.7; criterion = 1, statistic = 67.894
     4) Petal.Length <= 4.8; criterion = 0.999, statistic = 13.865
       5)* weights = 46
       4) Petal.Length > 4.8
         6)* weights = 8
       3) Petal.Width > 1.7
         7)* weights = 46

> (irisct_partykit <- partykit::ctree(Species ~ ., data = iris,
+ control = partykit::ctree_control(splitstat = "maximum"))

Model formula:
Species ~ Sepal.Length + Sepal.Width + Petal.Length + Petal.Width

Fitted party:
[1] root
| [2] Petal.Length <= 1.9: setosa (n = 50, err = 0.0%)
| [3] Petal.Length > 1.9
| | [4] Petal.Width <= 1.7
| | | [5] Petal.Length <= 4.8: versicolor (n = 46, err = 2.2%)
| | | [6] Petal.Length > 4.8: versicolor (n = 8, err = 50.0%)
| | [7] Petal.Width > 1.7: virginica (n = 46, err = 2.2%)

Number of inner nodes: 3
Number of terminal nodes: 4
```

```
> table(predict(irisct_party, type = "node"),
+       predict(irisct_partykit, type = "node"))

      2  5  6  7
2  50  0  0  0
5   0 46  0  0
6   0  0  8  0
7   0  0  0 46
```

The interface for computing conditional class probabilities changed from

```
> tr_party <- treeresponse(irisct_party, newdata = iris)
```

to

```
> tr_partykit <- predict(irisct_partykit, type = "prob",
+                       newdata = iris)
> max(abs(do.call("rbind", tr_party) - tr_partykit))
```

```
[1] 0
```

leading to identical results. For ordinal regression, the conditional class probabilities can be computed in the very same way:

```
> ### ordinal regression
> data("mammoexp", package = "TH.data")
> (mammoct_party <- party::ctree(ME ~ ., data = mammoexp))
```

```
      Conditional inference tree with 3 terminal nodes
```

```
Response: ME
Inputs:  SYMPT, PB, HIST, BSE, DECT
Number of observations: 412
```

```
1) SYMPT <= Agree; criterion = 1, statistic = 29.933
  2)* weights = 113
1) SYMPT > Agree
  3) PB <= 8; criterion = 0.988, statistic = 9.17
  4)* weights = 208
  3) PB > 8
  5)* weights = 91
```

```
> ### estimated class probabilities
> tr_party <- treeresponse(mammoct_party, newdata = mammoexp)
> (mammoct_partykit <- partykit::ctree(ME ~ ., data = mammoexp))
```

Model formula:

```
ME ~ SYMPT + PB + HIST + BSE + DECT
```

Fitted party:

```
[1] root
| [2] SYMPT <= Agree: Never (n = 113, err = 15.9%)
| [3] SYMPT > Agree
| | [4] PB <= 8: Never (n = 208, err = 60.1%)
| | [5] PB > 8: Never (n = 91, err = 38.5%)
```

Number of inner nodes: 2

Number of terminal nodes: 3

```
> ### estimated class probabilities
> tr_partykit <- predict(mammocct_partykit, newdata = mammoexp, type = "prob")
> max(abs(do.call("rbind", tr_party) - tr_partykit))
```

```
[1] 0
```

### 7.3. Survival Analysis

Like in classification analysis, the `treeresponse` function from package `party` was replaced by the `predict` function with argument `type = "prob"` in `partykit`. The default survival trees are identical:

```
> data("GBSG2", package = "TH.data")
> (GBSG2ct_party <- party::ctree(Surv(time, cens) ~ ., data = GBSG2))
```

Conditional inference tree with 4 terminal nodes

Response: Surv(time, cens)

Inputs: horTh, age, menostat, tsize, tgrade, pnodes, progrec, estrec

Number of observations: 686

```
1) pnodes <= 3; criterion = 1, statistic = 56.156
  2) horTh == {yes}; criterion = 0.965, statistic = 8.113
    3)* weights = 128
  2) horTh == {no}
    4)* weights = 248
1) pnodes > 3
  5) progrec <= 20; criterion = 0.999, statistic = 14.941
    6)* weights = 144
  5) progrec > 20
    7)* weights = 166
```

```
> (GBSG2ct_partykit <- partykit::ctree(Surv(time, cens) ~ ., data = GBSG2))
```

Model formula:

```
Surv(time, cens) ~ horTh + age + menostat + tsize + tgrade +
  pnodes + progrec + estrec
```

Fitted party:

```
[1] root
| [2] pnodes <= 3
| | [3] horTh in no: 2093.000 (n = 248)
| | [4] horTh in yes: Inf (n = 128)
| [5] pnodes > 3
| | [6] progrec <= 20: 624.000 (n = 144)
| | [7] progrec > 20: 1701.000 (n = 166)
```

Number of inner nodes: 3

Number of terminal nodes: 4

as are the conditional Kaplan-Meier estimators

```
> tr_party <- treeresponse(GBSG2ct_party, newdata = GBSG2)
> tr_partykit <- predict(GBSG2ct_partykit, newdata = GBSG2, type = "prob")
> all.equal(lapply(tr_party, function(x) unclass(x)[!(names(x) %in% "call")])),
+ lapply(tr_partykit, function(x) unclass(x)[!(names(x) %in% "call")])),
+ check.names = FALSE)
```

```
[1] TRUE
```

## 7.4. New Features

**partykit** comes with additional arguments in `ctree_control` allowing a more detailed control over the tree growing.

**alpha** : The user can optionally change the default nominal level of  $\alpha = 0.05$ ; `mincriterion` is updated to  $1 - \alpha$  and `logmincriterion` is then  $\log(1 - \alpha)$ . The latter allows variable selection on the scale of  $\log(1 - p\text{-value})$ :

```
> (airct_partykit_1 <- partykit::ctree(Ozone ~ ., data = airq,
+   control = partykit::ctree_control(maxsurrogate = 3, alpha = 0.001,
+   numsurrogate = FALSE)))
```

Model formula:

```
Ozone ~ Solar.R + Wind + Temp + Month + Day
```

Fitted party:

```
[1] root
| [2] Temp <= 82: 26.544 (n = 79, err = 42531.6)
| [3] Temp > 82: 75.405 (n = 37, err = 22452.9)
```

```
Number of inner nodes: 1
Number of terminal nodes: 2
```

```
> depth(airct_partykit_1)
```

```
[1] 1
```

```
> mean((airq$Ozone - predict(airct_partykit_1))^2)
```

```
[1] 560.2113
```

Lower values of  $\alpha$  lead to smaller trees.

**splittest** : This enables the computation of  $p$ -values for maximally selected statistics for variable selection. The default test statistic is not particularly powerful against cutpoint-alternatives but much faster to compute. Currently,  $p$ -value approximations are not available, so one has to rely on resampling for  $p$ -value estimation

```
> (airct_partykit <- partykit::ctree(Ozone ~ ., data = airq,
+   control = partykit::ctree_control(maxsurrogate = 3, splittest = TRUE,
+   testtype = "MonteCarlo")))
```

Model formula:

```
Ozone ~ Solar.R + Wind + Temp + Month + Day
```

Fitted party:

```
[1] root
|   [2] Temp <= 82
|   |   [3] Wind <= 6.9: 55.600 (n = 10, err = 21946.4)
|   |   [4] Wind > 6.9
|   |   |   [5] Temp <= 77
|   |   |   |   [6] Solar.R <= 78: 12.533 (n = 15, err = 723.7)
|   |   |   |   [7] Solar.R > 78: 21.182 (n = 33, err = 2460.9)
|   |   |   [8] Temp > 77
|   |   |   |   [9] Solar.R <= 148: 20.000 (n = 7, err = 652.0)
|   |   |   |   [10] Solar.R > 148: 36.714 (n = 14, err = 2664.9)
|   [11] Temp > 82
|   |   [12] Temp <= 87
|   |   |   [13] Wind <= 8.6: 72.308 (n = 13, err = 8176.8)
|   |   |   [14] Wind > 8.6: 45.571 (n = 7, err = 617.7)
|   |   [15] Temp > 87: 90.059 (n = 17, err = 3652.9)
```

```
Number of inner nodes: 7
Number of terminal nodes: 8
```

**saveinfo** : Reduces the memory footprint by not storing test results as part of the tree. The core information about trees is then roughly half the size needed by **party**.

`nmax` : Restricts the number of possible cutpoints to `nmax`, basically by treating all explanatory variables as ordered factors defined at quantiles of underlying numeric variables. This is mainly implemented in package **libcoin**. For the standard `ctree`, it is only appropriate to use in classification problems, where it can lead to substantial speed-ups:

```
> (irisct_partykit_1 <- partykit::ctree(Species ~ ., data = iris,
+ control = partykit::ctree_control(splitstat = "maximum", nmax = 25)))
```

Model formula:

```
Species ~ Sepal.Length + Sepal.Width + Petal.Length + Petal.Width
```

Fitted party:

```
[1] root
| [2] Petal.Width <= 0.6: setosa (n = 50, err = 0.0%)
| [3] Petal.Width > 0.6
| | [4] Petal.Width <= 1.7
| | | [5] Petal.Length <= 4.8: versicolor (n = 46, err = 2.2%)
| | | [6] Petal.Length > 4.8: versicolor (n = 8, err = 50.0%)
| | [7] Petal.Width > 1.7: virginica (n = 46, err = 2.2%)
```

Number of inner nodes: 3

Number of terminal nodes: 4

```
> table(predict(irisct_partykit), predict(irisct_partykit_1))
```

|            | setosa | versicolor | virginica |
|------------|--------|------------|-----------|
| setosa     | 50     | 0          | 0         |
| versicolor | 0      | 54         | 0         |
| virginica  | 0      | 0          | 46        |

`multiway` : Implements multiway splits in unordered factors, each level defines a corresponding daughter node:

```
> GBSG2$tgrade <- factor(GBSG2$tgrade, ordered = FALSE)
> (GBSG2ct_partykit <- partykit::ctree(Surv(time, cens) ~ tgrade,
+ data = GBSG2, control = partykit::ctree_control(multiway = TRUE,
+ alpha = .5)))
```

Model formula:

```
Surv(time, cens) ~ tgrade
```

Fitted party:

```
[1] root
| [2] tgrade in I: Inf (n = 81)
| [3] tgrade in II: 1730.000 (n = 444)
| [4] tgrade in III: 1337.000 (n = 161)
```

Number of inner nodes: 1

Number of terminal nodes: 3

`majority = FALSE` : enables random assignment of non-splitable observations to daughter nodes preserving the node distribution. With `majority = TRUE`, these observations go with the majority (the only available behaviour of `in party::ctree`).

Two arguments of `ctree` are also interesting. The novel `cluster` argument allows conditional inference trees to be fitted to (simple forms of) correlated observations. For each cluster, the variance of the test statistics used for variable selection and also splitting is computed separately, leading to stratified permutation tests (in the sense that only observations within clusters are permuted). For example, we can cluster the data in the `airquality` dataset by month to be used as cluster variable:

```
> airq$month <- factor(airq$Month)
> (airct_partykit_3 <- partykit::ctree(Ozone ~ Solar.R + Wind + Temp, data = airq,
+ cluster = month, control = partykit::ctree_control(maxsurrogate = 3)))
```

Model formula:

```
Ozone ~ Solar.R + Wind + Temp
```

Fitted party:

```
[1] root
| [2] Temp <= 82
| | [3] Temp <= 76: 18.250 (n = 48, err = 4199.0)
| | [4] Temp > 76
| | | [5] Wind <= 6.9: 71.857 (n = 7, err = 15510.9)
| | | [6] Wind > 6.9
| | | | [7] Temp <= 81: 32.412 (n = 17, err = 4204.1)
| | | | [8] Temp > 81: 23.857 (n = 7, err = 306.9)
| [9] Temp > 82
| | [10] Wind <= 10.3: 81.633 (n = 30, err = 15119.0)
| | [11] Wind > 10.3: 48.714 (n = 7, err = 1183.4)
```

Number of inner nodes: 5

Number of terminal nodes: 6

```
> info_node(node_party(airct_partykit_3))
```

\$criterion

|           | Solar.R       | Wind          | Temp          |
|-----------|---------------|---------------|---------------|
| statistic | 14.4805065501 | 3.299881e+01  | 4.783766e+01  |
| p.value   | 0.0004247923  | 2.766464e-08  | 1.389038e-11  |
| criterion | -0.0004248826 | -2.766464e-08 | -1.389038e-11 |

\$p.value

| Temp         |
|--------------|
| 1.389038e-11 |

\$unweighted

```
[1] TRUE
```

```
$nobs
```

```
[1] 116
```

```
> mean((airq$Ozone - predict(airct_partykit_3))^2)
```

```
[1] 349.3382
```

This reduces the number of partitioning variables and makes multiplicity adjustment less costly.

The `ytrafo` argument has been made more general. **party** is not able to update influence functions  $h$  within nodes. With the novel formula-based interface, users can create influence functions which are newly evaluated in each node. The following example illustrates how one can compute a survival tree with updated logrank scores:

```
> ### with weight-dependent log-rank scores
> ### log-rank trafo for observations in this node only (= weights > 0)
> h <- function(y, x, start = NULL, weights, offset, estfun = TRUE, object = FALSE, ...) {
+   if (is.null(weights)) weights <- rep(1, NROW(y))
+   s <- logrank_trafo(y[weights > 0, , drop = FALSE])
+   r <- rep(0, length(weights))
+   r[weights > 0] <- s
+   list(estfun = matrix(as.double(r), ncol = 1), converged = TRUE, unweighted = TRUE)
+ }
> partykit::ctree(Surv(time, cens) ~ ., data = GBSG2, ytrafo = h)
```

Model formula:

```
Surv(time, cens) ~ horTh + age + menostat + tsize + tgrade +
  pnodes + progrec + estrec
```

Fitted party:

```
[1] root
| [2] pnodes <= 3
| | [3] horTh in no: 2093.000 (n = 248)
| | [4] horTh in yes: Inf (n = 128)
| [5] pnodes > 3
| | [6] progrec <= 20: 624.000 (n = 144)
| | [7] progrec > 20: 1701.000 (n = 166)
```

```
Number of inner nodes: 3
```

```
Number of terminal nodes: 4
```

The results are usually not very sensitive to (simple) updated influence functions. However, when one uses score functions of more complex models as influence functions (similar to the `mob` family of trees), it is necessary to refit models in each node. For example, we are

interested in a normal linear model for ozone concentration given temperature; both the intercept and the regression coefficient for temperature shall vary across nodes of a tree. Such a “permutation-based” MOB, here taking clusters into account, can be set-up using

```
> ### normal varying intercept / varying coefficient model (aka "mob")
> h <- function(y, x, start = NULL, weights = NULL, offset = NULL, cluster = NULL, ...)
+   glm(y ~ 0 + x, family = gaussian(), start = start, weights = weights, ...)
> (airct_partykit_4 <- partykit::ctree(Ozone ~ Temp | Solar.R + Wind,
+   data = airq, cluster = month, ytrafo = h,
+   control = partykit::ctree_control(maxsurrogate = 3)))
```

Model formula:

```
Ozone ~ Temp + (Solar.R + Wind)
```

Fitted party:

```
[1] root
| [2] Wind <= 5.7: 98.692 (n = 13, err = 11584.8)
| [3] Wind > 5.7
| | [4] Wind <= 8
| | | [5] Wind <= 6.9: 55.286 (n = 14, err = 11330.9)
| | | [6] Wind > 6.9: 50.824 (n = 17, err = 15400.5)
| | [7] Wind > 8: 27.306 (n = 72, err = 25705.3)
```

Number of inner nodes: 3

Number of terminal nodes: 4

```
> airq$node <- factor(predict(airct_partykit_4, type = "node"))
> summary(m <- glm(Ozone ~ node + node:Temp - 1, data = airq))
```

Call:

```
glm(formula = Ozone ~ node + node:Temp - 1, data = airq)
```

Deviance Residuals:

|  | Min     | 1Q      | Median | 3Q     | Max    |
|--|---------|---------|--------|--------|--------|
|  | -45.801 | -11.208 | -1.049 | 10.903 | 53.615 |

Coefficients:

|            | Estimate  | Std. Error | t value | Pr(> t ) |     |
|------------|-----------|------------|---------|----------|-----|
| node2      | 300.0527  | 93.4828    | 3.210   | 0.001750 | **  |
| node5      | -217.3416 | 51.3970    | -4.229  | 4.94e-05 | *** |
| node6      | -178.9333 | 58.1093    | -3.079  | 0.002632 | **  |
| node7      | -82.2722  | 17.9951    | -4.572  | 1.29e-05 | *** |
| node2:Temp | -2.2922   | 1.0626     | -2.157  | 0.033214 | *   |
| node5:Temp | 3.2989    | 0.6191     | 5.328   | 5.47e-07 | *** |
| node6:Temp | 2.8059    | 0.7076     | 3.965   | 0.000132 | *** |
| node7:Temp | 1.4769    | 0.2408     | 6.133   | 1.45e-08 | *** |

---

Signif. codes: 0 '\*\*\*' 0.001 '\*\*' 0.01 '\*' 0.05 '.' 0.1 ' ' 1

(Dispersion parameter for gaussian family taken to be 329.3685)

Null deviance: 331029 on 116 degrees of freedom  
 Residual deviance: 35572 on 108 degrees of freedom  
 AIC: 1011.4

Number of Fisher Scoring iterations: 2

```
> mean((predict(m) - airq$Ozone)^2)
```

```
[1] 306.6534
```

Both intercept and effect of temperature change considerably between nodes. The corresponding MOB can be fitted using

```
> airq_lmtree <- partykit::lmtree(Ozone ~ Temp | Solar.R + Wind,
+                               data = airq, cluster = month)
> info_node(node_party(airq_lmtree))
```

```
$criterion
      Solar.R      Wind
statistic 8.5987001 19.559486324
p.value   0.2818551 0.002658029
criterion -0.3310839 -0.002661567
```

```
$p.value
      Wind
0.002658029
```

```
$coefficients
(Intercept)      Temp
-146.995491    2.428703
```

```
$objfun
[1] 64109.89
```

```
$object
```

```
Call:
lm(formula = Ozone ~ Temp)
```

```
Coefficients:
(Intercept)      Temp
-146.995      2.429
```

```
$converged
```

```
[1] TRUE
```

```
$nobs
```

```
[1] 116
```

```
> mean((predict(airq_lmtree, newdata = airq) - airq$Ozone)^2)
```

```
[1] 443.9422
```

The  $p$ -values in the root node are similar but the two procedures find different splits. `mob` (and therefore `lmtree`) directly search for splits by optimising the objective function for all possible splits whereas `ctree` only works with the score functions.

Argument `xtrafo` allowing the user to change the transformations  $g_j$  of the covariates was removed from the user interface.

## References

- Agresti A (2002). *Categorical Data Analysis*. 2nd edition. John Wiley & Sons, Hoboken.
- Breiman L, Friedman JH, Olshen RA, Stone CJ (1984). *Classification and Regression Trees*. Wadsworth, California.
- De'ath G (2002). "Multivariate Regression Trees: A New Technique for Modeling Species-Environment Relationships." *Ecology*, **83**(4), 1105–1117.
- De'ath G (2014). *mvpart: Multivariate Partitioning*. R package version 1.6-2, URL <http://CRAN.R-project.org/package=mvpart>.
- Hosmer DW, Lemeshow S (2000). *Applied Logistic Regression*. 2nd edition. John Wiley & Sons, New York.
- Hothorn T, Hornik K, Zeileis A (2006). "Unbiased Recursive Partitioning: A Conditional Inference Framework." *Journal of Computational and Graphical Statistics*, **15**(3), 651–674. doi:10.1198/106186006X133933.
- LeBlanc M, Crowley J (1992). "Relative Risk Trees for Censored Survival Data." *Biometrics*, **48**, 411–425.
- Mardin CY, Hothorn T, Peters A, Jünemann AG, Nguyen NX, Lausen B (2003). "New Glaucoma Classification Method Based on Standard HRT Parameters by Bagging Classification Trees." *Journal of Glaucoma*, **12**(4), 340–346.
- Mingers J (1987). "Expert Systems – Rule Induction with Statistical Data." *Journal of the Operations Research Society*, **38**(1), 39–47.

- Molinaro AM, Dudoit S, van der Laan MJ (2004). “Tree-Based Multivariate Regression and Density Estimation with Right-Censored Data.” *Journal of Multivariate Analysis*, **90**(1), 154–177.
- Müller J, Hothorn T (2004). “Maximally Selected Two-Sample Statistics as a new Tool for the Identification and Assessment of Habitat Factors with an Application to Breeding Bird Communities in Oak Forests.” *European Journal of Forest Research*, **123**, 218–228.
- Noh HG, Song MS, Park SH (2004). “An Unbiased Method for Constructing Multilabel Classification Trees.” *Computational Statistics & Data Analysis*, **47**(1), 149–164.
- O’Brien SM (2004). “Cutpoint Selection for Categorizing a Continuous Predictor.” *Biometrics*, **60**, 504–509.
- Quinlan JR (1993). *C4.5: Programs for Machine Learning*. Morgan Kaufmann Publishers, San Mateo.
- Schumacher M, Holländer N, Schwarzer G, Sauerbrei W (2001). “Prognostic Factor Studies.” In J Crowley (ed.), *Statistics in Oncology*, pp. 321–378. Marcel Dekker, New York.
- Segal MR (1988). “Regression Trees for Censored Data.” *Biometrics*, **44**, 35–47.
- Shih Y (1999). “Families of Splitting Criteria for Classification Trees.” *Statistics and Computing*, **9**, 309–315.
- Strasser H, Weber C (1999). “On the Asymptotic Theory of Permutation Statistics.” *Mathematical Methods of Statistics*, **8**, 220–250.
- Van der Aart PJ, Smeenk-Enserink N (1975). “Correlations between Distributions of Hunting Spiders (Lycosidae, Ctenidae) and Environment Characteristics in a Dune Area.” *Netherlands Journal of Zoology*, **25**, 1–45.
- Westfall PH, Young SS (1993). *Resampling-Based Multiple Testing*. John Wiley & Sons, New York.
- White AP, Liu WZ (1994). “Bias in Information-Based Measures in Decision Tree Induction.” *Machine Learning*, **15**, 321–329.
- Zhang H (1998). “Classification Trees for Multiple Binary Responses.” *Journal of the American Statistical Association*, **93**, 180–193.

**Affiliation:**

Torsten Hothorn  
Institut für Epidemiologie, Biostatistik und Prävention  
Universität Zürich  
Hirschengraben 84  
CH-8001 Zürich, Switzerland  
E-mail: [Torsten.Hothorn@R-project.org](mailto:Torsten.Hothorn@R-project.org)  
URL: <http://user.math.uzh.ch/hothorn/>

Kurt Hornik  
Institute for Statistics and Mathematics  
WU Wirtschaftsuniversität Wien  
Welthandelsplatz 1  
1020 Wien, Austria  
E-mail: [Kurt.Hornik@R-project.org](mailto:Kurt.Hornik@R-project.org)  
URL: <http://statmath.wu.ac.at/~hornik/>

Achim Zeileis  
Department of Statistics  
Faculty of Economics and Statistics  
Universität Innsbruck  
Universitätsstr. 15  
6020 Innsbruck, Austria  
E-mail: [Achim.Zeileis@R-project.org](mailto:Achim.Zeileis@R-project.org)  
URL: <http://eeecon.uibk.ac.at/~zeileis/>
