# Supplementary material for: The Power of Unbiased Recursive Partitioning: A Unifying View of CTree, MOB, and GUIDE
Source: arXiv:1906.10179 ancillary file (2019-06-24)
Supplement: Supplementary file 3 [file mob.pdf]

# Parties, Models, Mobsters: A New Implementation of Model-Based Recursive Partitioning in R

Achim Zeileis  
Universität Innsbruck

Torsten Hothorn  
Universität Zürich

---

## Abstract

MOB is a generic algorithm for model-based recursive partitioning (Zeileis, Hothorn, and Hornik 2008). Rather than fitting one global model to a dataset, it estimates local models on subsets of data that are “learned” by recursively partitioning. It proceeds in the following way: (1) fit a parametric model to a data set, (2) test for parameter instability over a set of partitioning variables, (3) if there is some overall parameter instability, split the model with respect to the variable associated with the highest instability, (4) repeat the procedure in each of the resulting subsamples. It is discussed how these steps of the conceptual algorithm are translated into computational tools in an object-oriented manner, allowing the user to plug in various types of parametric models. For representing the resulting trees, the R package **partykit** is employed and extended with generic infrastructure for recursive partitions where nodes are associated with statistical models. Compared to the previously available implementation in the **party** package, the new implementation supports more inference options, is easier to extend to new models, and provides more convenience features.

*Keywords:* parametric models, object-orientation, recursive partitioning.

---

## 1. Overview

To implement the model-based recursive partitioning (MOB) algorithm of Zeileis *et al.* (2008) in software, infrastructure for three aspects is required: (1) statistical “*models*”, (2) recursive “*party*”tions, and (3) “*mobsters*” carrying out the MOB algorithm.

Along with Zeileis *et al.* (2008), an implementation of all three steps was provided in the **party** package (Hothorn, Hornik, Strobl, and Zeileis 2015) for the R system for statistical computing (R Core Team 2013). This provided one very flexible `mob()` function combining **party**’s S4 classes for representing trees with binary splits and the S4 model wrapper functions from **modeltools** (Hothorn, Leisch, and Zeileis 2013). However, while this supported many applications of interest, it was somewhat limited in several directions: (1) The S4 wrappers for the models were somewhat cumbersome to set up. (2) The tree infrastructure was originally designed for `ctree()` and somewhat too narrowly focused on it. (3) Writing new “mobster” interfaces was not easy because of using unexported S4 classes.

Hence, a leaner and more flexible interface (based on S3 classes) is now provided in **partykit** (Hothorn and Zeileis 2015): (1) New models are much easier to provide in a basic version and customization does not require setting up an additional S4 class-and-methods layer anymore. (2) The trees are built on top of **partykit**’s flexible ‘**party**’ objects, inheriting many useful

methods and providing new ones dealing with the fitted models associated with the tree's nodes. (3) New “mobsters” dedicated to specific models, e.g., `lmtree()` and `glmmtree()` for MOB of (generalized) linear models, are readily provided.

The remainder of this vignette is organized as follows: Section 2 very briefly reviews the original MOB algorithm of Zeileis *et al.* (2008) and also highlights relevant subsequent work. Section 3 introduces the new `mob()` function in **partykit** in detail, discussing how all steps of the MOB algorithm are implemented and which options for customization are available. For illustration logistic-regression-based recursive partitioning is applied to the Pima Indians diabetes data set from the UCI machine learning repository (Bache and Lichman 2013). Section 4 and 5 present further illustrative examples (including replications from Zeileis *et al.* 2008) before Section 6 provides some concluding remarks.

## 2. MOB: Model-based recursive partitioning

First, the theory underling the MOB (model-based recursive partitioning) is briefly reviewed; a more detailed discussion is provided by Zeileis *et al.* (2008). To fix notation, consider a parametric model  $\mathcal{M}(Y, \theta)$  with (possibly vector-valued) observations  $Y$  and a  $k$ -dimensional vector of parameters  $\theta$ . This model could be a (possibly multivariate) normal distribution for  $Y$ , a psychometric model for a matrix of responses  $Y$ , or some kind of regression model when  $Y = (y, x)$  can be split up into a dependent variable  $y$  and regressors  $x$ . An example for the latter could be a linear regression model  $y = x^\top \theta$  or a generalized linear model (GLM) or a survival regression.

Given  $n$  observations  $Y_i$  ( $i = 1, \dots, n$ ) the model can be fitted by minimizing some objective function  $\sum_{i=1}^n \Psi(Y_i, \theta)$ , e.g., a residual sum of squares or a negative log-likelihood leading to ordinary least squares (OLS) or maximum likelihood (ML) estimation, respectively.

If a global model for all  $n$  observations does not fit well and further covariates  $Z_1, \dots, Z_\ell$  are available, it might be possible to partition the  $n$  observations with respect to these variables and find a fitting local model in each cell of the partition. The MOB algorithm tries to find such a partition adaptively using a greedy forward search. The reasons for looking at such local models might be different for different types of models: First, the detection of interactions and nonlinearities in regression relationships might be of interest just like in standard classification and regression trees (see e.g., Zeileis *et al.* 2008). Additionally, however, this approach allows to add explanatory variables to models that otherwise do not have regressors or where the link between the regressors and the parameters of the model is unclear (this idea is pursued by Strobl, Wickelmaier, and Zeileis 2011). Finally, the model-based tree can be employed as a thorough diagnostic test of the parameter stability assumption (also termed measurement invariance in psychometrics). If the tree does not split at all, parameter stability (or measurement invariance) cannot be rejected while a tree with splits would indicate in which way the assumption is violated (Strobl, Kopf, and Zeileis 2015, employ this idea in psychometric item response theory models).

The basic idea is to grow a tree in which every node is associated with a model of type  $\mathcal{M}$ . To assess whether splitting of the node is necessary a fluctuation test for parameter instability is performed. If there is significant instability with respect to any of the partitioning variables  $Z_j$ , the node is splitted into  $B$  locally optimal segments (the current version of the software has  $B = 2$  as the default and as the only option for numeric/ordered variables) and then the

procedure is repeated in each of the  $B$  children. If no more significant instabilities can be found, the recursion stops. More precisely, the steps of the algorithm are

1. Fit the model once to all observations in the current node.
2. Assess whether the parameter estimates are stable with respect to every partitioning variable  $Z_1, \dots, Z_\ell$ . If there is some overall instability, select the variable  $Z_j$  associated with the highest parameter instability, otherwise stop.
3. Compute the split point(s) that locally optimize the objective function  $\Psi$ .
4. Split the node into child nodes and repeat the procedure until some stopping criterion is met.

This conceptual framework is extremely flexible and allows to adapt it to various tasks by choosing particular models, tests, and methods in each of the steps:

1. *Model estimation:* The original MOB introduction (Zeileis *et al.* 2008) discussed regression models: OLS regression, GLMs, and survival regression. Subsequently, Grün, Kosmidis, and Zeileis (2012) have also adapted MOB to beta regression for limited response variables. Furthermore, MOB provides a generic way of adding covariates to models that otherwise have no regressors: this can either serve as a check whether the model is indeed independent from regressors or leads to local models for subsets. Both views are of interest when employing MOB to detect parameter instabilities in psychometric models for item responses such as the Bradley-Terry or the Rasch model (see Strobl *et al.* 2011, 2015, respectively).
2. *Parameter instability tests:* To assess the stability of all model parameters across a certain partitioning variable, the general class of score-based fluctuation tests proposed by Zeileis and Hornik (2007) is employed. Based on the empirical score function observations (i.e., empirical estimating functions or contributions to the gradient), ordered with respect to the partitioning variable, the fluctuation or instability in the model's parameters can be tested. From this general framework the Andrews' sup $LM$  test is used for assessing numerical partitioning variables and a  $\chi^2$  test for categorical partitioning variables (see Zeileis 2005 and Merkle and Zeileis 2013 for unifying views emphasizing regression and psychometric models, respectively). Furthermore, the test statistics for ordinal partitioning variables suggested by Merkle, Fan, and Zeileis (2014) have been added as further options (but are not used by default as the simulation of  $p$ -values is computationally demanding).
3. *Partitioning:* As the objective function  $\Psi$  is additive, it is easy to compute a single optimal split point (or cut point or break point). For each conceivable split, the model is estimated on the two resulting subsets and the resulting objective functions are summed. The split that optimizes this segmented objective function is then selected as the optimal split. For optimally splitting the data into  $B > 2$  segments, the same idea can be used and a full grid search can be avoided by employing a dynamic programming algorithms (Hawkins 2001; Bai and Perron 2003) but at the moment the latter is not implemented in the software. Optionally, however, categorical partitioning variables can be split into all of their categories (i.e., in that case  $B$  is set to the number of levels without searching for optimal groupings).

4. *Pruning*: For determining the optimal size of the tree, one can either use a pre-pruning or post-pruning strategy. For the former, the algorithm stops when no significant parameter instabilities are detected in the current node (or when the node becomes too small). For the latter, one would first grow a large tree (subject only to a minimal node size requirement) and then prune back splits that did not improve the model, e.g., judging by information criteria such as AIC or BIC (see e.g., [Su, Wang, and Fan 2004](#)). Currently, pre-pruning is used by default (via Bonferroni-corrected  $p$ -values from the score-based fluctuation tests) but AIC/BIC-based post-pruning is optionally available (especially for large data sets where traditional significance levels are not useful).

In the following it is discussed how most of the options above are embedded in a common computational framework using R's facilities for model estimation and object orientation.

### 3. A new implementation in R

This section introduces a new implementation of the general model-based recursive partitioning (MOB) algorithm in R. Along with [Zeileis \*et al.\* \(2008\)](#), a function `mob()` had been introduced to the **party** package ([Hothorn \*et al.\* 2015](#)) which continues to work but it turned out to be somewhat unflexible for certain applications/extensions. Hence, the **partykit** package ([Hothorn and Zeileis 2015](#)) provides a completely rewritten (and not backward compatible) implementation of a new `mob()` function along with convenience interfaces `lmtree()` and `glmmtree()` for fitting linear model and generalized linear model trees, respectively. The function `mob()` itself is intended to be the workhorse function that can also be employed to quickly explore new models – whereas `lmtree()` and `glmmtree()` will be the typical user interfaces facilitating applications.

The new `mob()` function has the following arguments:

```
mob(formula, data, subset, na.action, weights, offset,
    fit, control = mob_control(), ...)
```

All arguments in the first line are standard for modeling functions in R with a `formula` interface. They are employed by `mob()` to do some data preprocessing (described in detail in Section 3.1) before the `fit` function is used for parameter estimation on the preprocessed data. The `fit` function has to be set up in a certain way (described in detail in Section 3.2) so that `mob()` can extract all information that is needed in the MOB algorithm for parameter instability tests (see Section 3.3) and partitioning/splitting (see Section 3.4), i.e., the estimated parameters, the associated objective function, and the score function contributions. A list of `control` options can be set up by the `mob_control()` function, including options for pruning (see Section 3.5). Additional arguments `...` are passed on to the `fit` function.

The result is an object of class ‘`modelparty`’ inheriting from ‘`party`’. The `info` element of the overall ‘`party`’ and the individual ‘`node`’s contain various informations about the models. Details are provided in Section 3.6.

Finally, a wide range of standard (and some extra) methods are available for working with ‘`modelparty`’ objects, e.g., for extracting information about the models, for visualization, computing predictions, etc. The standard set of methods is introduced in Section 3.7. However, as will be discussed there, it may take some effort by the user to efficiently compute

certain pieces of information. Hence, convenience interfaces such as `lmtree()` or `glmtree()` can alleviate these obstacles considerably, as illustrated in Section 3.8.

### 3.1. Formula processing and data preparation

The formula processing within `mob()` is essentially done in “the usual way”, i.e., there is a `formula` and `data` and optionally further arguments such as `subset`, `na.action`, `weights`, and `offset`. These are processed into a `model.frame` from which the response and the covariates can be extracted and passed on to the actual `fit` function.

As there are possibly three groups of variables (response, regressors, and partitioning variables), the **Formula** package (Zeileis and Croissant 2010) is employed for processing these three parts. Thus, the formula can be of type  $y \sim x_1 + \dots + x_k \mid z_1 + \dots + z_l$  where the variables on the left of the `|` specify the data  $Y$  and the variables on the right specify the partitioning variables  $Z_j$ . As pointed out above, the  $Y$  can often be split up into response ( $y$  in the example above) and regressors ( $x_1, \dots, x_k$  in the example above). If there are no regressors and just constant fits are employed, then the formula can be specified as  $y \sim 1 \mid z_1 + \dots + z_l$ .

So far, this formula representation is really just a specification of groups of variables and does not imply anything about the type of model that is to be fitted to the data in the nodes of the tree. The `mob()` function does not know anything about the type of model and just passes (subsets of) the  $y$  and  $x$  variables on to the `fit` function. Only the partitioning variables  $z$  are used internally for the parameter instability tests (see Section 3.3).

As different `fit` functions will require the data in different formats, `mob_control()` allows to set the `ytype` and `xtype`. The default is to assume that  $y$  is just a single column of the model frame that is extracted as a `ytype = "vector"`. Alternatively, it can be a `"data.frame"` of all response variables or a `"matrix"` set up via `model.matrix()`. The options `"data.frame"` and `"matrix"` are also available for `xtype` with the latter being the default. Note that if `"matrix"` is used, then transformations (e.g., logs, square roots etc.) and dummy/interaction codings are computed and turned into columns of a numeric matrix while for `"data.frame"` the original variables are preserved.

By specifying the `ytype` and `xtype`, `mob()` is also provided with the information on how to correctly subset  $y$  and  $x$  when recursively partitioning data. In each step, only the subset of  $y$  and  $x$  pertaining to the current node of the tree is passed on to the `fit` function. Similarly, subsets of `weights` and `offset` are passed on (if specified).

#### *Illustration*

For illustration, we employ the popular benchmark data set on diabetes among Pima Indian women that is provided by the UCI machine learning repository (Bache and Lichman 2013) and available in the `mlbench` package (Leisch and Dimitriadou 2012):

```
R> data("PimaIndiansDiabetes", package = "mlbench")
```

Following Zeileis *et al.* (2008) we want to fit a model for `diabetes` employing the plasma glucose concentration `glucose` as a regressor. As the influence of the remaining variables on `diabetes` is less clear, their relationship should be learned by recursive partitioning. Thus, we employ the following formula:

```
R> pid_formula <- diabetes ~ glucose | pregnant + pressure + triceps +
+   insulin + mass + pedigree + age
```

Before passing this to `mob()`, a `fit` function is needed and a logistic regression function is set up in the following section.

### 3.2. Model fitting and parameter estimation

The `mob()` function itself does not actually carry out any parameter estimation by itself, but assumes that one of the many R functions available for model estimation is supplied. However, to be able to carry out the steps of the MOB algorithm, `mob()` needs to be able to extract certain pieces of information: especially the estimated parameters, the corresponding objective function, and associated score function contributions. Also, the interface of the fitting function clearly needs to be standardized so that `mob()` knows how to invoke the model estimation.

Currently, two possible interfaces for the `fit` function can be employed:

1. The `fit` function can take the following inputs

```
fit(y, x = NULL, start = NULL, weights = NULL, offset = NULL, ...,
    estfun = FALSE, object = FALSE)
```

where `y`, `x`, `weights`, `offset` are (the subset of) the preprocessed data. In `start` starting values for the parameter estimates may be supplied and `...` is passed on from the `mob()` function. The `fit` function then has to return an output list with the following elements:

- **coefficients:** Estimated parameters  $\hat{\theta}$ .
- **objfun:** Value of the minimized objective function  $\sum_i \Psi(y_i, x_i, \hat{\theta})$ .
- **estfun:** Empirical estimating functions (or score function contributions)  $\Psi'(y_i, x_i, \hat{\theta})$ . Only needed if `estfun = TRUE`, otherwise optionally `NULL`.
- **object:** A model object for which further methods could be available (e.g., `predict()`, or `fitted()`, etc.). Only needed if `object = TRUE`, otherwise optionally `NULL`.

By making `estfun` and `object` optional, the fitting function might be able to save computation time by only optimizing the objective function but avoiding further computations (such as setting up covariance matrix, residuals, diagnostics, etc.).

2. The `fit` function can also of a simpler interface with only the following inputs:

```
fit(y, x = NULL, start = NULL, weights = NULL, offset = NULL, ...)
```

The meaning of all arguments is the same as above. However, in this case `fit` needs to return a classed model object for which methods to `coef()`, `logLik()`, and `estfun()` (see Zeileis 2006, and the `sandwich` package) are available for extracting the parameter estimates, the maximized log-likelihood, and associated empirical estimating functions (or score contributions), respectively. Internally, a function of type (1) is set up by `mob()` in case a function of type (2) is supplied. However, as pointed out above, a function of type (1) might be useful to save computation time.

In either case the `fit` function can, of course, choose to ignore any arguments that are not applicable, e.g., if there are no regressors `x` in the model or if starting values are not supported. The `fit` function of type (2) is typically convenient to quickly try out a new type of model in recursive partitioning. However, when writing a new `mob()` interface such as `lmtree()` or `glmtree()`, it will typically be better to use type (1). Similarly, employing supporting starting values in `fit` is then recommended to save computation time.

### *Illustration*

For recursively partitioning the `diabetes ~ glucose` relationship (as already set up in the previous section), we employ a logistic regression model. An interface of type (2) can be easily set up:

```
R> logit <- function(y, x, start = NULL, weights = NULL, offset = NULL, ...) {
+   glm(y ~ 0 + x, family = binomial, start = start, ...)
+ }
```

Thus, `y`, `x`, and the starting values are passed on to `glm()` which returns an object of class ‘`glm`’ for which all required methods (`coef()`, `logLik()`, and `estfun()`) are available.

Using this `fit` function and the formula already set up above the MOB algorithm can be easily applied to the `PimaIndiansDiabetes` data:

```
R> pid_tree <- mob(pid_formula, data = PimaIndiansDiabetes, fit = logit)
```

The result is a logistic regression tree with three terminal nodes that can be easily visualized via `plot(pid_tree)` (see Figure 1) and printed:

```
R> pid_tree
```

Model-based recursive partitioning (logit)

Model formula:

```
diabetes ~ glucose | pregnant + pressure + triceps + insulin +
  mass + pedigree + age
```

Fitted party:

```
[1] root
| [2] mass <= 26.3: n = 167
|   x(Intercept)    xglucose
|   -9.95151        0.05871
| [3] mass > 26.3
| | [4] age <= 30: n = 304
| |   x(Intercept)    xglucose
| |   -6.70559        0.04684
| | [5] age > 30: n = 297
| |   x(Intercept)    xglucose
| |   -2.77095        0.02354
```

```

Number of inner nodes:    2
Number of terminal nodes: 3
Number of parameters per node: 2
Objective function: 355.5

```

The tree finds three groups of Pima Indian women:

- #2 Women with low body mass index that have on average a low risk of diabetes, however this increases clearly with glucose level.
- #4 Women with average and high body mass index, younger than 30 years, that have a higher average risk that also increases with glucose level.
- #5 Women with average and high body mass index, older than 30 years, that have a high average risk that increases only slowly with glucose level.

Note that the example above is used for illustration here and `glmtree()` is recommended over using `mob()` plus manually setting up a `logit()` function. The same tree structure can be found via:

```

R> pid_tree2 <- glmtree(diabetes ~ glucose | pregnant +
+   pressure + triceps + insulin + mass + pedigree + age,
+   data = PimaIndiansDiabetes, family = binomial)

```

However, `glmtree()` is slightly faster as it avoids many unnecessary computations, see Section 3.8 for further details.

Here, we only point out that `plot(pid_tree2)` produces a nicer visualization (see Figure 2). As  $y$  is `diabetes`, a binary variable, and  $x$  is `glucose`, a numeric variable, a spinogram is chosen automatically for visualization (using the `vcd` package, Meyer, Zeileis, and Hornik 2006). The x-axis breaks in the spinogram are the five-point summary of `glucose` on the full data set. The fitted lines are the mean predicted probabilities in each group.

### 3.3. Testing for parameter instability

In each node of the tree, first the parametric model is fitted to all observations in that node (see Section 3.2). Subsequently it is of interest to find out whether the model parameters are stable over each particular ordering implied by the partitioning variables  $Z_j$  or whether splitting the sample with respect to one of the  $Z_j$  might capture instabilities in the parameters and thus improve the fit. The tests used in this step belong to the class of generalized M-fluctuation tests (Zeileis 2005; Zeileis and Hornik 2007). Depending on the class of each of the partitioning variables in  $\mathbf{z}$  different types of tests are chosen by `mob()`:

1. For numeric partitioning variables (of class ‘`numeric`’ or ‘`integer`’) the  $\text{sup}LM$  statistic is used which is the maximum over all single-split  $LM$  statistics. Associated  $p$ -values can be obtained from a table of critical values (based on Hansen 1997) stored within the package.

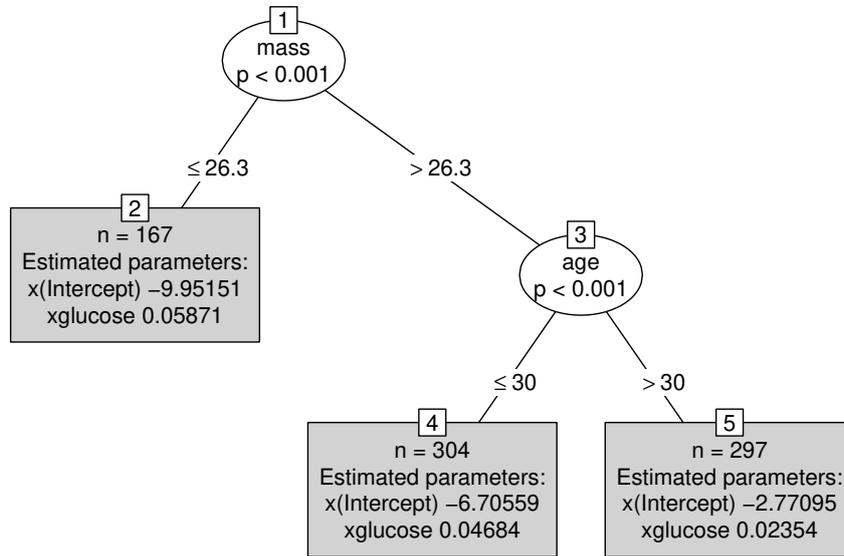

Figure 1: Logistic-regression-based tree for the Pima Indians diabetes data. The plots in the leaves report the estimated regression coefficients.

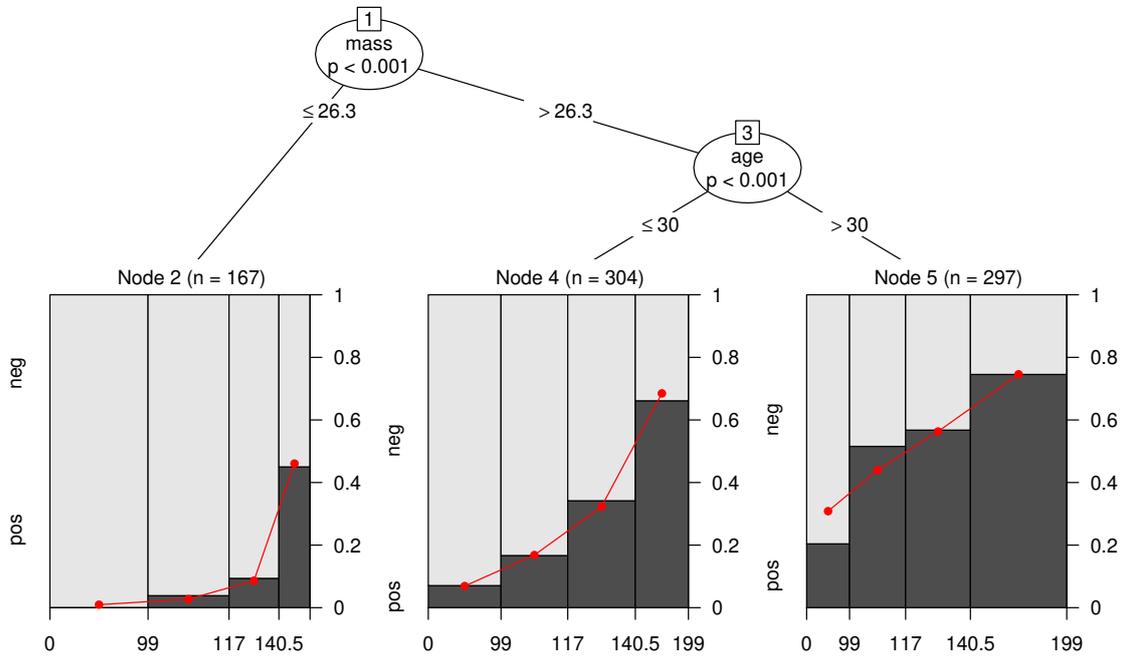

Figure 2: Logistic-regression-based tree for the Pima Indians diabetes data. The plots in the leaves give spinograms for diabetes versus glucose.

If there are ties in the partitioning variable, the sequence of  $LM$  statistics (and hence their maximum) is not unique and hence the results by default may depend to some degree on the ordering of the observations. To explore this, the option `breakties = TRUE` can be set in `mob_control()` which breaks ties randomly. If there are only few ties, the influence is often negligible. If there are many ties (say only a dozen unique values of the partitioning variable), then the variable may be better treated as an ordered factor (see below).

2. For categorical partitioning variables (of class ‘`factor`’), a  $\chi^2$  statistic is employed which captures the fluctuation within each of the categories of the partitioning variable. This is also an  $LM$ -type test and is asymptotically equivalent to the corresponding likelihood ratio test. However, it is somewhat cheaper to compute the  $LM$  statistic because the model just has to be fitted once in the current node and not separately for each category of each possible partitioning variable. See also [Merkle \*et al.\* \(2014\)](#) for a more detailed discussion.
3. For ordinal partitioning variables (of class ‘`ordered`’ inheriting from ‘`factor`’) the same  $\chi^2$  as for the unordered categorical variables is used by default (as suggested by [Zeileis \*et al.\* 2008](#)). Although this test is consistent for any parameter instabilities across ordered variables, it does not exploit the ordering information.

Recently, [Merkle \*et al.\* \(2014\)](#) proposed an adapted  $\max LM$  test for ordered variables and, alternatively, a weighted double maximum test. Both are optionally available in the new `mob()` implementation by setting `ordinal = "L2"` or `ordinal = "max"` in `mob_control()`, respectively. Unfortunately, computing  $p$ -values from both tests is more costly than for the default `ordinal = "chisq"`. For "L2" suitable tables of critical values have to be simulated on the fly using `ordL2BB()` from the `strucchange` package ([Zeileis, Leisch, Hornik, and Kleiber 2002](#)). For "max" a multivariate normal probability has to be computed using the `mvtnorm` package ([Genz \*et al.\* 2015](#)).

All of the parameter instability tests above can be computed in an object-oriented manner as the “`estfun`” has to be available for the fitted model object. (Either by computing it in the `fit` function directly or by providing a `estfun()` extractor, see Section 3.2.)

All tests also require an estimate of the corresponding variance-covariance matrix of the estimating functions. The default is to compute this using an outer-product-of-gradients (OPG) estimator. Alternatively, the corresponding information matrix or sandwich matrix can be used if: (a) the estimating functions are actually maximum likelihood scores, and (b) a `vcov()` method (based on an estimate of the information) is provided for the fitted model objects. The corresponding option in `mob_control()` is to set `vcov = "info"` or `vcov = "sandwich"` rather than `vcov = "opg"` (the default).

For each of the  $j = 1, \dots, \ell$  partitioning variables in  $\mathbf{z}$  the test selected in the control options is employed and the corresponding  $p$ -value  $p_j$  is computed. To adjust for multiple testing, the  $p$  values can be Bonferroni adjusted (which is the default). To determine whether there is some overall instability, it is checked whether the minimal  $p$ -value  $p_{j^*} = \min_{j=1, \dots, \ell} p_j$  falls below a pre-specified significance level  $\alpha$  (by default  $\alpha = 0.05$ ) or not. If there is significant instability, the variable  $Z_{j^*}$  associated with the minimal  $p$ -value is used for splitting the node.

*Illustration*

In the logistic-regression-based MOB `pid_tree` computed above, the parameter instability tests can be extracted using the `sctest()` function from the **strucchange** package (for structural change test). In the first node, the test statistics and Bonferroni-corrected  $p$ -values are:

```
R> library("strucchange")
R> sctest(pid_tree, node = 1)

      pregnant pressure  triceps insulin      mass pedigree
statistic 2.989e+01   7.5024 15.94095  6.5969 4.881e+01 18.33476
p.value   9.778e-05   0.9104  0.06474  0.9701 8.317e-09  0.02253
      age
statistic 4.351e+01
p.value   1.183e-07
```

Thus, the body mass index has the lowest  $p$ -value and is highly significant and hence used for splitting the data. In the second node, no further significant parameter instabilities can be detected and hence partitioning stops in that branch.

```
R> sctest(pid_tree, node = 2)

      pregnant pressure  triceps insulin      mass pedigree      age
statistic 10.3923   4.3538  5.9114   3.786 10.4749   3.626 6.0978
p.value    0.4903   0.9998  0.9869   1.000 0.4785   1.000 0.9818
```

In the third node, however, there is still significant instability associated with the `age` variable and hence partitioning continues.

```
R> sctest(pid_tree, node = 3)

      pregnant pressure  triceps insulin      mass pedigree
statistic 2.674e+01   6.1758  7.3468   7.896 9.1546 17.96439
p.value   4.434e-04   0.9845  0.9226   0.870 0.7033  0.02647
      age
statistic 3.498e+01
p.value   8.099e-06
```

Because no further instabilities can be found in the fourth and fifth node, the recursive partitioning stops there.

**3.4. Splitting**

In this step, the observations in the current node are split with respect to the chosen partitioning variable  $Z_{j^*}$  into  $B$  child nodes. As pointed out above, the `mob()` function currently only supports binary splits, i.e.,  $B = 2$ . For determining the split point, an exhaustive search

procedure is adopted: For each conceivable split point in  $Z_{j^*}$ , the two subset models are fit and the split associated with the minimal value of the objective function  $\Psi$  is chosen.

Computationally, this means that the `fit` function is applied to the subsets of  $y$  and  $x$  for each possibly binary split. The “`objfun`” values are simply summed up (because the objective function is assumed to be additive) and its minimum across splits is determined. In a search over a numeric partitioning variable, this means that typically a lot of subset models have to be fitted and often these will not vary a lot from one split to the next. Hence, the parameter estimates “`coefficients`” from the previous split are employed as `start` values for estimating the coefficients associated with the next split. Thus, if the `fit` function makes use of these starting values, the model fitting can often be speeded up.

### *Illustration*

For the Pima Indians diabetes data, the split points found for `pid_tree` are displayed both in the print output and the visualization (see Figure 1 and 2).

## 3.5. Pruning

By default, the size of `mob()` trees is determined only by the significance tests, i.e., when there is no more significant parameter instability (by default at level  $\alpha = 0.05$ ) the tree stops growing. Additional stopping criteria are only the minimal node size (`minsize`) and the maximum tree depth (`maxdepth`, by default infinity).

However, for very large sample size traditional significance levels are typically not useful because even tiny parameter instabilities can be detected. To avoid overfitting in such a situation, one would either have to use much smaller significance levels or add some form of post-pruning to reduce the size of the tree afterwards. Similarly, one could wish to first grow a very large tree (using a large  $\alpha$  level) and then prune it afterwards, e.g., using some information criterion like AIC or BIC.

To accommodate such post-pruning strategies, `mob_control()` has an argument `prune` that can be a `function(objfun, df, nobs)` that either returns `TRUE` if a node should be pruned or `FALSE` if not. The arguments supplied are a vector of objective function values in the current node and the sum of all child nodes, a vector of corresponding degrees of freedom, and the number of observations in the current node and in total. For example if the objective function used is the negative log-likelihood, then for BIC-based pruning the `prune` function is:  $(2 * \text{objfun}[1] + \log(\text{nobs}[1]) * \text{df}[1]) < (2 * \text{objfun}[2] + \log(\text{nobs}[2]) * \text{df}[2])$ . As the negative log-likelihood is the default objective function when using the “simple” `fit` interface, `prune` can also be set to “AIC” or “BIC” and then suitable functions will be set up internally. Note, however, that for other objective functions this strategy is not appropriate and the functions would have to be defined differently (which `lmtree()` does for example).

In the literature, there is no clear consensus as to how many degrees of freedom should be assigned to the selection of a split point. Hence, `mob_control()` allows to set `dfsplitted` which by default is `dfsplitted = TRUE` and then `as.integer(dfsplitted)` (i.e., 1 by default) degrees of freedom per split are used. This can be modified to `dfsplitted = FALSE` (or equivalently `dfsplitted = 0`) or `dfsplitted = 3` etc. for lower or higher penalization of additional splits.

*Illustration*

With  $n = 768$  observations, the sample size is quite reasonable for using the classical significance level of  $\alpha = 0.05$  which is also reflected by the moderate tree size with three terminal nodes. However, if we wished to explore further splits, a conceivable strategy could be the following:

```
R> pid_tree3 <- mob(pid_formula, data = PimaIndiansDiabetes,
+   fit = logit, control = mob_control(verbose = TRUE,
+   minsize = 50, maxdepth = 4, alpha = 0.9, prune = "BIC"))
```

This first grows a large tree until the nodes become too small (minimum node size: 50 observations) or the tree becomes too deep (maximum depth 4 levels) or the significance levels come very close to one (larger than  $\alpha = 0.9$ ). Here, this large tree has eleven nodes which are subsequently pruned based on whether or not they improve the BIC of the model. For this data set, the resulting BIC-pruned tree is in fact identical to the pre-pruned `pid_tree` considered above.

**3.6. Fitted ‘party’ objects**

The result of `mob()` is an object of class ‘`modelparty`’ inheriting from ‘`party`’. See the other vignettes in the `partykit` package (Hothorn and Zeileis 2015) for more details of the general ‘`party`’ class. Here, we just point out that the main difference between a ‘`modelparty`’ and a plain ‘`party`’ is that additional information about the data and the associated models is stored in the `info` elements: both of the overall ‘`party`’ and the individual ‘`node`’s. The details are exemplified below.

*Illustration*

In the `info` of the overall ‘`party`’ the following information is stored for `pid_tree`:

```
R> names(pid_tree$info)

[1] "call"      "formula" "Formula" "terms"    "fit"      "control"
[7] "dots"      "nreg"
```

The `call` contains the `mob()` call. The `formula` and `Formula` are virtually the same but are simply stored as plain ‘`formula`’ and extended ‘`Formula`’ (Zeileis and Croissant 2010) objects, respectively. The `terms` contain separate lists of terms for the `response` (and regressor) and the `partitioning` variables. The `fit`, `control` and `dots` are the arguments that were provided to `mob()` and `nreg` is the number of regressor variables.

Furthermore, each `node` of the tree contains the following information:

```
R> names(pid_tree$node$info)

[1] "criterion"    "p.value"      "coefficients" "objfun"
[5] "object"      "converged"    "nobs"
```

The `coefficients`, `objfun`, and `object` are the results of the `fit` function for that node. In `nobs` and `p.value` the number of observations and the minimal  $p$ -value are provided, respectively. Finally, `test` contains the parameter instability test results. Note that the `object` element can also be suppressed through `mob_control()` to save memory space.

### 3.7. Methods

There is a wide range of standard methods available for objects of class ‘`modelparty`’. The standard `print()`, `plot()`, and `predict()` build on the corresponding methods for ‘`party`’ objects but provide some more special options. Furthermore, methods are provided that are typically available for models with formula interfaces: `formula()` (optionally one can set `extended = TRUE` to get the ‘Formula’), `getCall()`, `model.frame()`, `weights()`. Finally, there is a standard set of methods for statistical model objects: `coef()`, `residuals()`, `logLik()` (optionally setting `dfsplitted = FALSE` suppresses counting the splits in the degrees of freedom, see Section 3.5), `deviance()`, `fitted()`, and `summary()`.

Some of these methods rely on reusing the corresponding methods for the individual model objects in the terminal nodes. Functions such as `coef()`, `print()`, `summary()` also take a `node` argument that can specify the node IDs to be queried.

Two methods have non-standard arguments to allow for additional flexibility when dealing with model trees. Typically, “normal” users do not have to use these arguments directly but they are very flexible and facilitate writing convenience interfaces such as `glmtree()` (see Section 3.8).

- The `predict()` method has the following arguments: `predict(object, newdata = NULL, type = "node", ...)`. The argument `type` can either be a function or a character string. More precisely, if `type` is a function it should be a function `(object, newdata = NULL, ...)` that returns a vector or matrix of predictions from a fitted model `object` either with or without `newdata`. If `type` is a character string, such a function is set up internally as `predict(object, newdata = newdata, type = type, ...)`, i.e., it relies on a suitable `predict()` method being available for the fitted models associated with the ‘`party`’ object.
- The `plot()` method has the following arguments: `plot(x, terminal_panel = NULL, FUN = NULL)`. This simply calls the `plot()` method for ‘`party`’ objects with a custom panel function for the terminal panels. By default, `node_terminal` is used to include some short text in each terminal node. This text can be set up by `FUN` with the default being the number of observations and estimated parameters. However, more elaborate terminal panel functions can be written, as done for the convenience interfaces.

Finally, two S3-style functions are provided without the corresponding generics (as these reside in packages that `partykit` does not depend on). The `sctest.modelparty` can be used in combination with the `sctest()` generic from `strucchange` as illustrated in Section 3.3. The `refit.modelparty` function extracts (or refits if necessary) the fitted model objects in the specified nodes (by default from all nodes).

#### *Illustration*

The `plot()` and `print()` methods have already been illustrated for the `pid_tree` above.

However, here we add that the `print()` method can also be used to show more detailed information about particular nodes instead of showing the full tree:

```
R> print(pid_tree, node = 3)
```

```
Model-based recursive partitioning (logit)
```

```
-- Node 3 --
```

```
Estimated parameters:
```

```
x(Intercept)    xglucose
      -4.61015      0.03426
```

```
Objective function:
```

```
344.2
```

```
Parameter instability tests:
```

```
          pregnant pressure triceps insulin  mass pedigree
statistic 2.674e+01  6.1758  7.3468   7.896 9.1546 17.96439
p.value   4.434e-04  0.9845  0.9226   0.870 0.7033 0.02647
          age
statistic 3.498e+01
p.value   8.099e-06
```

Information about the model and coefficients can for example be extracted by:

```
R> coef(pid_tree)
```

```
      x(Intercept) xglucose
2          -9.952  0.05871
4          -6.706  0.04684
5          -2.771  0.02354
```

```
R> coef(pid_tree, node = 1)
```

```
x(Intercept)    xglucose
      -5.35008      0.03787
```

```
R> summary(pid_tree, node = 1)
```

```
Call:
```

```
glm(formula = y ~ 0 + x, family = binomial, start = start)
```

```
Deviance Residuals:
```

```
      Min       1Q   Median       3Q      Max
-2.110  -0.784  -0.536   0.857   3.273
```

```
Coefficients:
```

```

                Estimate Std. Error z value Pr(>|z|)
x(Intercept) -5.35008    0.42083  -12.7   <2e-16 ***
xglucose      0.03787    0.00325   11.7   <2e-16 ***
---
Signif. codes:  0 '***' 0.001 '**' 0.01 '*' 0.05 '.' 0.1 ' ' 1

```

(Dispersion parameter for binomial family taken to be 1)

```

Null deviance: 1064.67 on 768 degrees of freedom
Residual deviance: 808.72 on 766 degrees of freedom
AIC: 812.7

```

Number of Fisher Scoring iterations: 4

As the coefficients pertain to a logistic regression, they can be easily interpreted as odds ratios by taking the `exp()`:

```
R> exp(coef(pid_tree)[,2])
```

```

      2      4      5
1.060 1.048 1.024

```

i.e., the odds increase by 6%, 4.8% and 2.4% with respect to glucose in the three terminal nodes.

Log-likelihoods and information criteria are available (which by default also penalize the estimation of splits):

```
R> logLik(pid_tree)
```

```
'log Lik.' -355.5 (df=8)
```

```
R> AIC(pid_tree)
```

```
[1] 726.9
```

```
R> BIC(pid_tree)
```

```
[1] 764.1
```

Mean squared residuals (or deviances) can be extracted in different ways:

```
R> mean(residuals(pid_tree)^2)
```

```
[1] 0.9257
```

```
R> deviance(pid_tree)/sum(weights(pid_tree))
```

```
[1] 0.9257
```

```
R> deviance(pid_tree)/nobs(pid_tree)
```

```
[1] 0.9257
```

Predicted nodes can also be easily obtained:

```
R> pid <- head(PimaIndiansDiabetes)
```

```
R> predict(pid_tree, newdata = pid, type = "node")
```

```
1 2 3 4 5 6
5 5 2 4 5 2
```

More predictions, e.g., predicted probabilities within the nodes, can also be obtained but require some extra coding if only `mob()` is used. However, with the `glmtree()` interface this is very easy as shown below.

Finally, several methods for ‘party’ objects are, of course, also available for ‘modelparty’ objects, e.g., querying width and depth of the tree:

```
R> width(pid_tree)
```

```
[1] 3
```

```
R> depth(pid_tree)
```

```
[1] 2
```

Also subtrees can be easily extracted:

```
R> pid_tree[3]
```

Model-based recursive partitioning (logit)

Model formula:

```
diabetes ~ glucose | pregnant + pressure + triceps + insulin +
      mass + pedigree + age
```

Fitted party:

```
[3] root
|   [4] age <= 30: n = 304
|       x(Intercept)      xglucose
|       -6.70559         0.04684
|   [5] age > 30: n = 297
|       x(Intercept)      xglucose
|       -2.77095         0.02354
```

```

Number of inner nodes:    1
Number of terminal nodes: 2
Number of parameters per node: 2
Objective function: 325.2

```

The subtree is again a completely valid ‘`modelparty`’ and hence it could also be visualized via `plot(pid_tree[3])` etc.

### 3.8. Extensions and convenience interfaces

As illustrated above, dealing with MOBs can be carried out in a very generic and object-oriented way. Almost all information required for dealing with recursively partitioned models can be encapsulated in the `fit()` function and `mob()` does not require more information on what type of model is actually used.

However, for certain tasks more detailed information about the type of model used or the type of data it can be fitted to can (and should) be exploited. Notable examples for this are visualizations of the data along with the fitted model or model-based predictions in the leaves of the tree. To conveniently accommodate such specialized functionality, the **partykit** provides two convenience interfaces `lmtree()` and `glmtree()` and encourages other packages to do the same (e.g., `raschtree()` and `bttree()` in **psychotree**). Furthermore, such a convenience interface can avoid duplicated formula processing in both `mob()` plus its `fit` function.

Specifically, `lmtree()` and `glmtree()` interface `lm.fit()`, `lm.wfit()`, and `glm.fit()`, respectively, and then provide some extra computations to return valid fitted ‘`lm`’ and ‘`glm`’ objects in the nodes of the tree. The resulting ‘`modelparty`’ object gains an additional class ‘`lmtree`’/‘`glmtree`’ to dispatch to its enhanced `plot()` and `predict()` methods.

#### *Illustration*

The `pid_tree2` object was already created above with `glmtree()` (instead of `mob()` as for `pid_tree`) to illustrate the enhanced plotting capabilities in Figure 2. Here, the enhanced `predict()` method is used to obtain predicted means (i.e., probabilities) and associated linear predictors (on the logit scale) in addition to the previously available predicted nodes IDs.

```
R> predict(pid_tree2, newdata = pid, type = "node")
```

```

1 2 3 4 5 6
5 5 2 4 5 2

```

```
R> predict(pid_tree2, newdata = pid, type = "response")
```

```

      1      2      3      4      5      6
0.67092 0.31639 0.68827 0.07330 0.61146 0.04143

```

```
R> predict(pid_tree2, newdata = pid, type = "link")
```

```

      1      2      3      4      5      6
0.7123 -0.7704  0.7920 -2.5371  0.4535 -3.1414

```

## 4. Illustrations

In the remainder of the vignette, further empirical illustrations of the MOB method are provided, including replications of the results from [Zeileis \*et al.\* \(2008\)](#):

1. An investigation of the price elasticity of the demand for economics journals across co-variables describing the type of journal (e.g., its price, its age, and whether it is published by a society, etc.)
2. Prediction of house prices in the well-known Boston Housing data set, also taken from the UCI machine learning repository.
3. Explore how teaching ratings and beauty scores of professors are associated and how this association changes across further explanatory variables such as age, gender, and native speaker status of the professors.
4. Assessment of differences in the preferential treatment of women/children (“women and children first”) across subgroups of passengers on board of the ill-fated maiden voyage of the RMS Titanic.
5. Modeling of breast cancer survival by capturing heterogeneity in certain (treatment) effects across patients.
6. Modeling of paired comparisons of topmodel candidates by capturing heterogeneity in their attractiveness scores across participants in a survey.

More details about several of the underlying data sets, previous studies exploring the data, and the results based on MOB can be found in [Zeileis \*et al.\* \(2008\)](#).

Here, we focus on using the **partykit** package to replicate the analysis and explore the resulting trees. The first three illustrations employ the `lmtree()` convenience function, the fourth is based on logistic regression using `glmtree()`, and the fifth uses `survreg()` from **survival** ([Therneau 2015](#)) in combination with `mob()` directly. The sixth and last illustration is deferred to a separate section and shows in detail how to set up new “mobster” functionality from scratch.

### 4.1. Demand for economic journals

The price elasticity of the demand for 180 economic journals is assessed by an OLS regression in log-log form: The dependent variable is the logarithm of the number of US library subscriptions and the regressor is the logarithm of price per citation. The data are provided by the **AER** package ([Kleiber and Zeileis 2008](#)) and can be loaded and transformed via:

```
R> data("Journals", package = "AER")
R> Journals <- transform(Journals,
+   age = 2000 - foundingyear,
+   chars = charpp * pages)
```

Subsequently, the stability of the price elasticity across the remaining variables can be assessed using MOB. Below, `lmtree()` is used with the following partitioning variables: raw price and

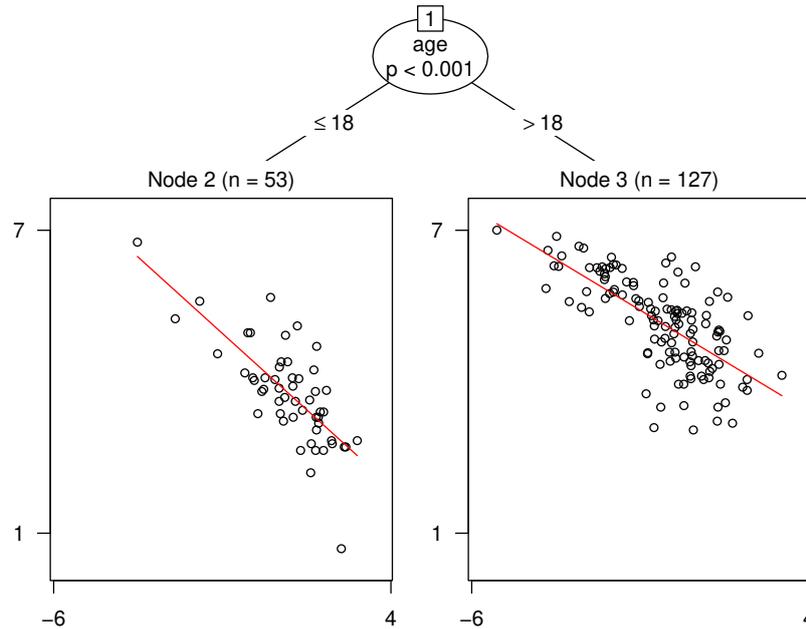

Figure 3: Linear-regression-based tree for the journals data. The plots in the leaves show linear regressions of  $\log(\text{subscriptions})$  by  $\log(\text{price}/\text{citation})$ .

citations, age of the journal, number of characters, and whether the journal is published by a scientific society or not. A minimal segment size of 10 observations is employed and by setting `verbose = TRUE` detailed progress information about the recursive partitioning is displayed while growing the tree:

```
R> j_tree <- lmtree(log(subs) ~ log(price/citations) | price + citations +
+   age + chars + society, data = Journals, minsize = 10, verbose = TRUE)
```

The resulting tree just has one split and two terminal nodes for young journals (with a somewhat larger price elasticity) and old journals (with an even lower price elasticity), respectively. Figure 3 can be obtained by `plot(j_tree)` and the corresponding printed representation is shown below.

```
R> j_tree
```

```
Linear model tree
```

```
Model formula:
```

```
log(subs) ~ log(price/citations) | price + citations + age +
  chars + society
```

```
Fitted party:
```

```
[1] root
| [2] age <= 18: n = 53
```

```
|           (Intercept) log(price/citations)
|           4.3528          -0.6049
| [3] age > 18: n = 127
|           (Intercept) log(price/citations)
|           5.011          -0.403
```

```
Number of inner nodes: 1
Number of terminal nodes: 2
Number of parameters per node: 2
Objective function (residual sum of squares): 77.05
```

Finally, various quantities of interest such as the coefficients, standard errors and test statistics, and the associated parameter instability tests could be extracted by the following code. The corresponding output is suppressed here.

```
R> coef(j_tree, node = 1:3)
R> summary(j_tree, node = 1:3)
R> sctest(j_tree, node = 1:3)
```

## 4.2. Boston housing data

The Boston housing data are a popular and well-investigated empirical basis for illustrating nonlinear regression methods both in machine learning and statistics. We follow previous analyses by segmenting a bivariate linear regression model for the house values.

The data set is available in package **mlbench** and can be obtained and transformed via:

```
R> data("BostonHousing", package = "mlbench")
R> BostonHousing <- transform(BostonHousing,
+   chas = factor(chas, levels = 0:1, labels = c("no", "yes")),
+   rad = factor(rad, ordered = TRUE))
```

It provides  $n = 506$  observations of the median value of owner-occupied homes in Boston (in USD 1000) along with 14 covariates including in particular the number of rooms per dwelling (**rm**) and the percentage of lower status of the population (**lstat**). A segment-wise linear relationship between the value and these two variables is very intuitive, whereas the shape of the influence of the remaining covariates is rather unclear and hence should be learned from the data. Therefore, a linear regression model for median value explained by  $\text{rm}^2$  and  $\log(\text{lstat})$  is employed and partitioned with respect to all remaining variables. Choosing appropriate transformations of the dependent variable and the regressors that enter the linear regression model is important to obtain a well-fitting model in each segment and we follow in our choice the recommendations of [Breiman and Friedman \(1985\)](#). Monotonic transformations of the partitioning variables do not affect the recursive partitioning algorithm and hence do not have to be performed. However, it is important to distinguish between numerical and categorical variables for choosing an appropriate parameter stability test. The variable **chas** is a dummy indicator variable (for tract bounds with Charles river) and thus needs to be turned into a factor. Furthermore, the variable **rad** is an index of accessibility to radial highways and takes only 9 distinct values. Hence, it is most appropriately treated as an ordered factor.

Note that both transformations only affect the parameter stability test chosen (step 2), not the splitting procedure (step 3).

```
R> bh_tree <- lmtree(medv ~ log(lstat) + I(rm^2) | zn + indus + chas + nox +
+   age + dis + rad + tax + crim + b + ptratio, data = BostonHousing)
R> bh_tree
```

Linear model tree

Model formula:

```
medv ~ log(lstat) + I(rm^2) | zn + indus + chas + nox + age +
  dis + rad + tax + crim + b + ptratio
```

Fitted party:

```
[1] root
| [2] tax <= 432
| | [3] ptratio <= 15.2: n = 72
| | | (Intercept) log(lstat) I(rm^2)
| | | 9.2349 -4.9391 0.6859
| | [4] ptratio > 15.2
| | | [5] ptratio <= 19.6
| | | | [6] tax <= 265: n = 63
| | | | | (Intercept) log(lstat) I(rm^2)
| | | | | 3.9637 -2.7663 0.6881
| | | | [7] tax > 265: n = 162
| | | | | (Intercept) log(lstat) I(rm^2)
| | | | | -1.7984 -0.2677 0.6539
| | | [8] ptratio > 19.6: n = 56
| | | | (Intercept) log(lstat) I(rm^2)
| | | | 17.5865 -4.6190 0.3387
| [9] tax > 432: n = 153
| | (Intercept) log(lstat) I(rm^2)
| | 68.2971 -16.3540 -0.1478
```

Number of inner nodes: 4

Number of terminal nodes: 5

Number of parameters per node: 3

Objective function (residual sum of squares): 6090

The corresponding visualization is shown in Figure 4. It shows partial scatter plots of the dependent variable against each of the regressors in the terminal nodes. Each scatter plot also shows the fitted values, i.e., a projection of the fitted hyperplane.

From this visualization, it can be seen that in the nodes 4, 6, 7 and 8 the increase of value with the number of rooms dominates the picture (upper panel) whereas in node 9 the decrease with the lower status population percentage (lower panel) is more pronounced. Splits are performed in the variables `tax` (property-tax rate) and `ptratio` (pupil-teacher ratio).

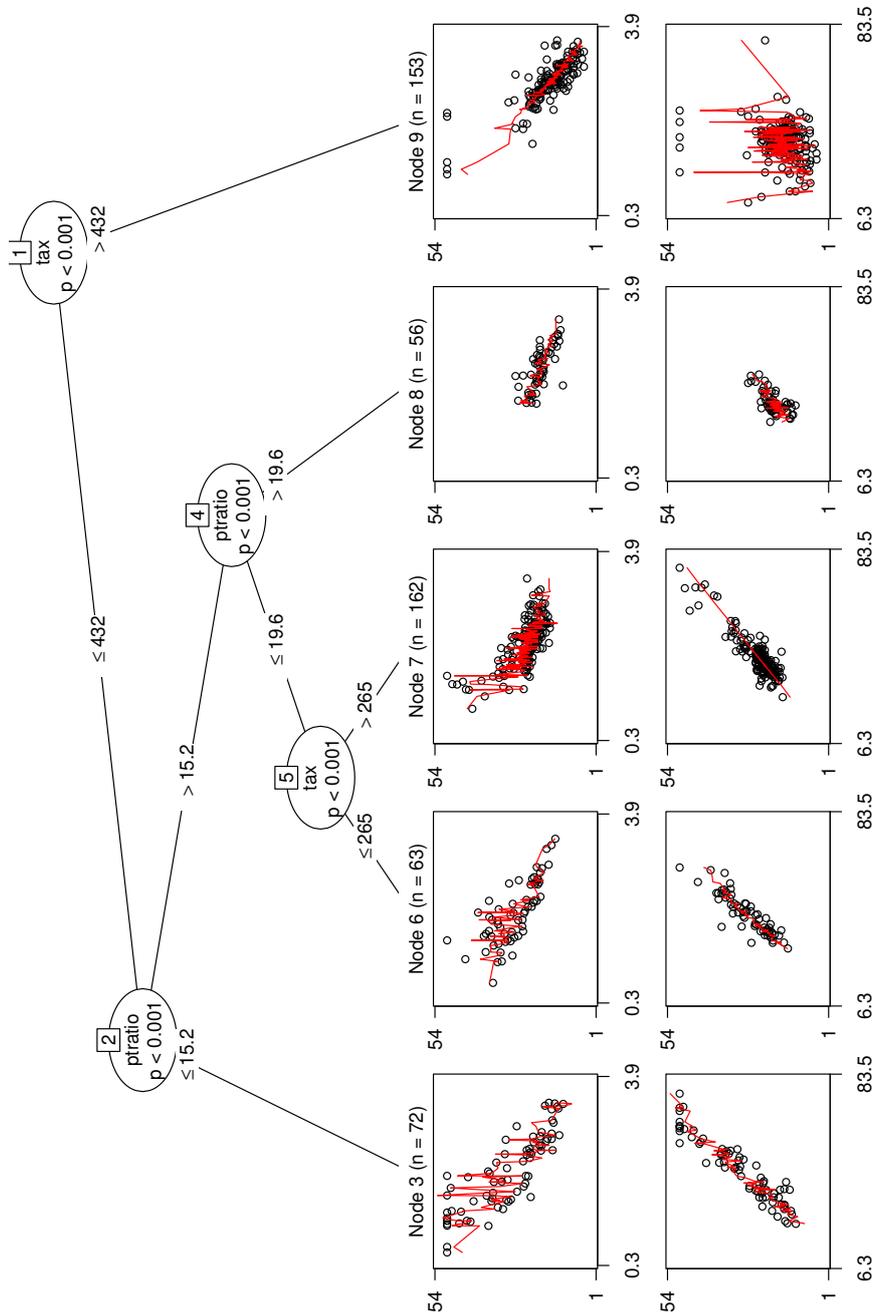

Figure 4: Linear-regression-based tree for the Boston housing data. The plots in the leaves give partial scatter plots for `rm` (upper panel) and `lstat` (lower panel).

For summarizing the quality of the fit, we could compute the mean squared error, log-likelihood or AIC:

```
R> mean(residuals(bh_tree)^2)
```

```
[1] 12.04
```

```
R> logLik(bh_tree)
```

```
'log Lik.' -1311 (df=24)
```

```
R> AIC(bh_tree)
```

```
[1] 2669
```

### 4.3. Teaching ratings data

[Hamermesh and Parker \(2005\)](#) investigate the correlation of beauty and teaching evaluations for professors. They provide data on course evaluations, course characteristics, and professor characteristics for 463 courses for the academic years 2000–2002 at the University of Texas at Austin. It is of interest how the average teaching evaluation per course (on a scale 1–5) depends on a standardized measure of beauty (as assessed by a committee of six persons based on photos). [Hamermesh and Parker \(2005\)](#) employ a linear regression, weighted by the number of students per course and adjusting for several further main effects: gender, whether or not the teacher is from a minority, a native speaker, or has tenure, respectively, and whether the course is taught in the upper or lower division. Additionally, the age of the professors is available as a regressor but not considered by [Hamermesh and Parker \(2005\)](#) because the corresponding main effect is not found to be significant in either linear or quadratic form.

Here, we employ a similar model but use the available regressors differently. The basic model is again a linear regression for teaching rating by beauty, estimated by weighted least squares (WLS). All remaining explanatory variables are *not* used as regressors but as partitioning variables because we argue that it is unclear how they influence the correlation between teaching rating and beauty. Hence, MOB is used to adaptively incorporate these further variables and determine potential interactions.

First, the data are loaded from the **AER** package ([Kleiber and Zeileis 2008](#)) and only the subset of single-credit courses is excluded.

```
R> data("TeachingRatings", package = "AER")
R> tr <- subset(TeachingRatings, credits == "more")
```

The single-credit courses include elective modules that are quite different from the remaining courses (e.g., yoga, aerobics, or dance) and are hence omitted from the main analysis.

WLS estimation of the null model (with only an intercept) and the main effects model is carried out in a first step:

```
R> tr_null <- lm(eval ~ 1, data = tr, weights = students)
R> tr_lm <- lm(eval ~ beauty + gender + minority + native + tenure + division,
+ data = tr, weights = students)
```

Then, the model-based tree can be estimated with `lmtree()` using only `beauty` as a regressor and all remaining variables for partitioning. For WLS estimation, we set `weights = students` and `caseweights = FALSE` (because the weights are only proportionality factors and do not signal exactly replicated observations).

```
R> (tr_tree <- lmtree(eval ~ beauty | minority + age + gender + division +
+ native + tenure, data = tr, weights = students, caseweights = FALSE))
```

Linear model tree

Model formula:

```
eval ~ beauty | minority + age + gender + division + native +
      tenure
```

Fitted party:

```
[1] root
| [2] gender in female
| | [3] age <= 40: n = 69
| | (Intercept) beauty
| | 4.0137 0.1222
| | [4] age > 40
| | | [5] division in lower: n = 36
| | | (Intercept) beauty
| | | 3.5900 0.4033
| | | [6] division in upper: n = 81
| | | (Intercept) beauty
| | | 3.7752 -0.1976
| [7] gender in male
| | [8] age <= 50: n = 113
| | (Intercept) beauty
| | 3.9968 0.1292
| | [9] age > 50: n = 137
| | (Intercept) beauty
| | 4.0857 0.5028
```

Number of inner nodes: 4

Number of terminal nodes: 5

Number of parameters per node: 2

Objective function (residual sum of squares): 2752

The resulting tree can be visualized by `plot(tr_tree)` and is shown in Figure 5. This shows that despite age not having a significant main effect (as reported by [Hamermesh and Parker 2005](#)), it clearly plays an important role: While the correlation of teaching rating and beauty

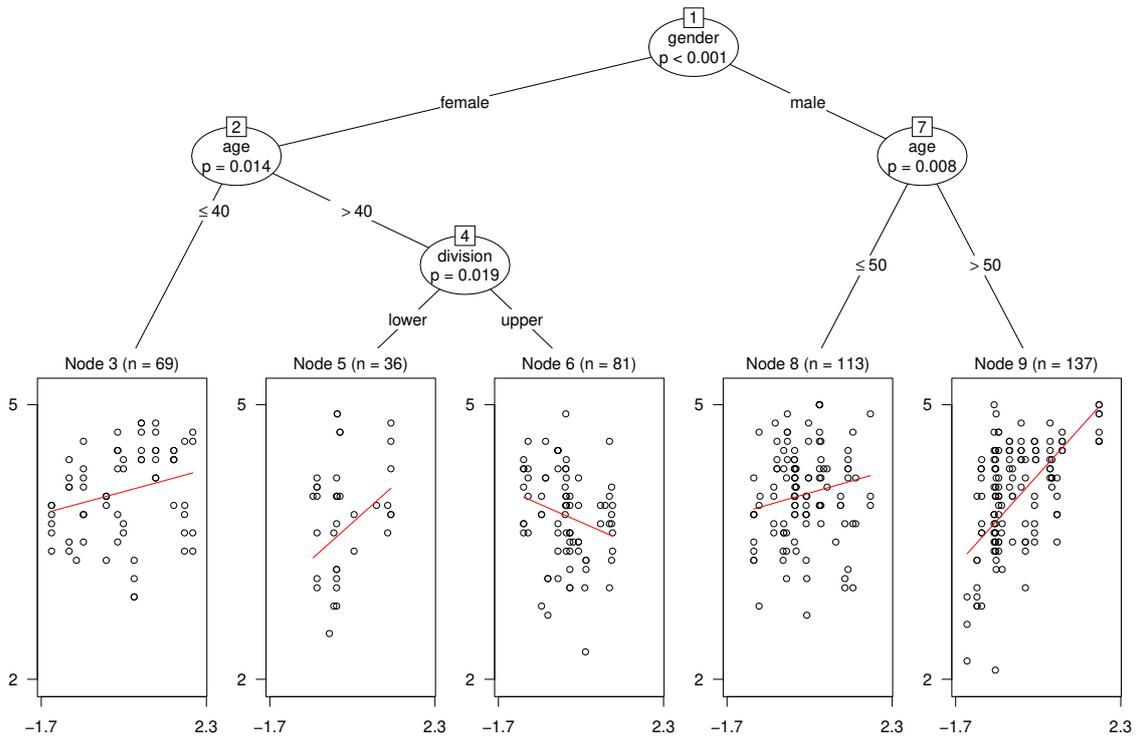

Figure 5: WLS-based tree for the teaching ratings data. The plots in the leaves show scatterplots for teaching rating by beauty score.

score is rather moderate for younger professors, there is a clear correlation for older professors (with the cutoff age somewhat lower for female professors).

```
R> coef(tr_lm)[2]
```

```
beauty
0.2826
```

```
R> coef(tr_tree)[, 2]
```

```
      3      5      6      8      9
0.1222 0.4033 -0.1976 0.1292 0.5028
```

The  $R^2$  of the tree is also clearly improved over the main effects model:

```
R> 1 - c(deviance(tr_lm), deviance(tr_tree))/deviance(tr_null)
```

```
[1] 0.2713 0.3820
```

#### 4.4. Titanic survival data

To illustrate how differences in treatment effects can be captured by MOB, the Titanic survival data is considered: The question is whether “women and children first” is applied in the same

way for all subgroups of the passengers of the Titanic. Or, in other words, whether the effectiveness of preferential treatment for women/children differed across subgroups.

The Titanic data is provided in base R as a contingency table and transformed here to a 'data.frame' for use with `glmtree()`:

```
R> data("Titanic", package = "datasets")
R> ttnc <- as.data.frame(Titanic)
R> ttnc <- ttnc[rep(1:nrow(ttnc), ttnc$Freq), 1:4]
R> names(ttnc)[2] <- "Gender"
R> ttnc <- transform(ttnc, Treatment = factor(
+   Gender == "Female" | Age == "Child", levels = c(FALSE, TRUE),
+   labels = c("Male&Adult", "Female|Child")))
```

The data provides factors `Survived` (yes/no), `Class` (1st, 2nd, 3rd, crew), `Gender` (male, female), and `Age` (child, adult). Additionally, a factor `Treatment` is added that distinguishes women/children from male adults.

To investigate how the preferential treatment effect (`Survived ~ Treatment`) differs across the remaining explanatory variables, the following logistic-regression-based tree is considered. The significance level of `alpha = 0.01` is employed here to avoid overfitting and separation problems in the logistic regression.

```
R> ttnc_tree <- glmtree(Survived ~ Treatment | Class + Gender + Age,
+   data = ttnc, family = binomial, alpha = 0.01)
R> ttnc_tree
```

Generalized linear model tree (family: binomial)

Model formula:

`Survived ~ Treatment | Class + Gender + Age`

Fitted party:

```
[1] root
| [2] Class in 1st, 2nd, Crew
| | [3] Class in 1st, Crew: n = 1210
| | (Intercept) TreatmentFemale|Child
| | -1.152 4.318
| | [4] Class in 2nd: n = 285
| | (Intercept) TreatmentFemale|Child
| | -2.398 4.477
| [5] Class in 3rd: n = 706
| (Intercept) TreatmentFemale|Child
| -1.641 1.327
```

Number of inner nodes: 2

Number of terminal nodes: 3

Number of parameters per node: 2

Objective function (negative log-likelihood): 1061

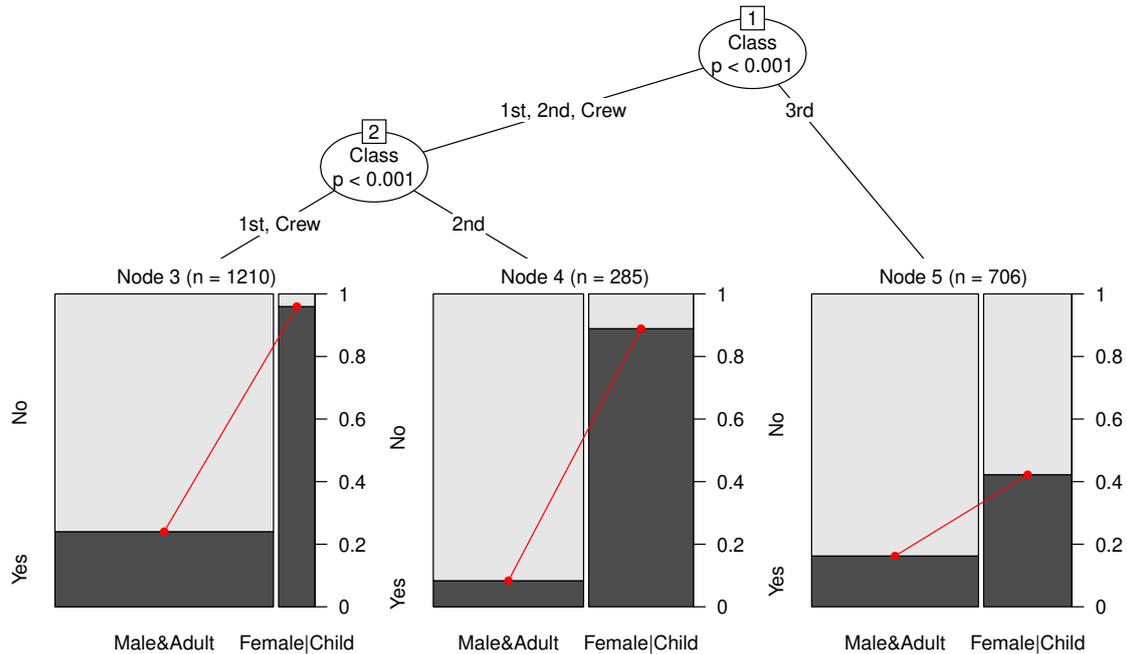

Figure 6: Logistic-regression-based tree for the Titanic survival data. The plots in the leaves give spinograms for survival status versus preferential treatment (women or children).

This shows that the treatment differs strongly across passengers classes, see also the result of `plot(ttnc_tree)` in Figure 6. The treatment effect is much lower in the 3rd class where women/children still have higher survival rates than adult men but the odds ratio is much lower compared to all remaining classes. The split between the 2nd and the remaining two classes (1st, crew) is due to a lower overall survival rate (intercepts of -2.4 and -1.64, respectively) while the odds ratios associated with the preferential treatment are rather similar (4.48 and 1.33, respectively).

Another option for assessing the class effect would be to immediately split into all four classes rather than using recursive binary splits. This can be obtained by setting `catsplit = "multiway"` in the `glmtree()` call above. This yields a tree with just a single split but four kid nodes.

#### 4.5. German breast cancer data

To illustrate that the MOB approach can also be used beyond (generalized) linear regression models, it is employed in the following to analyze censored survival times among German women with positive node breast cancer. The data is available in the **TH.data** package and the survival time is transformed from days to years:

```
R> data("GBSG2", package = "TH.data")
R> GBSG2$time <- GBSG2$time/365
```

For regression a parametric Weibull regression based on the `survreg()` function from the **survival** package (Therneau 2015) is used. A fitting function for `mob()` can be easily set up:

```
R> library("survival")
R> wbgreg <- function(y, x, start = NULL, weights = NULL, offset = NULL, ...) {
+   survreg(y ~ 0 + x, weights = weights, dist = "weibull", ...)
+ }
```

As the **survreg** package currently does not provide a `logLik()` method for ‘survreg’ objects, this needs to be added here:

```
R> logLik.survreg <- function(object, ...)
+   structure(object$loglik[2], df = sum(object$df), class = "logLik")
```

Without the `logLik()` method, `mob()` would not know how to extract the optimized objective function from the fitted model.

With the functions above available, a censored Weibull-regression-tree can be fitted: The dependent variable is the censored survival time and the two regressor variables are the main risk factor (number of positive lymph nodes) and the treatment variable (hormonal therapy). All remaining variables are used for partitioning: age, tumor size and grade, progesterone and estrogen receptor, and menopausal status. The minimal segment size is set to 80.

```
R> gbsg2_tree <- mob(Surv(time, cens) ~ horTh + pnodes | age + tsize +
+   tgrade + progrec + estrec + menostat, data = GBSG2,
+   fit = wbgreg, control = mob_control(minsize = 80))
```

Based on progesterone receptor, a tree with two leaves is found:

```
R> gbsg2_tree
```

Model-based recursive partitioning (wbgreg)

Model formula:

```
Surv(time, cens) ~ horTh + pnodes | age + tsize + tgrade + progrec +
  estrec + menostat
```

Fitted party:

```
[1] root
| [2] progrec <= 24: n = 299
|   x(Intercept)   xhorThyes   xpnodes
|   1.77331        0.17364     -0.06535
| [3] progrec > 24: n = 387
|   x(Intercept)   xhorThyes   xpnodes
|   1.9730         0.4451     -0.0302
```

```
Number of inner nodes: 1
Number of terminal nodes: 2
Number of parameters per node: 3
Objective function: 809.9
```

```
R> coef(gbsg2_tree)
```

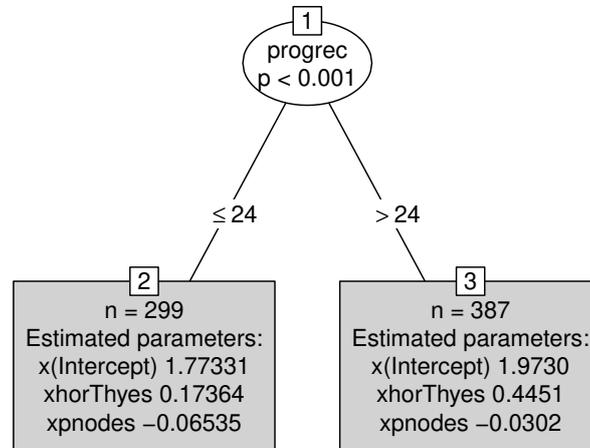

Figure 7: Censored Weibull-regression-based tree for the German breast cancer data. The plots in the leaves report the estimated regression coefficients.

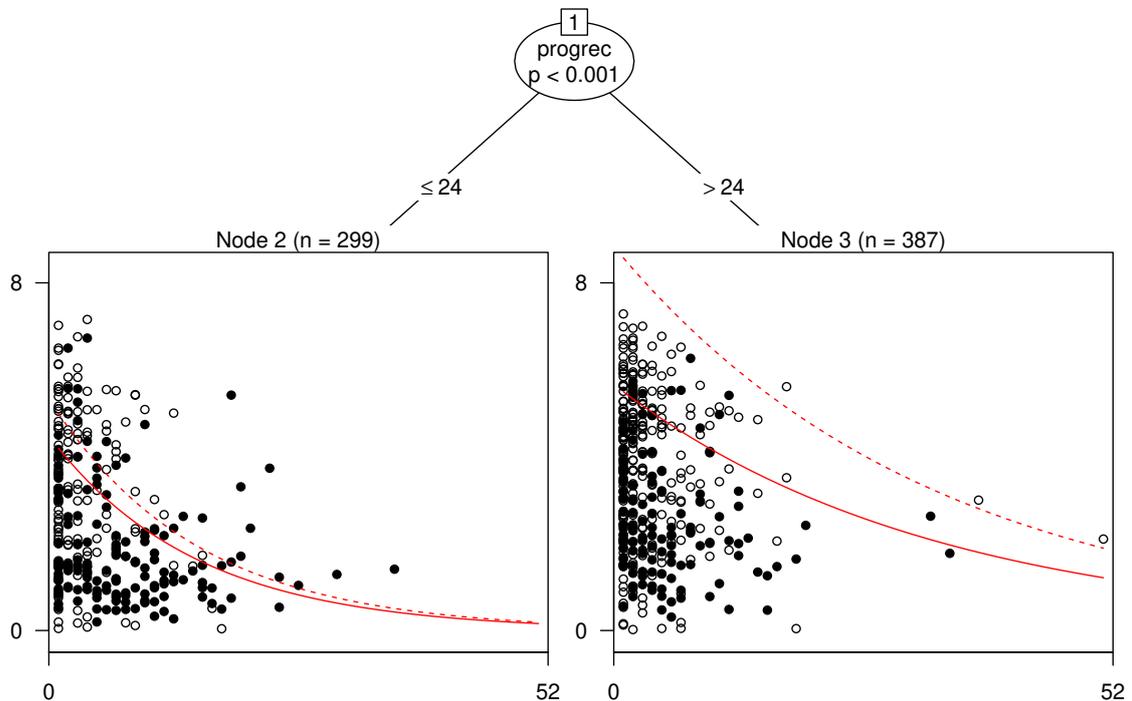

Figure 8: Censored Weibull-regression-based tree for the German breast cancer data. The plots in the leaves depict censored (hollow) and uncensored (solid) survival time by number of positive lymph nodes along with fitted median survival for patients with (dashed line) and without (solid line) hormonal therapy.

```

  x(Intercept) xhorThyes  xpnodes
2          1.773    0.1736 -0.06535
3          1.973    0.4451 -0.03020

```

```
R> logLik(gbsg2_tree)
```

```
'log Lik.' -809.9 (df=9)
```

The visualization produced by `plot(gbsg2_tree)` is shown in Figure 7. A nicer graphical display using a scatter plot (with indication of censoring) and fitted regression curves is shown in Figure 8. This uses a custom panel function whose code is too long and elaborate to be shown here. Interested readers are referred to the R code underlying the vignette.

The visualization shows that for higher progesterone receptor levels: (1) survival times are higher overall, (2) the treatment effect of hormonal therapy is higher, and (3) the negative effect of the main risk factor (number of positive lymph nodes) is less severe.

## 5. Setting up a new mobster

To conclude this vignette, we present another illustration that shows how to set up new mobster functionality from scratch. To do so, we implement the Bradley-Terry tree suggested by Strobl *et al.* (2011) “by hand”. The `psychotree` package already provides an easy-to-use mobster called `bttree()` but as an implementation exercise we recreate its functionality here.

The only inputs required are a suitable data set with paired comparisons (`Topmodel2007` from `psychotree`) and a parametric model for paired comparison data (`btmodel()` from `psychotools`, implementing the Bradley-Terry model). The latter optionally computes the empirical estimating functions and already comes with a suitable extractor method.

```
R> data("Topmodel2007", package = "psychotree")
R> library("psychotools")
```

The Bradley-Terry (or Bradley-Terry-Luce) model is a standard model for paired comparisons in social sciences. It parametrizes the probability  $\pi_{ij}$  for preferring some object  $i$  over another object  $j$  in terms of corresponding “ability” or “worth” parameters  $\theta_i$ :

$$\begin{aligned}\pi_{ij} &= \frac{\theta_i}{\theta_i + \theta_j} \\ \text{logit}(\pi_{ij}) &= \log(\theta_i) - \log(\theta_j)\end{aligned}$$

This model can be easily estimated by maximum likelihood as a logistic or log-linear GLM. This is the approach used internally by `btmodel()`.

The `Topmodel2007` data provide paired comparisons of attractiveness among the six finalists of the TV show *Germany's Next Topmodel 2007*: Barbara, Anni, Hana, Fiona, Mandy, Anja. The data were collected in a survey with 192 respondents at Universität Tübingen and the available covariates comprise gender, age, and familiarity with the TV show. The latter is assessed by three by yes/no questions: (1) Do you recognize the women?/Do you know the show? (2) Did you watch it regularly? (3) Did you watch the final show?/Do you know who won?

To fit the Bradley-Terry tree to the data, the available building blocks just have to be tied together. First, we set up the basic/simple model fitting interface described in Section 3.2:

```
R> btfit1 <- function(y, x = NULL, start = NULL, weights = NULL,
+   offset = NULL, ...) btmodel(y, ...)
```

The function `btfit1()` simply calls `btmodel()` ignoring all arguments except `y` as the others are not needed here. No more processing is required because ‘`btmodel`’ objects come with a `coef()`, `logLik()`, and `estfun()` method. Hence, we can call `mob()` now specifying the response and the partitioning variable (and no regressors because there are no regressors in this model).

```
R> bt1 <- mob(preference ~ 1 | gender + age + q1 + q2 + q3,
+   data = Topmodel2007, fit = btfit1)
```

An alternative way to fit the exact same tree somewhat more quickly would be to employ the extended interface described in Section 3.2:

```
R> btfit2 <- function(y, x = NULL, start = NULL, weights = NULL,
+   offset = NULL, ..., estfun = FALSE, object = FALSE) {
+   rval <- btmodel(y, ..., estfun = estfun, vcov = object)
+   list(
+     coefficients = rval$coefficients,
+     objfun = -rval$loglik,
+     estfun = if(estfun) rval$estfun else NULL,
+     object = if(object) rval else NULL
+   )
+ }
```

Still `btmodel()` is employed for fitting the model but the quantities `estfun` and `vcov` are only computed if they are really required. This may save some computation time – about 20% on the authors’ machine at the time of writing – when computing the tree:

```
R> bt2 <- mob(preference ~ 1 | gender + age + q1 + q2 + q3,
+   data = Topmodel2007, fit = btfit2)
```

The speed-up is not huge but comes almost for free: just a few additional lines of code in `btfit2()` are required. For other models where it is more costly to set up a full model (with variance-covariance matrix, predictions, residuals, etc.) larger speed-ups are also possible.

Both trees, `bt1` and `bt2`, are equivalent (except for the details of the fitting function). Hence, in the following we only explore `bt2`. However, the same code can be applied to `bt1` as well.

Many tools come completely for free and are inherited from the general ‘`modelparty`’/‘`party`’. For example, both printing (`print(bt2)`) and plotting (`plot(bt2)`) shows the estimated parameters in the terminal nodes which can also be extracted by the `coef()` method:

```
R> bt2
```

Model-based recursive partitioning (btfit2)

Model formula:

```
preference ~ 1 | gender + age + q1 + q2 + q3
```

Fitted party:

```
[1] root
| [2] age <= 52
| | [3] q2 in no
| | | [4] gender in female: n = 56
| | |   Barbara   Anni   Hana   Fiona   Mandy
| | |   0.9475  0.7246  0.4452  0.6350 -0.4965
| | | [5] gender in male: n = 71
| | |   Barbara   Anni   Hana   Fiona   Mandy
| | |   0.43866  0.08877  0.84629  0.69424 -0.10003
| | [6] q2 in yes: n = 35
| |   Barbara   Anni   Hana   Fiona   Mandy
| |   1.3378  1.2318  2.0499  0.8339  0.6217
| [7] age > 52: n = 30
|   Barbara   Anni   Hana   Fiona   Mandy
|   0.2178 -1.3166 -0.3059 -0.2591 -0.2357
```

Number of inner nodes: 3

Number of terminal nodes: 4

Number of parameters per node: 5

Objective function: 1829

```
R> coef(bt2)
```

```
   Barbara   Anni   Hana   Fiona   Mandy
4  0.9475  0.72459  0.4452  0.6350 -0.4965
5  0.4387  0.08877  0.8463  0.6942 -0.1000
6  1.3378  1.23183  2.0499  0.8339  0.6217
7  0.2178 -1.31663 -0.3059 -0.2591 -0.2357
```

The corresponding visualization is shown in the upper panel of Figure 9. In all cases, the estimated coefficients on the logit scale omitting the fixed zero reference level (Anja) are reported. To show the corresponding worth parameters  $\theta_i$  including the reference level, one can simply provide a small panel function `worthf()`. This applies the `worth()` function from **psychotools** to the fitted-model object stored in the `info` slot of each node, yielding the lower panel in Figure 9.

```
R> worthf <- function(info) paste(info$object$labels,
+   format(round(worth(info$object), digits = 3)), sep = ": ")
R> plot(bt2, FUN = worthf)
```

To show a graphical display of these worth parameters rather than printing their numerical values, one can use a simply glyph-style plot. A simply way to generate these is to use the

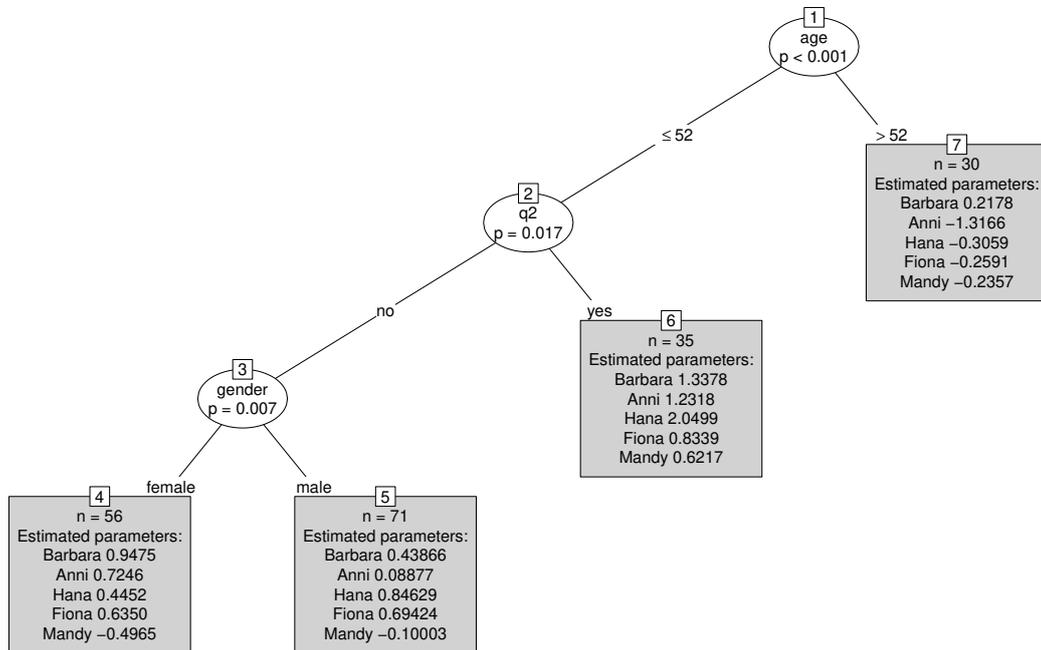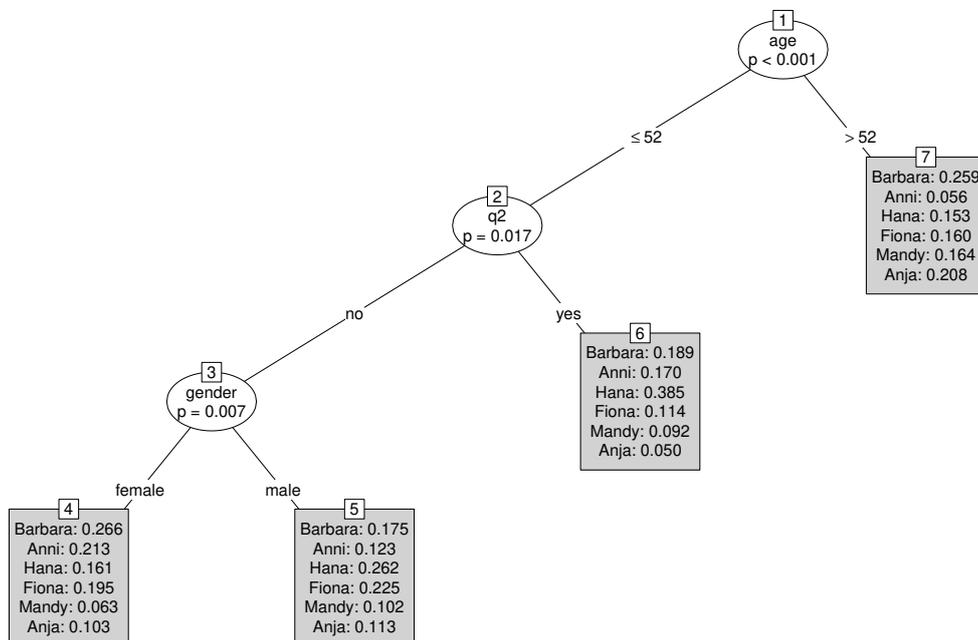

Figure 9: Bradley-Terry-based tree for the topmodel attractiveness data. The default plot (upper panel) reports the estimated coefficients on the log scale while the adapted plot (lower panel) shows the corresponding worth parameters.

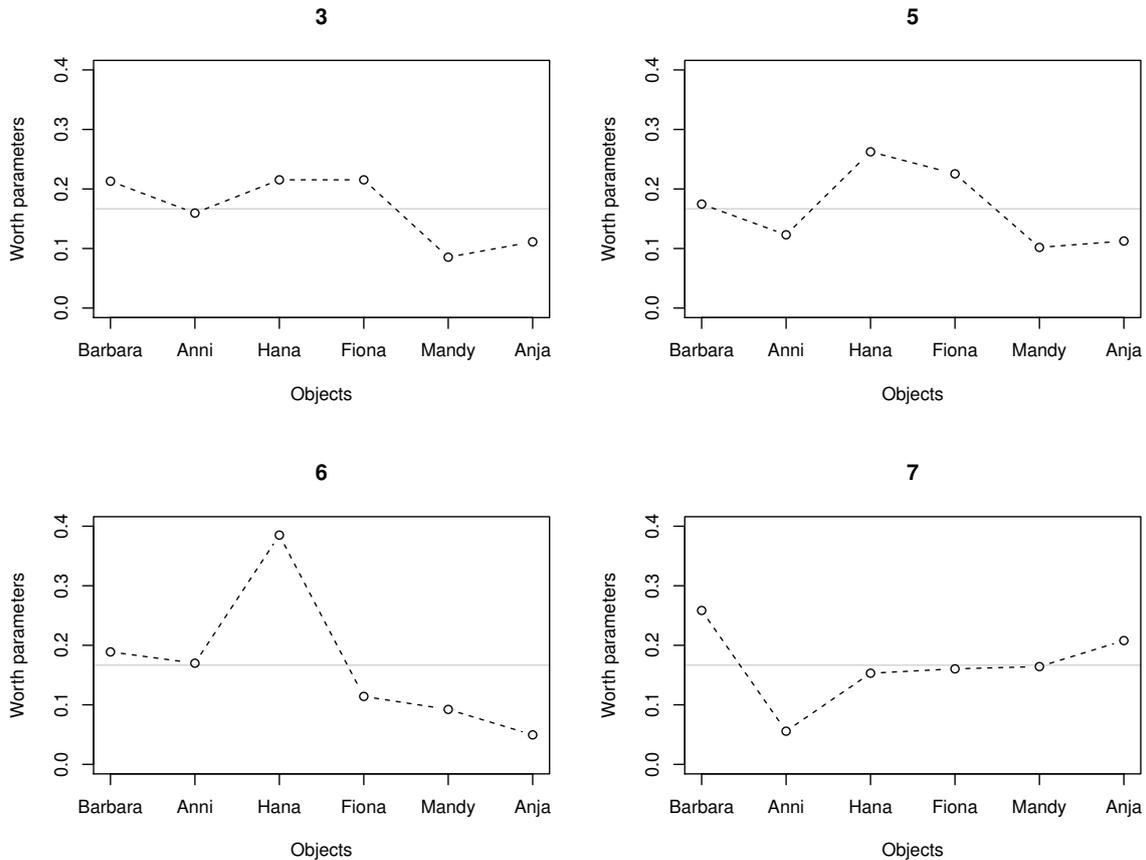

Figure 10: Worth parameters in the terminal nodes of the Bradley-Terry-based tree for the topmodel attractiveness data.

`plot()` method for ‘`btmodel`’ objects from **partykit** and `nodeapply` this to all terminal nodes (see Figure 10):

```
R> par(mfrow = c(2, 2))
R> nodeapply(bt2, ids = c(3, 5, 6, 7), FUN = function(n)
+   plot(n$info$object, main = n$id, ylim = c(0, 0.4)))
```

Alternatively, one could set up a proper panel-generating function in **grid** that allows to create the glyphs within the terminal nodes of the tree (see Figure 11). As the code for this panel-generating function `node_btplot()` is too complicated to display within the vignette, we refer interested readers to the underlying code. Given this panel-generating function Figure 11 can be generated with

```
R> plot(bt2, drop = TRUE, tnex = 2,
+   terminal_panel = node_btplot(bt2, abbreviate = 1, yscale = c(0, 0.5)))
```

Finally, to illustrate how different predictions can be easily computed, we set up a small data set with three new individuals:

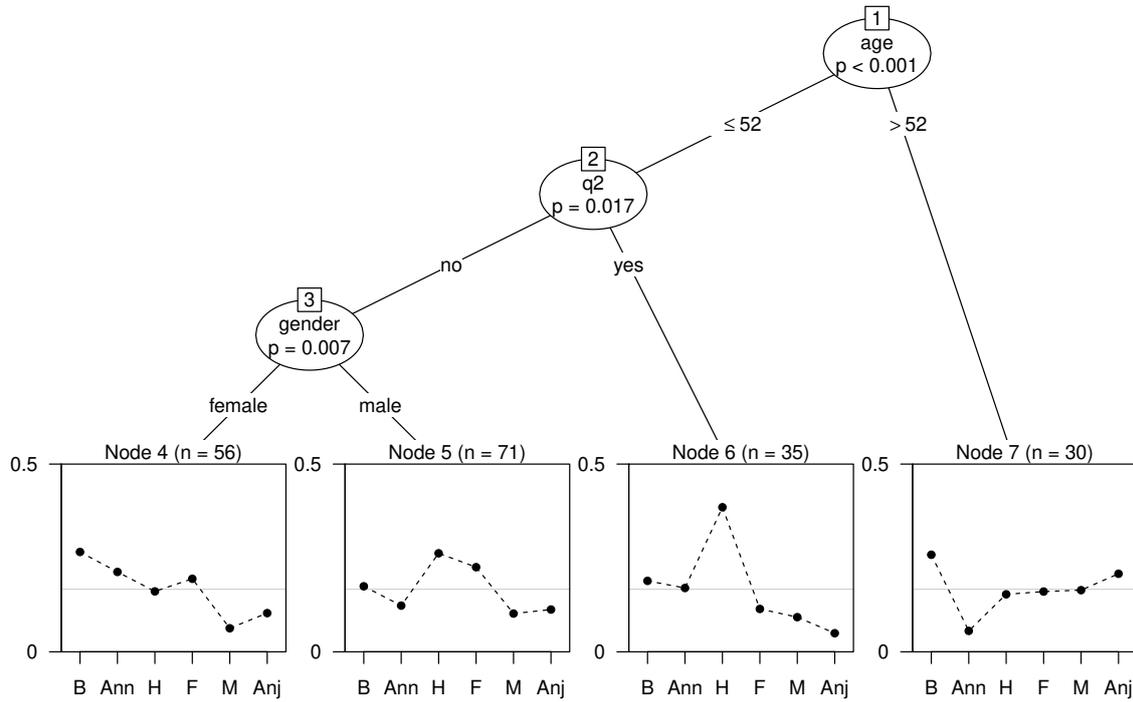

Figure 11: Bradley-Terry-based tree for the topmodel attractiveness data with visualizations of the worth parameters in the terminal nodes.

```

age gender q1 q2 q3
1 60 male no no no
2 25 female no no no
3 35 female no yes no

```

For these we can easily compute (1) the predicted node ID, (2) the corresponding worth parameters, (3) the associated ranks.

```
R> tm
```

```

age gender q1 q2 q3
1 60 male no no no
2 25 female no no no
3 35 female no yes no

```

```
R> predict(bt2, tm, type = "node")
```

```

1 2 3
7 4 6

```

```
R> predict(bt2, tm, type = function(object) t(worth(object)))
```

|   | Barbara | Anni    | Hana   | Fiona  | Mandy   | Anja    |
|---|---------|---------|--------|--------|---------|---------|
| 1 | 0.2585  | 0.05573 | 0.1531 | 0.1605 | 0.16427 | 0.20792 |
| 2 | 0.2659  | 0.21278 | 0.1609 | 0.1945 | 0.06275 | 0.10310 |
| 3 | 0.1889  | 0.16993 | 0.3851 | 0.1142 | 0.09232 | 0.04958 |

```
R> predict(bt2, tm, type = function(object) t(rank(-worth(object))))
```

|   | Barbara | Anni | Hana | Fiona | Mandy | Anja |
|---|---------|------|------|-------|-------|------|
| 1 | 1       | 6    | 5    | 4     | 3     | 2    |
| 2 | 1       | 2    | 4    | 3     | 6     | 5    |
| 3 | 2       | 3    | 1    | 4     | 5     | 6    |

This completes the tour of fitting, printing, plotting, and predicting the Bradley-Terry tree model. Convenience interfaces that employ code like shown above can be easily defined and collected in new packages such as **psychotree**.

## 6. Conclusion

The function `mob()` in the **partykit** package provides a new flexible and object-oriented implementation of the general algorithm for model-based recursive partitioning using **partykit**'s recursive partytioning infrastructure. New model fitting functions can be easily provided, especially if standard extractor functions (such as `coef()`, `estfun()`, `logLik()`, etc.) are available. The resulting model trees can then learned, visualized, investigated, and employed for predictions. To gain some efficiency in the computations and to allow for further customization (in particular specialized visualization and prediction methods), convenience interfaces `lmtree()` and `glmmtree()` are provided for recursive partitioning based on (generalized) linear models.

## References

- Bache K, Lichman M (2013). "UCI Machine Learning Repository." URL <http://archive.ics.uci.edu/ml/>.
- Bai J, Perron P (2003). "Computation and Analysis of Multiple Structural Change Models." *Journal of Applied Econometrics*, **18**, 1–22.
- Breiman L, Friedman JH (1985). "Estimating Optimal Transformations for Multiple Regression and Correlation." *Journal of the American Statistical Association*, **80**(391), 580–598.
- Genz A, Bretz F, Miwa T, Mi X, Leisch F, Scheipl F, Hothorn T (2015). *mvtnorm: Multivariate Normal and t Distributions*. R package version 1.0-3, URL <http://CRAN.R-project.org/package=mvtnorm>.
- Grün B, Kosmidis I, Zeileis A (2012). "Extended Beta Regression in R: Shaken, Stirred, Mixed, and Partitioned." *Journal of Statistical Software*, **48**(11), 1–25. URL <http://www.jstatsoft.org/v48/i11/>.

- Hamermesh DS, Parker A (2005). “Beauty in the Classroom: Instructors’ Pulchritude and Putative Pedagogical Productivity.” *Economics of Education Review*, **24**, 369–376.
- Hansen BE (1997). “Approximate Asymptotic  $p$  Values for Structural-Change Tests.” *Journal of Business & Economic Statistics*, **15**, 60–67.
- Hawkins DM (2001). “Fitting Multiple Change-Point Models to Data.” *Computational Statistics & Data Analysis*, **37**, 323–341.
- Hothorn T, Hornik K, Strobl C, Zeileis A (2015). *party: A Laboratory for Recursive Partitioning*. R package version 1.0-23, URL <http://CRAN.R-project.org/package=party>.
- Hothorn T, Leisch F, Zeileis A (2013). *modeltools: Tools and Classes for Statistical Models*. R package version 0.2-21, URL <http://CRAN.R-project.org/package=modeltools>.
- Hothorn T, Zeileis A (2015). *partykit: A Toolkit for Recursive Partitioning*. R package version 1.0-3, URL <http://CRAN.R-project.org/package=partykit>.
- Kleibler C, Zeileis A (2008). *Applied Econometrics with R*. Springer-Verlag, New York. URL <http://CRAN.R-project.org/package=AER>.
- Leisch F, Dimitriadou E (2012). *mlbench: Machine Learning Benchmark Problems*. R package version 2.1-1, URL <http://CRAN.R-project.org/package=mlbench>.
- Merkle EC, Fan J, Zeileis A (2014). “Testing for Measurement Invariance with Respect to an Ordinal Variable.” *Psychometrika*, **79**(4), 569–584. doi:10.1007/S11336-013-9376-7.
- Merkle EC, Zeileis A (2013). “Tests of Measurement Invariance without Subgroups: A Generalization of Classical Methods.” *Psychometrika*, **78**(1), 59–82. doi:10.1007/s11336-012-9302-4.
- Meyer D, Zeileis A, Hornik K (2006). “The Strucplot Framework: Visualizing Multi-Way Contingency Tables with **vcd**.” *Journal of Statistical Software*, **17**(3), 1–48. URL <http://www.jstatsoft.org/v17/i03/>.
- R Core Team (2013). *R: A Language and Environment for Statistical Computing*. R Foundation for Statistical Computing, Vienna, Austria. URL <http://www.R-project.org/>.
- Strobl C, Kopf J, Zeileis A (2015). “Rasch Trees: A New Method for Detecting Differential Item Functioning in the Rasch Model.” *Psychometrika*, **80**(2), 289–316. doi:10.1007/s11336-013-9388-3.
- Strobl C, Wickelmaier F, Zeileis A (2011). “Accounting for Individual Differences in Bradley-Terry Models by Means of Recursive Partitioning.” *Journal of Educational and Behavioral Statistics*, **36**(2), 135–153.
- Su X, Wang M, Fan J (2004). “Maximum Likelihood Regression Trees.” *Journal of Computational and Graphical Statistics*, **13**, 586–598.
- Therneau TM (2015). *survival: A Package for Survival Analysis in S*. R package version 2.38-3, URL <http://CRAN.R-project.org/package=survival>.

- Zeileis A (2005). “A Unified Approach to Structural Change Tests Based on ML Scores,  $F$  Statistics, and OLS Residuals.” *Econometric Reviews*, **24**, 445–466. doi:10.1080/07474930500406053.
- Zeileis A (2006). “Object-Oriented Computation of Sandwich Estimators.” *Journal of Statistical Software*, **16**(9), 1–16. URL <http://www.jstatsoft.org/v16/i09/>.
- Zeileis A, Croissant Y (2010). “Extended Model Formulas in R: Multiple Parts and Multiple Responses.” *Journal of Statistical Software*, **34**(1), 1–13. URL <http://www.jstatsoft.org/v34/i01/>.
- Zeileis A, Hornik K (2007). “Generalized M-Fluctuation Tests for Parameter Instability.” *Statistica Neerlandica*, **61**(4), 488–508. doi:10.1111/j.1467-9574.2007.00371.x.
- Zeileis A, Hothorn T, Hornik K (2008). “Model-Based Recursive Partitioning.” *Journal of Computational and Graphical Statistics*, **17**(2), 492–514. doi:10.1198/106186008X319331.
- Zeileis A, Leisch F, Hornik K, Kleiber C (2002). “**strucchange**: An R Package for Testing for Structural Change in Linear Regression Models.” *Journal of Statistical Software*, **7**(2), 1–38. URL <http://www.jstatsoft.org/v07/i02/>.

**Affiliation:**

Achim Zeileis  
Department of Statistics  
Faculty of Economics and Statistics  
Universität Innsbruck  
Universitätsstr. 15  
6020 Innsbruck, Austria  
E-mail: [Achim.Zeileis@R-project.org](mailto:Achim.Zeileis@R-project.org)  
URL: <http://eeecon.uibk.ac.at/~zeileis/>

Torsten Hothorn  
Institut für Epidemiologie, Biostatistik und Prävention  
Universität Zürich  
Hirschengraben 84  
CH-8001 Zürich, Switzerland  
E-mail: [Torsten.Hothorn@R-project.org](mailto:Torsten.Hothorn@R-project.org)  
URL: <http://user.math.uzh.ch/hothorn/>
