# Supplementary material for: The Power of Unbiased Recursive Partitioning: A Unifying View of CTree, MOB, and GUIDE
Source: arXiv:1906.10179 ancillary file (2019-06-24)
Supplement: Supplementary file 4 [file partykit.pdf]

# partykit: A Toolkit for Recursive Partytioning

Achim Zeileis  
Universität Innsbruck

Torsten Hothorn  
Universität Zürich

---

## Abstract

The **partykit** package provides a flexible toolkit with infrastructure for learning, representing, summarizing, and visualizing a wide range of tree-structured regression and classification models. The functionality encompasses: (a) Basic infrastructure for *representing* trees (inferred by any algorithm) so that unified **print/plot/predict** methods are available. (b) Dedicated methods for trees with *constant fits* in the leaves (or terminal nodes) along with suitable coercion functions to create such tree models (e.g., by **rpart**, **RWeka**, PMML). (c) A reimplementaion of *conditional inference trees* (**ctree**, originally provided in the **party** package). (d) An extended reimplementaion of *model-based recursive partitioning* (**mob**, also originally in **party**) along with dedicated methods for trees with parametric models in the leaves. This vignette gives a brief overview of the package and discusses in detail the generic infrastructure for representing trees (a). Items (b)–(d) are discussed in the remaining vignettes in the package.

*Keywords:* recursive partitioning, regression trees, classification trees, decision trees.

---

## 1. Overview

In the more than fifty years since [Morgan and Sonquist \(1963\)](#) published their seminal paper on “automatic interaction detection”, a wide range of methods has been suggested that is usually termed “recursive partitioning” or “decision trees” or “tree(-structured) models” etc. Particularly influential were the algorithms CART (classification and regression trees, [Breiman, Friedman, Olshen, and Stone 1984](#)), C4.5 ([Quinlan 1993](#)), QUEST/GUIDE ([Loh and Shih 1997](#); [Loh 2002](#)), and CTree ([Hothorn, Hornik, and Zeileis 2006](#)) among many others (see [Loh 2014](#), for a recent overview). Reflecting the heterogeneity of conceptual algorithms, a wide range of computational implementations in various software systems emerged: Typically the original authors of an algorithm also provide accompanying software but many software systems, e.g., including **Weka** ([Witten and Frank 2005](#)) or R ([R Core Team 2013](#)), also provide collections of various types of trees. Within R the list of prominent packages includes **rpart** ([Therneau and Atkinson 1997](#), implementing the CART algorithm), **mvpart** ([De’ath 2014](#), for multivariate CART), **RWeka** ([Hornik, Buchta, and Zeileis 2009](#), containing interfaces to J4.8, M5’, LMT from **Weka**), and **party** ([Hothorn, Hornik, Strobl, and Zeileis 2015](#), implementing CTree and MOB) among many others. See the CRAN task view “Machine Learning” ([Hothorn 2014](#)) for an overview.

All of these algorithms and software implementations have to deal with very similar challenges. However, due to the fragmentation of the communities in which the corresponding research is published – ranging from statistics over machine learning to various applied fields

– many discussions of the algorithms do not reuse established theoretical results and terminology. Similarly, there is no common “language” for the software implementations and different solutions are provided by different packages (even within R) with relatively little reuse of code. The **partykit** tries to address the latter point and improve the computational situation by providing a common unified infrastructure for recursive partytioning in the R system for statistical computing. In particular, **partykit** provides tools for representing fitted trees along with printing, plotting, and computing predictions. The design principles are:

- One ‘agnostic’ base class (`‘party’`) which can encompass an extremely wide range of different types of trees.
- Subclasses for important types of trees, e.g., trees with constant fits (`‘constparty’`) or with parametric models (`‘modelparty’`) in each terminal node (or leaf).
- Nodes are recursive objects, i.e., a node can contain child nodes.
- Keep the (learning) data out of the recursive node and split structure.
- Basic printing, plotting, and predicting for raw node structure.
- Customization via suitable panel or panel-generating functions.
- Coercion from existing object classes in R (`rpart`, `J48`, etc.) to the new class.
- Usage of simple/fast S3 classes and methods.

In addition to all of this generic infrastructure, two specific tree algorithms are implemented in **partykit** as well: `ctree()` for conditional inference trees (Hothorn *et al.* 2006) and `mob()` for model-based recursive partitioning (Zeileis, Hothorn, and Hornik 2008).

This vignette (`"partykit"`) introduces the basic `‘party’` class and associated infrastructure while three further vignettes discuss the tools built on top of it: `"constparty"` covers the eponymous class for constant-fit trees along with suitable coercion functions, and `"ctree"` and `"mob"` discuss the new `ctree()` and `mob()` implementations, respectively. Each of the vignettes can be viewed within R via `vignette("name", package = "partykit")`.

Normal users reading this vignette will typically be interested only in the motivating example in Section 2 while the remaining sections are intended for programmers who want to build infrastructure on top of **partykit**.

## 2. Motivating example

### 2.1. Data

To illustrate how **partykit** can be used to represent trees, we employ a simple artificial data set taken from Witten and Frank (2005). It concerns the conditions suitable for playing some unspecified game:

```
R> data("WeatherPlay", package = "partykit")
R> WeatherPlay
```

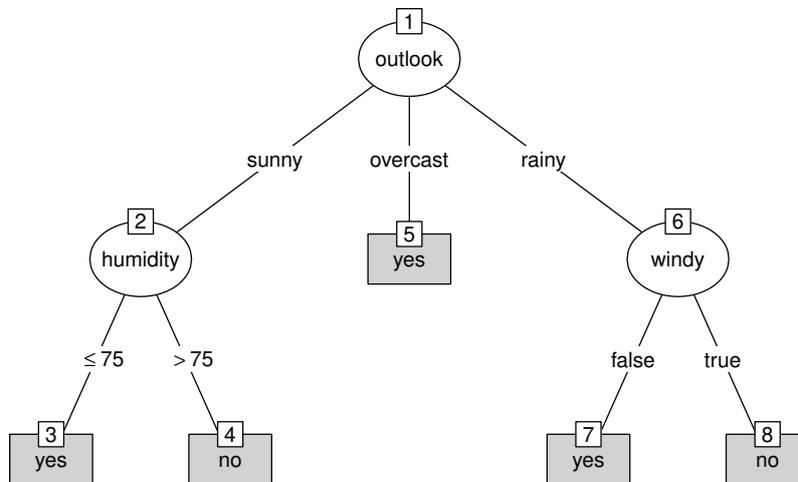

Figure 1: Decision tree for play decision based on weather conditions in WeatherPlay data.

|    | outlook  | temperature | humidity | windy | play |
|----|----------|-------------|----------|-------|------|
| 1  | sunny    | 85          | 85       | false | no   |
| 2  | sunny    | 80          | 90       | true  | no   |
| 3  | overcast | 83          | 86       | false | yes  |
| 4  | rainy    | 70          | 96       | false | yes  |
| 5  | rainy    | 68          | 80       | false | yes  |
| 6  | rainy    | 65          | 70       | true  | no   |
| 7  | overcast | 64          | 65       | true  | yes  |
| 8  | sunny    | 72          | 95       | false | no   |
| 9  | sunny    | 69          | 70       | false | yes  |
| 10 | rainy    | 75          | 80       | false | yes  |
| 11 | sunny    | 75          | 70       | true  | yes  |
| 12 | overcast | 72          | 90       | true  | yes  |
| 13 | overcast | 81          | 75       | false | yes  |
| 14 | rainy    | 71          | 91       | true  | no   |

To represent the `play` decision based on the corresponding weather condition variables one could use the tree displayed in Figure 1. For now, it is ignored how this tree was inferred and it is simply assumed to be given.

To represent this tree (or recursive partition) in **partykit**, two basic building blocks are used: splits of class `'partysplit'` and nodes of class `'partynode'`. The resulting recursive partition can then be associated with a data set in an object of class `'party'`.

## 2.2. Splits

First, we employ the `partysplit()` function to create the three splits in the “play tree” from

Figure 1. The function takes the following arguments

```
partysplit(varid, breaks = NULL, index = NULL, ..., info = NULL)
```

where `varid` is an integer id (column number) of the variable used for splitting, e.g., 1L for outlook, 3L for humidity, 4L for windy etc. Then, `breaks` and `index` determine which observations are sent to which of the branches, e.g., `breaks = 75` for the humidity split. Apart from further arguments not shown above (and just comprised under ‘...’), some arbitrary information can be associated with a ‘`partysplit`’ object by passing it to the `info` argument. The three splits from Figure 1 can then be created via

```
R> sp_o <- partysplit(1L, index = 1:3)
R> sp_h <- partysplit(3L, breaks = 75)
R> sp_w <- partysplit(4L, index = 1:2)
```

For the numeric humidity variable the `breaks` are set while for the factor variables outlook and windy the information is supplied which of the levels should be associated with which of the branches of the tree.

### 2.3. Nodes

Second, we use these splits in the creation of the whole decision tree. In **partykit** a tree is represented by a ‘`partynode`’ object which is recursive in that it may have “kids” that are again ‘`partynode`’ objects. These can be created with the function

```
partynode(id, split = NULL, kids = NULL, ..., info = NULL)
```

where `id` is an integer identifier of the node number, `split` is a ‘`partysplit`’ object, and `kids` is a list of ‘`partynode`’ objects. Again, there are further arguments not shown (...) and arbitrary information can be supplied in `info`. The whole tree from Figure 1 can then be created via

```
R> pn <- partynode(1L, split = sp_o, kids = list(
+   partynode(2L, split = sp_h, kids = list(
+     partynode(3L, info = "yes"),
+     partynode(4L, info = "no"))),
+   partynode(5L, info = "yes"),
+   partynode(6L, split = sp_w, kids = list(
+     partynode(7L, info = "yes"),
+     partynode(8L, info = "no")))))
```

where the previously created ‘`partysplit`’ objects are used as splits and the nodes are simply numbered (depth first) from 1 to 8. For the terminal nodes of the tree there are no `kids` and the corresponding play decision is stored in the `info` argument. Printing the ‘`partynode`’ object reflects the recursive structure stored.

```
R> pn
```

```
[1] root
| [2] V1 in (-Inf,1]
| | [3] V3 <= 75 *
| | [4] V3 > 75 *
| [5] V1 in (1,2] *
| [6] V1 in (2, Inf]
| | [7] V4 <= 1 *
| | [8] V4 > 1 *
```

However, the displayed information is still rather raw as it has not yet been associated with the `WeatherPlay` data set.

## 2.4. Trees (or recursive partitions)

Therefore, in a third step the recursive tree structure stored in `pn` is coupled with the corresponding data in a ‘party’ object.

```
R> py <- party(pn, WeatherPlay)
R> print(py)
```

```
[1] root
| [2] outlook in sunny
| | [3] humidity <= 75: yes
| | [4] humidity > 75: no
| [5] outlook in overcast: yes
| [6] outlook in rainy
| | [7] windy in false: yes
| | [8] windy in true: no
```

Now, Figure 1 can easily be created by

```
R> plot(py)
```

In addition to `print()` and `plot()`, the `predict()` method can now be applied, yielding the predicted terminal node IDs.

```
R> predict(py, head(WeatherPlay))
```

```
1 2 3 4 5 6
4 4 5 7 7 8
```

In addition to the ‘partynode’ and the ‘data.frame’, the function `party()` takes several further arguments

```
party(node, data, fitted = NULL, terms = NULL, ..., info = NULL)
```

i.e., `fitted` values, a `terms` object, arbitrary additional `info`, and again some further arguments comprised in `...`

## 2.5. Methods and other utilities

The main idea about the ‘`party`’ class is that tedious tasks such as `print()`, `plot()`, `predict()` do not have to be reimplemented for every new kind of decision tree but can simply be reused. However, in addition to these three basic tasks (as already illustrated above) developers of tree model software also need further basic utilities for working with trees: e.g., functions for querying or subsetting the tree and for customizing printed/plotted output. Below, various utilities provided by the **partykit** package are introduced.

For querying the dimensions of the tree, three basic functions are available: `length()` gives the number of kid nodes of the root node, `depth()` the depth of the tree and `width()` the number of terminal nodes.

```
R> length(py)
```

```
[1] 8
```

```
R> width(py)
```

```
[1] 5
```

```
R> depth(py)
```

```
[1] 2
```

As decision trees can grow to be rather large, it is often useful to inspect only subtrees. These can be easily extracted using the standard `[]` or `[[` operators:

```
R> py[6]
```

```
[6] root
|   [7] windy in false: yes
|   [8] windy in true: no
```

The resulting object is again a full valid ‘`party`’ tree and can hence be printed (as above) or plotted (via `plot(py[6])`, see the left panel of Figure 2). Instead of using the integer node IDs for subsetting, node labels can also be used. By default these are just (character versions of) the node IDs but other names can be easily assigned:

```
R> py2 <- py
R> names(py2)
```

```
[1] "1" "2" "3" "4" "5" "6" "7" "8"
```

```
R> names(py2) <- LETTERS[1:8]
R> py2

[A] root
| [B] outlook in sunny
| | [C] humidity <= 75: yes
| | [D] humidity > 75: no
| [E] outlook in overcast: yes
| [F] outlook in rainy
| | [G] windy in false: yes
| | [H] windy in true: no
```

The function `nodeids()` queries the integer node IDs belonging to a ‘party’ tree. By default all IDs are returned but optionally only the terminal IDs (of the leaves) can be extracted.

```
R> nodeids(py)
```

```
[1] 1 2 3 4 5 6 7 8
```

```
R> nodeids(py, terminal = TRUE)
```

```
[1] 3 4 5 7 8
```

Often functions need to be applied to certain nodes of a tree, e.g., for extracting information. This is accommodated by a new generic function `nodeapply()` that follows the style of other R functions from the `apply` family and has methods for ‘party’ and ‘partynode’ objects. Furthermore, it needs a set of node IDs (often computed via `nodeids()`) and a function `FUN` that is applied to each of the requested ‘partynode’ objects, typically for extracting/formatting the `info` of the node.

```
R> nodeapply(py, ids = c(1, 7), FUN = function(n) n$info)
```

```
$`1`
NULL
```

```
$`7`
[1] "yes"
```

```
R> nodeapply(py, ids = nodeids(py, terminal = TRUE),
+   FUN = function(n) paste("Play decision:", n$info))
```

```
$`3`
[1] "Play decision: yes"
```

```
$`4`
[1] "Play decision: no"
```

```
$`5`
[1] "Play decision: yes"
```

```
$`7`
[1] "Play decision: yes"
```

```
$`8`
[1] "Play decision: no"
```

Similar to the functions applied in a `nodeapply()`, the `print()`, `predict()`, and `plot()` methods can be customized through panel function that format certain parts of the tree (such as header, footer, node, etc.). Hence, the same kind of panel function employed above can also be used for predictions:

```
R> predict(py, FUN = function(n) paste("Play decision:", n$info))
```

```

          1          2          3
"Play decision: no" "Play decision: no" "Play decision: yes"
          4          5          6
"Play decision: yes" "Play decision: yes" "Play decision: no"
          7          8          9
"Play decision: yes" "Play decision: no" "Play decision: yes"
         10         11         12
"Play decision: yes" "Play decision: yes" "Play decision: yes"
         13         14
"Play decision: yes" "Play decision: no"
```

As a variation of this approach, an extended formatting with multiple lines can be easily accomodated by supplying a character vector in every node:

```
R> print(py, terminal_panel = function(n)
+   c(", then the play decision is:", toupper(n$info)))
```

```
[1] root
| [2] outlook in sunny
| | [3] humidity <= 75, then the play decision is:
| |   YES
| | [4] humidity > 75, then the play decision is:
| |   NO
| [5] outlook in overcast, then the play decision is:
|   YES
| [6] outlook in rainy
| | [7] windy in false, then the play decision is:
| |   YES
| | [8] windy in true, then the play decision is:
| |   NO
```

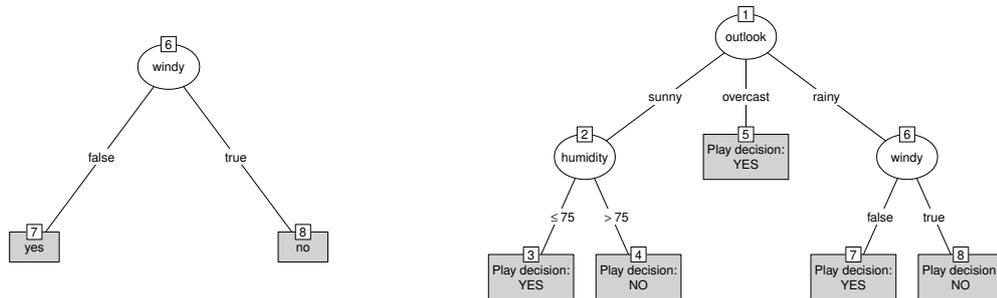

Figure 2: Visualization of subtree (left) and tree with custom text in terminal nodes (right).

The same type of approach can also be used in the default `plot()` method (with the main difference that the panel function operates on the `info` directly rather than on the `'party'node`).

```
R> plot(py, tp_args = list(FUN = function(i)
+   c("Play decision:", toupper(i))))
```

See the right panel of Figure 2 for the resulting graphic. Many more elaborate panel functions are provided in **partykit**, especially for not only showing text in the visualizations but also statistical graphics. Some of these are briefly illustrated in this and the other package vignettes. Programmers that want to write their own panel functions are advised to inspect the corresponding R source code to see how flexible (but sometimes also complicated) these panel functions are.

Finally, an important utility function is `nodeprune()` which allows to prune `'party'` trees. It takes a vector of node IDs and prunes all of their kids, i.e., making all the indicated node IDs terminal nodes.

```
R> nodeprune(py, 2)
```

```
[1] root
| [2] outlook in sunny: *
| [3] outlook in overcast: yes
| [4] outlook in rainy
| | [5] windy in false: yes
| | [6] windy in true: no
```

```
R> nodeprune(py, c(2, 6))
```

```
[1] root
| [2] outlook in sunny: *
| [3] outlook in overcast: yes
| [4] outlook in rainy: *
```

Note that for the pruned versions of this particular `'party'` tree, the new terminal nodes are displayed with a `*` rather than the play decision. This is because we did not store any play

decisions in the `info` of the inner nodes of `py`. We could have of course done so initially, or could do so now, or we might want to do so automatically. For the latter, we would have to know how predictions should be obtained from the data and this is briefly discussed at the end of this vignette and in more detail in `vignette("constparty", package = "partykit")`.

### 3. Technical details

#### 3.1. Design principles

To facilitate reading of the subsequent sections, two design principles employed in the creation of **partykit** are briefly explained.

1. Many helper utilities are encapsulated in functions that follow a simple naming convention. To extract/compute some information *foo* from splits, nodes, or trees, **partykit** provides `foo_split`, `foo_node`, `foo_party` functions (that are applicable to ‘`partysplit`’, ‘`party`’, and ‘`party`’ objects, respectively).

An example for the information *foo* might be `kidids` or `info`. Hence, in the printing example above using `info_node(n)` rather than `n$info` for a node `n` would have been the preferred syntax; at least when programming new functionality on top of **partykit**.

2. As already illustrated above, printing and plotting relies on *panel functions* that visualize and/or format certain aspects of the resulting display, e.g., that of inner nodes, terminal nodes, headers, footers, etc. Furthermore, arguments like `terminal_panel` can also take *panel-generating functions*, i.e., functions that produce a panel function when applied to the ‘`party`’ object.

#### 3.2. Splits

##### *Overview*

A split is basically a function that maps data – or more specifically a partitioning variable – to daughter nodes. Objects of class ‘`partysplit`’ are designed to represent such functions and are set up by the `partysplit()` constructor. For example, a binary split in the numeric partitioning variable `humidity` (the 3rd variable in `WeatherPlay`) at the breakpoint 75 can be created (as above) by

```
R> sp_h <- partysplit(3L, breaks = 75)
R> class(sp_h)
```

```
[1] "partysplit"
```

The internal structure of class ‘`partysplit`’ contains information about the partitioning variable, the splitpoints (or cutpoints or breakpoints), the handling of splitpoints, the treatment of observations with missing values and the kid nodes to send observations to:

```
R> unclass(sp_h)
```

```

$varid
[1] 3

$breaks
[1] 75

$index
NULL

$right
[1] TRUE

$prob
NULL

$info
NULL

```

Here, the splitting rule is  $\text{humidity} \leq 75$ :

```
R> character_split(sp_h, data = WeatherPlay)
```

```

$name
[1] "humidity"

$levels
[1] "<= 75" "> 75"

```

This representation of splits is completely abstract and, most importantly, independent of any data. Now, data comes into play when we actually want to perform splits:

```
R> kidids_split(sp_h, data = WeatherPlay)
```

```
[1] 2 2 2 2 2 1 1 2 1 2 1 2 1 2
```

For each observation in `WeatherPlay` the split is performed and the number of the kid node to send this observation to is returned. Of course, this is a very complicated way of saying

```
R> as.numeric(!(WeatherPlay$humidity <= 75)) + 1
```

```
[1] 2 2 2 2 2 1 1 2 1 2 1 2 1 2
```

### *Mathematical notation*

To explain the splitting strategy more formally, we employ some mathematical notation. **partykit** considers a split to represent a function  $f$  mapping an element  $x = (x_1, \dots, x_p)$  of a

$p$ -dimensional sample space  $\mathcal{X}$  into a set of  $k$  daughter nodes  $\mathcal{D} = \{d_1, \dots, d_k\}$ . This mapping is defined as a composition  $f = h \circ g$  of two functions  $g : \mathcal{X} \rightarrow \mathcal{I}$  and  $h : \mathcal{I} \rightarrow \mathcal{D}$  with index set  $\mathcal{I} = \{1, \dots, l\}, l \geq k$ .

Let  $\mu = (-\infty, \mu_1, \dots, \mu_{l-1}, \infty)$  denote the split points ( $(\mu_1, \dots, \mu_{l-1}) = \text{breaks}$ ). We are interested to split according to the information contained in the  $i$ -th element of  $x$  ( $i = \text{varid}$ ). For numeric  $x_i$ , the split points are also numeric. If  $x_i$  is a factor at levels  $1, \dots, K$ , the default split points are  $\mu = (-\infty, 1, \dots, K - 1, \infty)$ .

The function  $g$  essentially determines, which of the intervals (defined by  $\mu$ ) the value  $x_i$  is contained in ( $I$  denotes the indicator function here):

$$x \mapsto g(x) = \sum_{j=1}^l j I_{\mathcal{A}(j)}(x_i)$$

where  $\mathcal{A}(j) = (\mu_{j-1}, \mu_j]$  for `right = TRUE` except  $\mathcal{A}(l) = (\mu_{l-1}, \infty)$ . If `right = FALSE`, then  $\mathcal{A}(j) = [\mu_{j-1}, \mu_j)$  except  $\mathcal{A}(1) = (-\infty, \mu_1)$ . Note that for a categorical variable  $x_i$  and default split points,  $g$  is simply the identity.

Now,  $h$  maps from the index set  $\mathcal{I}$  into the set of daughter nodes:

$$f(x) = h(g(x)) = d_{\sigma_{g(x)}}$$

where  $\sigma = (\sigma_1, \dots, \sigma_l) \in \{1, \dots, k\}^l$  (`index`). By default,  $\sigma = (1, \dots, l)$  and  $k = l$ .

If  $x_i$  is missing, then  $f(x)$  is randomly drawn with  $\mathbb{P}(f(x) = d_j) = \pi_j, j = 1, \dots, k$  for a discrete probability distribution  $\pi = (\pi_1, \dots, \pi_k)$  over the  $k$  daughter nodes (`prob`).

In the simplest case of a binary split in a numeric variable  $x_i$ , there is only one split point  $\mu_1$  and, with  $\sigma = (1, 2)$ , observations with  $x_i \leq \mu_1$  are sent to daughter node  $d_1$  and observations with  $x_i > \mu_1$  to  $d_2$ . However, this representation of splits is general enough to deal with more complicated set-ups like surrogate splits, where typically the index needs modification, for example  $\sigma = (2, 1)$ , categorical splits, i.e., there is one data structure for both ordered and unordered splits, multiway splits, and functional splits. The latter can be implemented by defining a new artificial splitting variable  $x_{p+1}$  by means of a potentially very complex function of  $x$  later used for splitting.

### *Further examples*

Consider a split in a categorical variable at three levels where the first two levels go to the left daughter node and the third one to the right daughter node:

```
R> sp_o2 <- partysplit(1L, index = c(1L, 1L, 2L))
R> character_split(sp_o2, data = WeatherPlay)

$name
[1] "outlook"

$levels
[1] "sunny, overcast" "rainy"

R> table(kidids_split(sp_o2, data = WeatherPlay), WeatherPlay$outlook)
```

|   | sunny | overcast | rainy |
|---|-------|----------|-------|
| 1 | 5     | 4        | 0     |
| 2 | 0     | 0        | 5     |

The internal structure of this object contains the `index` slot that maps levels to kid nodes.

```
R> unclass(sp_o2)
```

```
$varid
[1] 1

$breaks
NULL

$index
[1] 1 1 2

$right
[1] TRUE

$prob
NULL

$info
NULL
```

This mapping is also useful with splits in ordered variables or when representing multiway splits:

```
R> sp_o <- partysplit(1L, index = 1L:3L)
R> character_split(sp_o, data = WeatherPlay)
```

```
$name
[1] "outlook"

$levels
[1] "sunny" "overcast" "rainy"
```

For a split in a numeric variable, the mapping to daughter nodes can also be changed by modifying `index`:

```
R> sp_t <- partysplit(2L, breaks = c(69.5, 78.8), index = c(1L, 2L, 1L))
R> character_split(sp_t, data = WeatherPlay)
```

```
$name
[1] "temperature"

$levels
[1] "(-Inf,69.5] | (78.8, Inf]" "(69.5,78.8]"
```

```
R> table(kidids_split(sp_t, data = WeatherPlay),
+       cut(WeatherPlay$temperature, breaks = c(-Inf, 69.5, 78.8, Inf)))

      (-Inf,69.5] (69.5,78.8] (78.8, Inf]
1          4          0          4
2          0          6          0
```

*Further comments*

The additional argument `prop` can be used to specify a discrete probability distribution over the daughter nodes that is used to map observations with missing values to daughter nodes. Furthermore, the `info` argument and slot can take arbitrary objects to be stored with the split (for example split statistics). Currently, no specific structure of the `info` is used.

Programmers that employ this functionality in their own functions/packages should access the elements of a ‘`partysplit`’ object by the corresponding accessor function (and not just the `$` operator as the internal structure might be changed/extended in future release).

**3.3. Nodes***Overview*

Inner and terminal nodes are represented by objects of class ‘`partynode`’. Each node has a unique identifier `id`. A node consisting only of such an identifier (and possibly additional information in `info`) is a terminal node:

```
R> n1 <- partynode(id = 1L)
R> is.terminal(n1)
```

```
[1] TRUE
```

```
R> print(n1)
```

```
[1] root *
```

Inner nodes have to have a primary split `split` and at least two daughter nodes. The daughter nodes are objects of class ‘`partynode`’ itself and thus represent the recursive nature of this data structure. The daughter nodes are pooled in a list `kids`.

In addition, a list of ‘`partysplit`’ objects offering surrogate splits can be supplied in argument `surrogates`. These are used in case the variable needed for the primary split has missing values in a particular data set.

The IDs in a ‘`partynode`’ should be numbered “depth first” (sometimes also called “infix” or “pre-order traversal”). This simply means that the root node has identifier 1; the first kid node has identifier 2, whose kid (if present) has identifier 3 and so on. If other IDs are desired, then one can simply set `names()` (see above) for the tree; however, internally the depth-first numbering needs to be used. Note that the `partynode()` constructor also allows to create

‘`partynode`’ objects with other ID schemes as this is necessary for growing the tree. If one wants to assure the a given ‘`partynode`’ object has the correct IDs, one can simply apply `as.partynode()` once more to assure the right order of IDs.

Finally, let us emphasize that ‘`partynode`’ objects are not directly connected to the actual data (only indirectly through the associated ‘`partysplit`’ objects).

### Examples

Based on the binary split `sp_h` defined in the previous section, we set up an inner node with two terminal daughter nodes and print this stump (the data is needed because neither split nor nodes contain information about variable names or levels):

```
R> n1 <- partynode(id = 1L, split = sp_o, kids = lapply(2L:4L, partynode))
R> print(n1, data = WeatherPlay)
```

```
[1] root
|  [2] outlook in sunny *
|  [3] outlook in overcast *
|  [4] outlook in rainy *
```

Now that we have defined this simple tree, we want to assign observations to terminal nodes:

```
R> fitted_node(n1, data = WeatherPlay)
```

```
[1] 2 2 3 4 4 4 3 2 2 4 2 3 3 4
```

Here, the `ids` of the terminal node each observations falls into are returned. Alternatively, we could compute the position of these daughter nodes in the list `kids`:

```
R> kidids_node(n1, data = WeatherPlay)
```

```
[1] 1 1 2 3 3 3 2 1 1 3 1 2 2 3
```

Furthermore, the `info` argument and slot takes arbitrary objects to be stored with the node (predictions, for example, but we will handle this issue later). The slots can be extracted by means of the corresponding accessor functions.

### Methods

A number of methods is defined for ‘`partynode`’ objects: `is.partynode()` checks if the argument is a valid ‘`partynode`’ object. `is.terminal()` is `TRUE` for terminal nodes and `FALSE` for inner nodes. The subset method `[` returns the ‘`partynode`’ object corresponding to the `i`-th kid.

The `as.partynode()` and `as.list()` methods can be used to convert flat list structures into recursive ‘`partynode`’ objects and vice versa. As pointed out above, `as.partynode()` applied to ‘`partynode`’ objects also renumbers the recursive nodes starting with root node identifier `from`.

Furthermore, many of the methods defined for the class ‘party’ illustrated above also work for plain ‘partynode’ objects. For example, `length()` gives the number of kid nodes of the root node, `depth()` the depth of the tree and `width()` the number of terminal nodes.

### 3.4. Trees

Although tree structures can be represented by ‘partynode’ objects, a tree is more than a number of nodes and splits. More information about (parts of the) corresponding data is necessary for high-level computations on trees.

#### *Trees and data*

First, the raw node/split structure needs to be associated with a corresponding data set.

```
R> t1 <- party(n1, data = WeatherPlay)
R> t1
```

```
[1] root
| [2] outlook in sunny: *
| [3] outlook in overcast: *
| [4] outlook in rainy: *
```

Note that the `data` may have zero rows (i.e., only contain variable names/classes but not the actual data) and all methods that do not require the presence of any learning data still work fine:

```
R> party(n1, data = WeatherPlay[0, ])
```

```
[1] root
| [2] outlook in sunny: *
| [3] outlook in overcast: *
| [4] outlook in rainy: *
```

#### *Response variables and regression relationships*

Second, for decision trees (or regression and classification trees) more information is required: namely, the response variable and its fitted values. Hence, a ‘`data.frame`’ can be supplied in `fitted` that has at least one variable (`fitted`) containing the terminal node numbers of data used for fitting the tree. For representing the dependence of the response on the partitioning variables, a `terms` object can be provided that is leveraged for appropriately preprocessing new data in predictions. Finally, any additional (currently unstructured) information can be stored in `info` again.

```
R> t2 <- party(n1,
+   data = WeatherPlay,
+   fitted = data.frame(
+     "(fitted)" = fitted_node(n1, data = WeatherPlay),
```

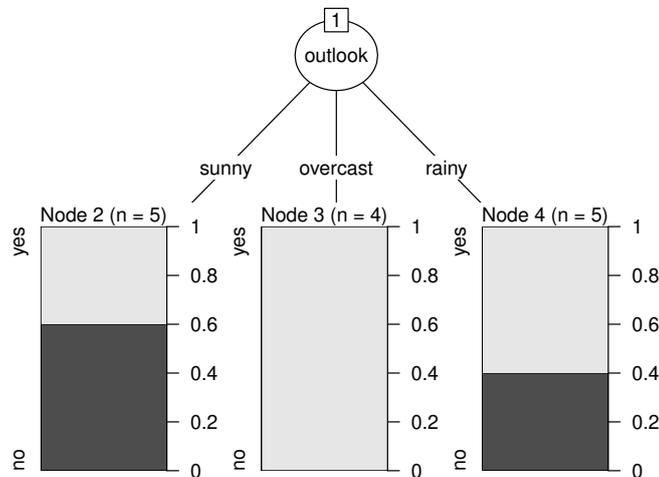

Figure 3: Constant-fit tree for play decision based on weather conditions in WeatherPlay data.

```
+      "(response)" = WeatherPlay$play,
+      check.names = FALSE),
+      terms = terms(play ~ ., data = WeatherPlay),
+    )
```

The information that is now contained in the tree `t2` is sufficient for all operations that should typically be performed on constant-fit trees. For this type of trees there is also a dedicated class `constparty` that provides some further convenience methods, especially for plotting and predicting. If a suitable `party` object like `t2` is already available, it just needs to be coerced:

```
R> t2 <- as.constparty(t2)
R> t2
```

Model formula:

```
play ~ outlook + temperature + humidity + windy
```

Fitted party:

```
[1] root
| [2] outlook in sunny: no (n = 5, err = 40%)
| [3] outlook in overcast: yes (n = 4, err = 0%)
| [4] outlook in rainy: yes (n = 5, err = 40%)
```

Number of inner nodes: 1

Number of terminal nodes: 3

As pointed out above, `constparty` objects have enhanced `plot()` and `predict()` methods. For example, `plot(t2)` now produces stacked bar plots in the leaves (see Figure 3) as `t2` is

a classification tree For regression and survival trees, boxplots and Kaplan-Meier curves are employed automatically, respectively.

As there is information about the response variable, the `predict()` method can now produce more than just the predicted node IDs. The default is to predict the "response", i.e., a factor for a classification tree. In this case, class probabilities ("prob") are also available in addition to the majority votings.

```
R> nd <- data.frame(outlook = factor(c("overcast", "sunny"),
+   levels = levels(WeatherPlay$outlook)))
R> predict(t2, newdata = nd, type = "response")
```

```
  1  2
yes no
Levels: yes no
```

```
R> predict(t2, newdata = nd, type = "prob")
```

```
  yes  no
1 1.0 0.0
2 0.4 0.6
```

```
R> predict(t2, newdata = nd, type = "node")
```

```
1 2
3 2
```

More details on how 'constparty' objects and their methods work can be found in the corresponding vignette("constparty", package = "partykit").

## 4. Summary

This vignette ("partykit") introduces the package **partykit** that provides a toolkit for computing with recursive partytions, especially decision/regression/classification trees. In this vignette, the basic 'party' class and associated infrastructure are discussed: splits, nodes, and trees with functions for printing, plotting, and predicting. Further vignettes in the package discuss in more detail the tools built on top of it.

## References

- Breiman L, Friedman JH, Olshen RA, Stone CJ (1984). *Classification and Regression Trees*. Wadsworth, California.
- De'ath G (2014). *mvpart: Multivariate Partitioning*. R package version 1.6-2, URL <http://CRAN.R-project.org/package=mvpart>.

- Hornik K, Buchta C, Zeileis A (2009). “Open-Source Machine Learning: R Meets **Weka**.” *Computational Statistics*, **24**(2), 225–232.
- Hothorn T (2014). “CRAN Task View: Machine Learning & Statistical Learning.” Version 2014-08-30, URL <https://CRAN.R-project.org/view=MachineLearning>.
- Hothorn T, Hornik K, Strobl C, Zeileis A (2015). *party: A Laboratory for Recursive Partitioning*. R package version 1.0-23, URL <http://CRAN.R-project.org/package=party>.
- Hothorn T, Hornik K, Zeileis A (2006). “Unbiased Recursive Partitioning: A Conditional Inference Framework.” *Journal of Computational and Graphical Statistics*, **15**(3), 651–674. doi:10.1198/106186006X133933.
- Loh WY (2002). “Regression Trees with Unbiased Variable Selection and Interaction Detection.” *Statistica Sinica*, **12**, 361–386.
- Loh WY (2014). “Fifty Years of Classification and Regression Trees.” *International Statistical Review*, **82**(3), 329–348. doi:10.1111/insr.12016.
- Loh WY, Shih YS (1997). “Split Selection Methods for Classification Trees.” *Statistica Sinica*, **7**, 815–840.
- Morgan JN, Sonquist JA (1963). “Problems in the Analysis of Survey Data, and a Proposal.” *Journal of the American Statistical Association*, **58**, 415–434.
- Quinlan JR (1993). *C4.5: Programs for Machine Learning*. Morgan Kaufmann Publishers, San Mateo.
- R Core Team (2013). *R: A Language and Environment for Statistical Computing*. R Foundation for Statistical Computing, Vienna, Austria. URL <http://www.R-project.org/>.
- Therneau TM, Atkinson EJ (1997). “An Introduction to Recursive Partitioning Using the **rpart** Routine.” *Technical Report 61*, Section of Biostatistics, Mayo Clinic, Rochester. URL <http://www.mayo.edu/hsr/techrpt/61.pdf>.
- Witten IH, Frank E (2005). *Data Mining: Practical Machine Learning Tools and Techniques*. 2nd edition. Morgan Kaufmann, San Francisco.
- Zeileis A, Hothorn T, Hornik K (2008). “Model-Based Recursive Partitioning.” *Journal of Computational and Graphical Statistics*, **17**(2), 492–514. doi:10.1198/106186008X319331.

**Affiliation:**

Achim Zeileis  
Department of Statistics  
Faculty of Economics and Statistics  
Universität Innsbruck  
Universitätsstr. 15  
6020 Innsbruck, Austria  
E-mail: [Achim.Zeileis@R-project.org](mailto:Achim.Zeileis@R-project.org)  
URL: <http://eeecon.uibk.ac.at/~zeileis/>

Torsten Hothorn  
Institut für Epidemiologie, Biostatistik und Prävention  
Universität Zürich  
Hirschengraben 84  
CH-8001 Zürich, Switzerland  
E-mail: [Torsten.Hothorn@R-project.org](mailto:Torsten.Hothorn@R-project.org)  
URL: <http://user.math.uzh.ch/hothorn/>
